# Supplementary material for: Analysis note: two-particle correlation in $e^+e^-$ collisions at 91-209 GeV with archived ALEPH data
Source: arXiv:2309.09874 source file (2024-01-27)
Supplement: Supplementary file 1 [file appendix.tex]

\appendix

\section{Two-particle correlations within a specific $p_T$ interval}
\label{app:2PC_ptbinned}
%%%%%%%%%%%%%%% Beam 
%%%%%%%%%%%%%%%%%%%%%%%%%%% 2D 
\begin{figure}[ht]
\centering
\makebox[\textwidth][c]{
    \includegraphics[width=1.2\textwidth]{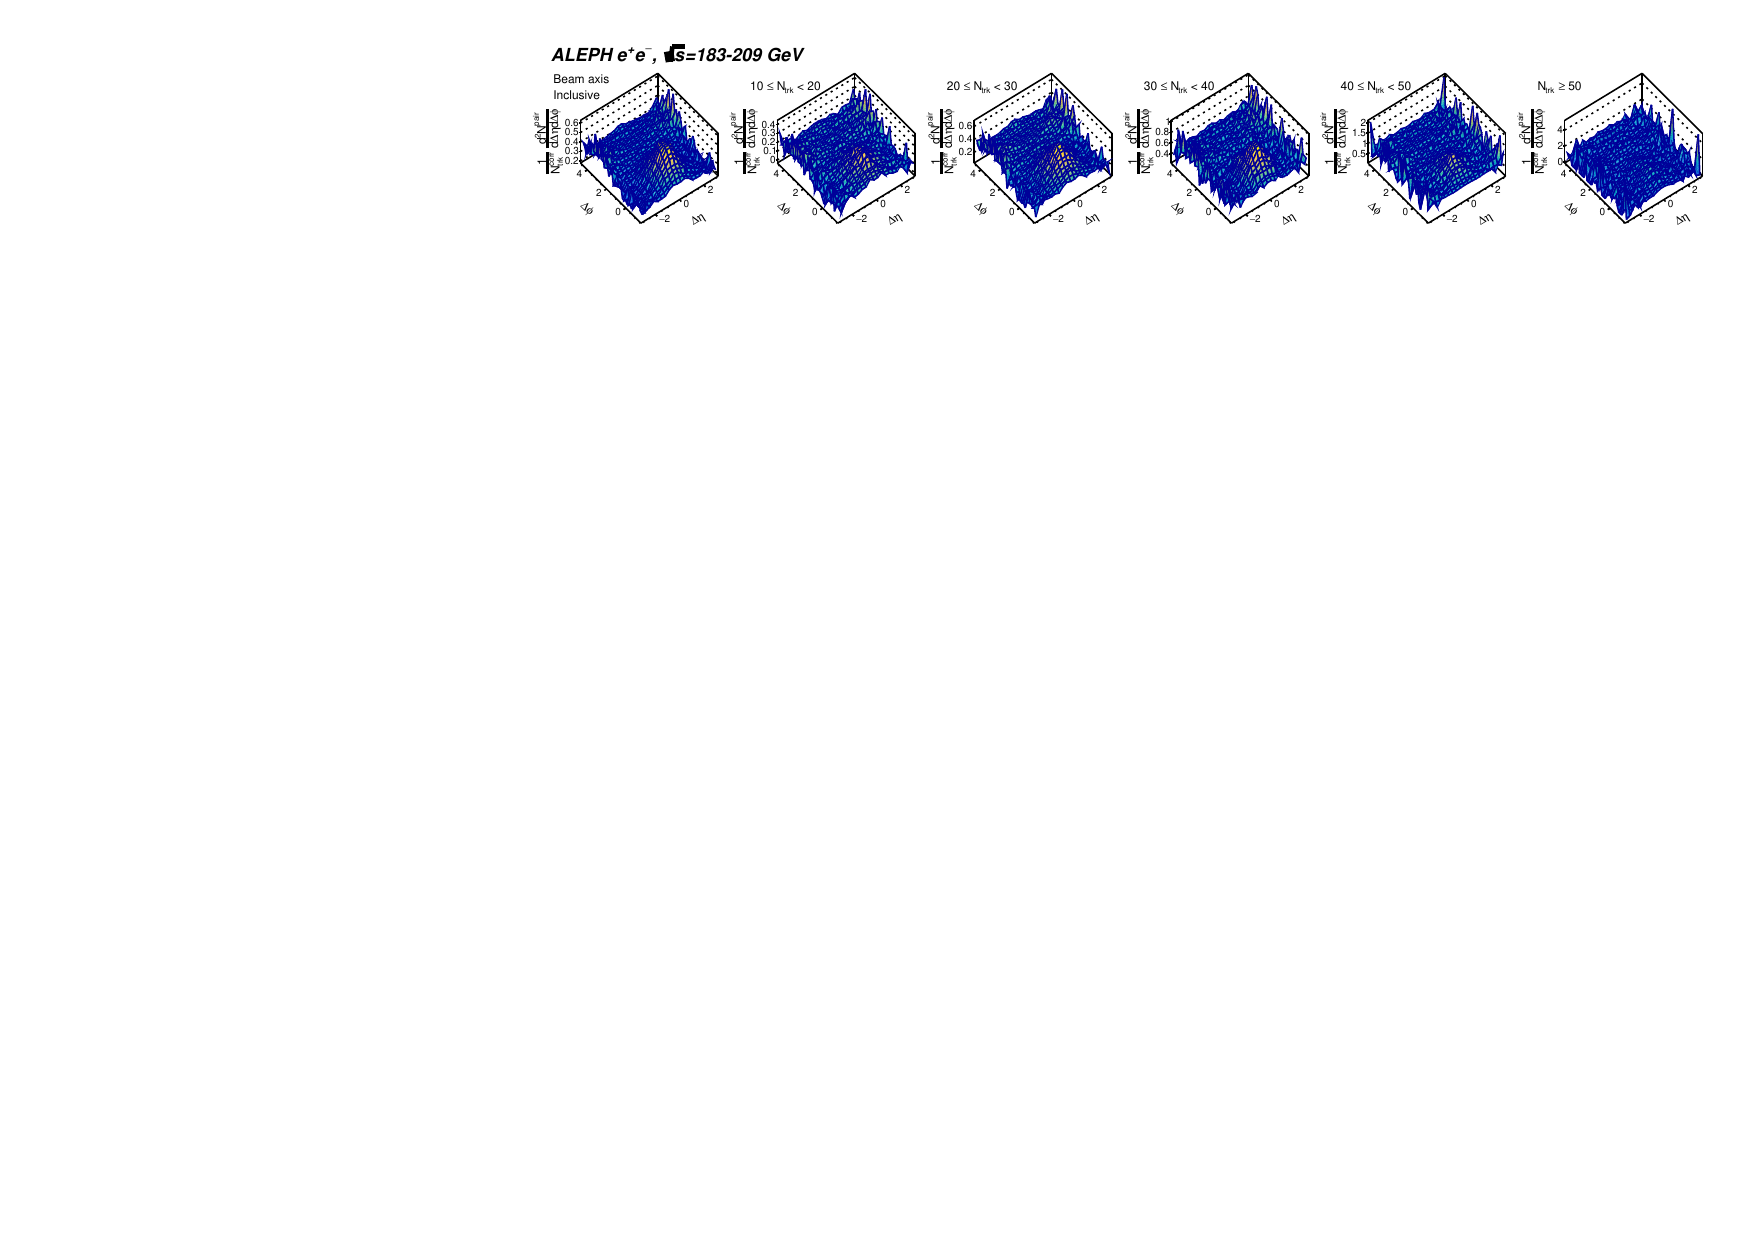}
}
\caption{Two-particle correlation function for $0 < p_T < 0.5$~GeV with the high-energy sample in the beam axis analysis. Results are shown multiplicity-inclusively and as a function of the offline multiplicity in $[10,20), [20,30), [30,40), [40,50), [50, \infty)$ intervals.}
\label{fig:EnergyCut_ge_100_TransPtCut_0.0_0.5_beam}
\end{figure}

\begin{figure}[ht]
\centering
\makebox[\textwidth][c]{
    \includegraphics[width=1.2\textwidth]{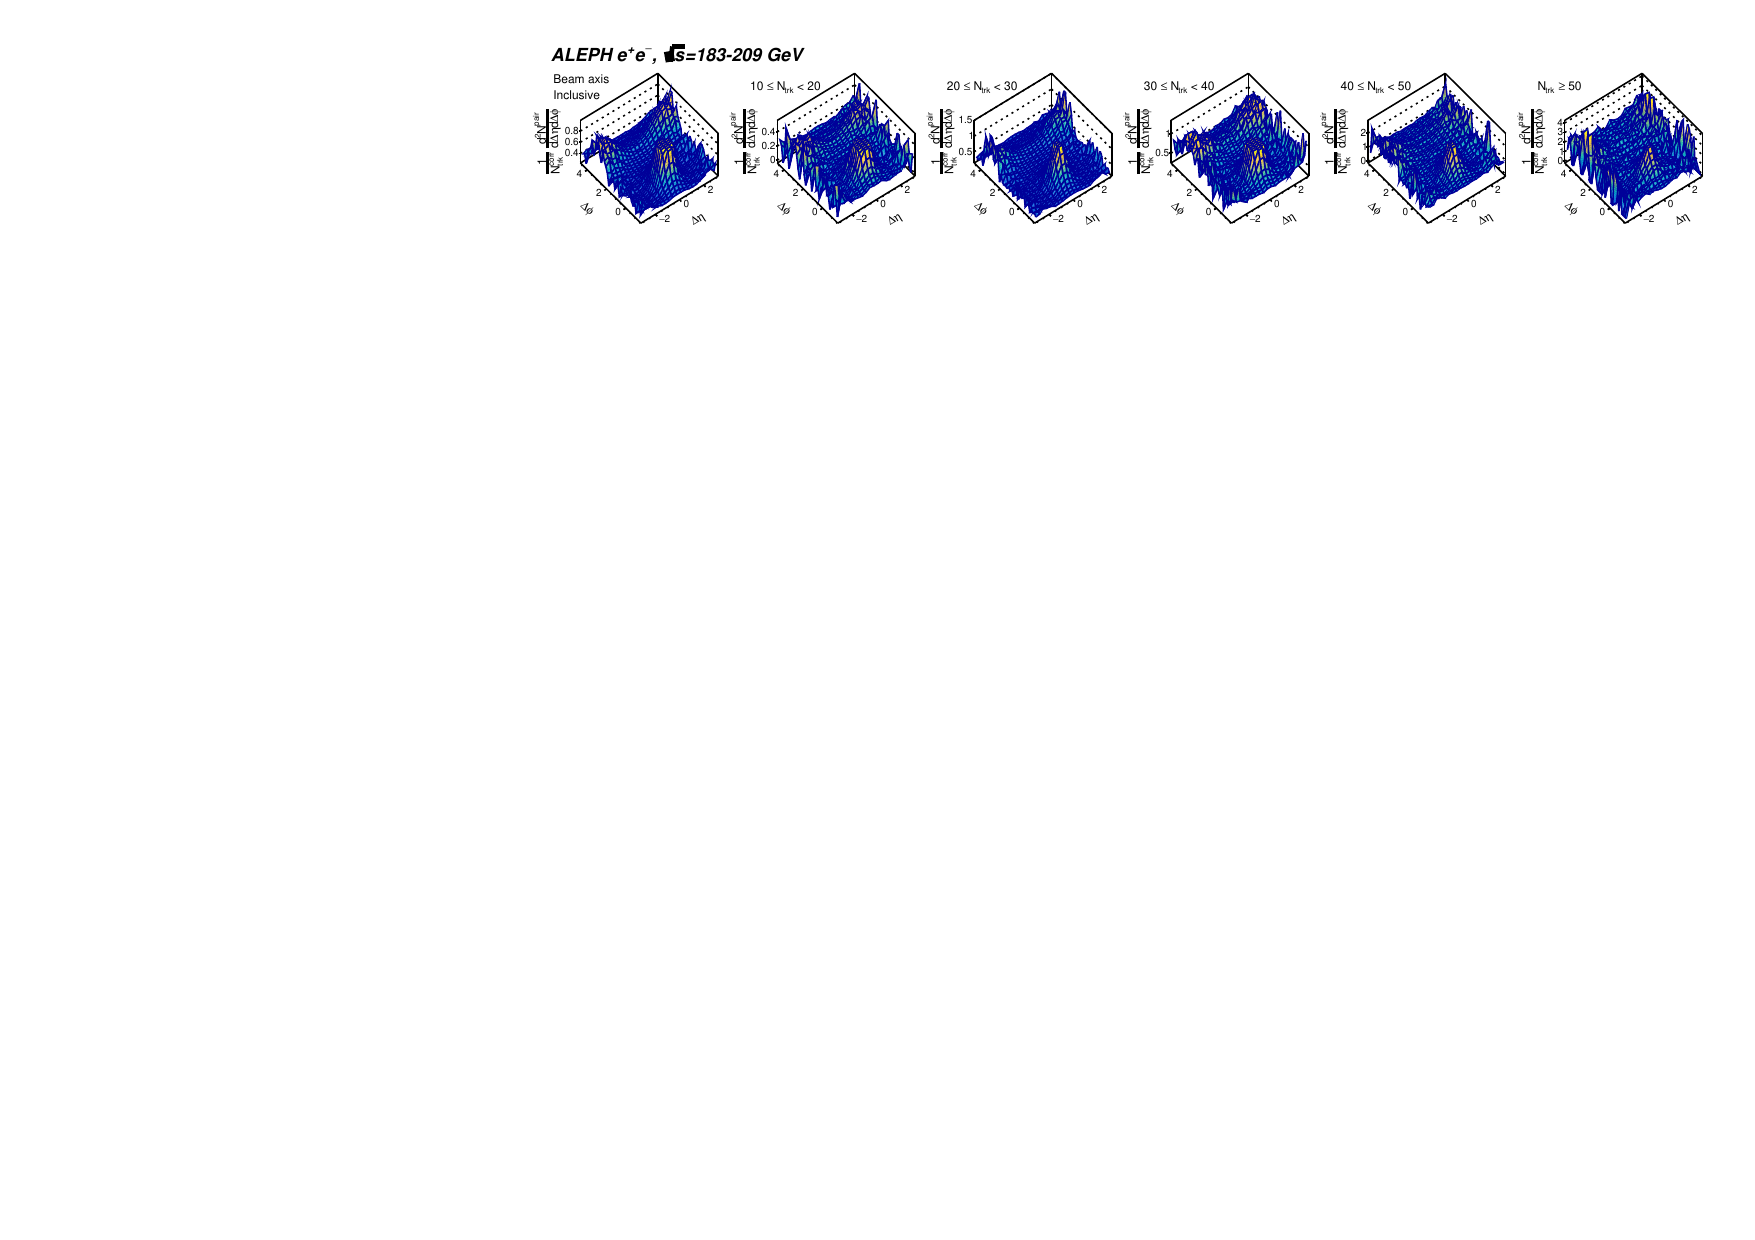}
}
\caption{Two-particle correlation function for $0.5 < p_T < 1$~GeV with the high-energy sample in the beam axis analysis. Results are shown multiplicity-inclusively and as a function of the offline multiplicity in $[10,20), [20,30), [30,40), [40,50), [50, \infty)$ intervals.}
\label{fig:EnergyCut_ge_100_TransPtCut_0.5_1.0_beam}
\end{figure}

\begin{figure}[ht]
\centering
\makebox[\textwidth][c]{
    \includegraphics[width=1.2\textwidth]{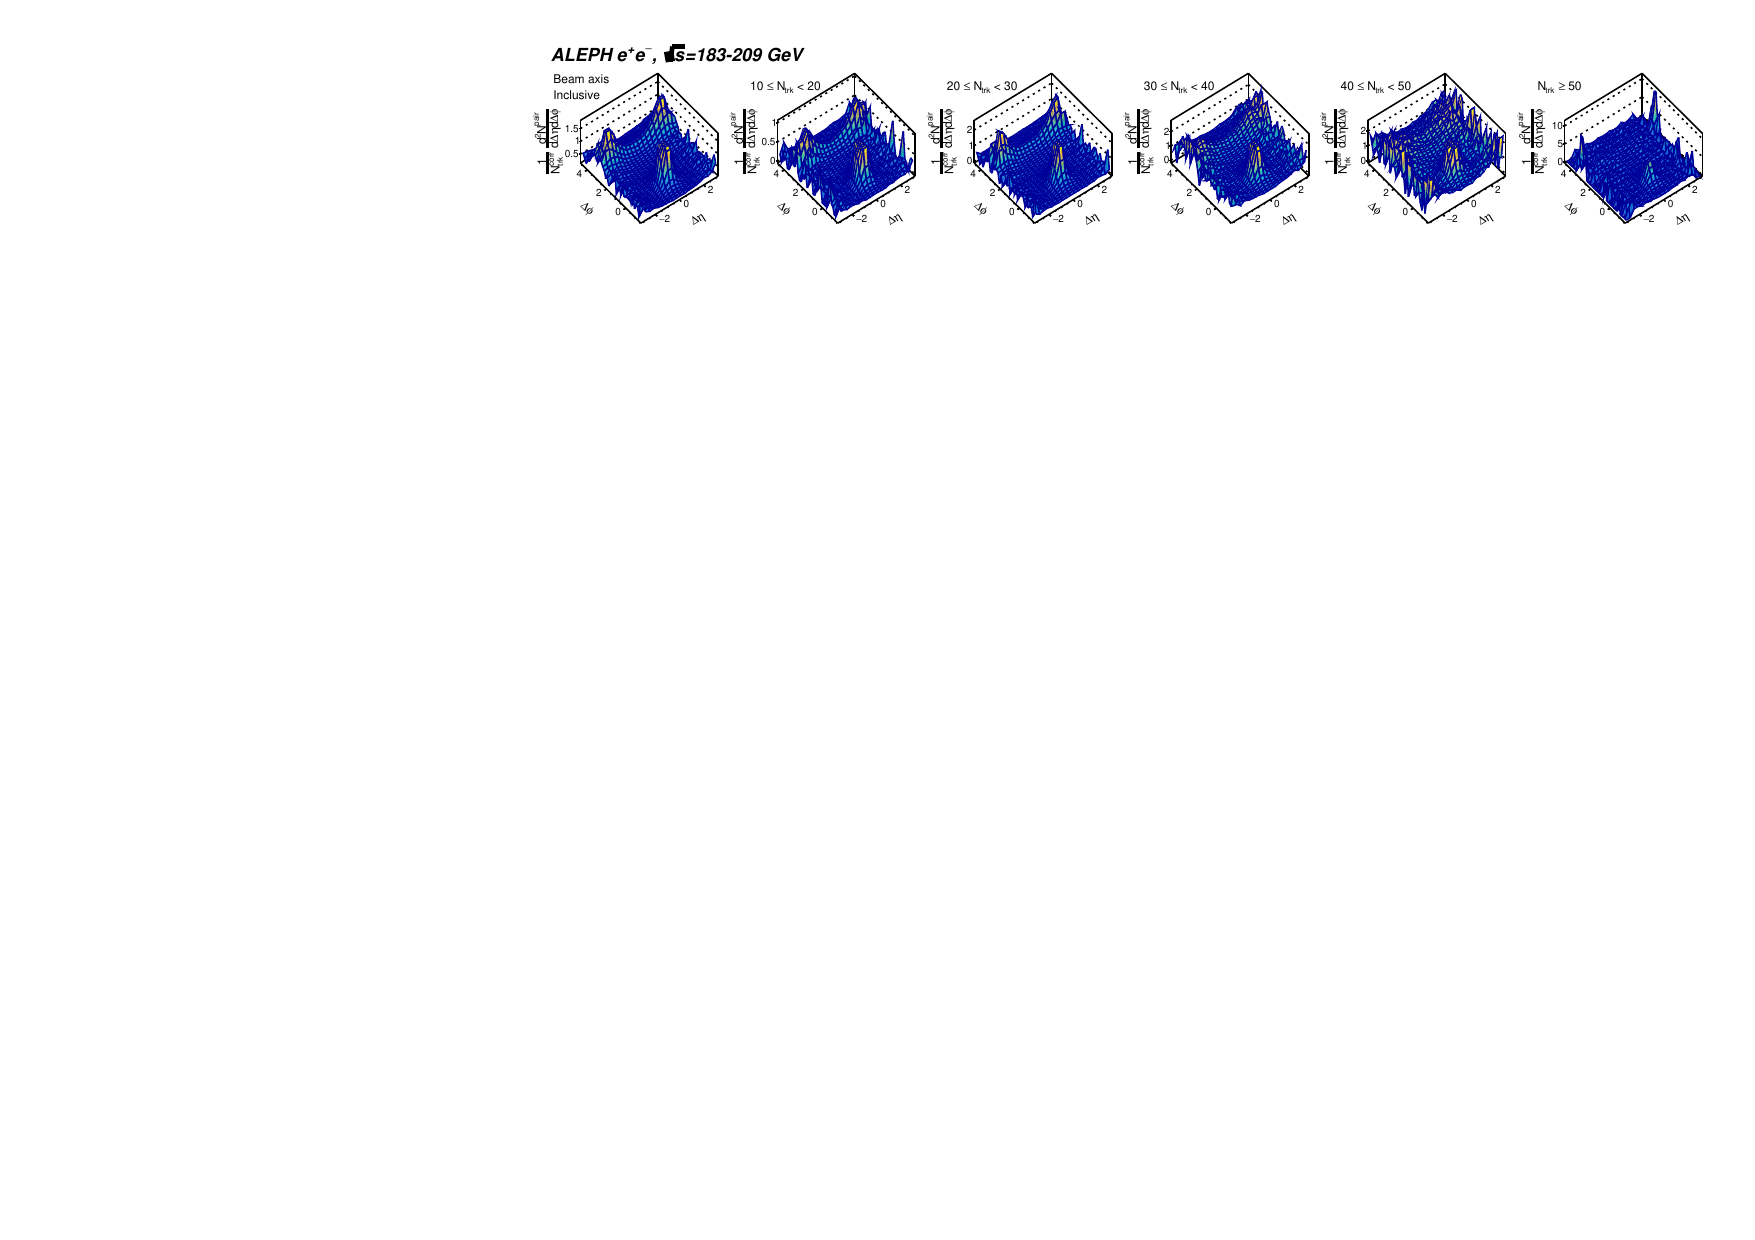}
}
\caption{Two-particle correlation function for $1 < p_T < 2$~GeV with the high-energy sample in the beam axis analysis. Results are shown multiplicity-inclusively and as a function of the offline multiplicity in $[10,20), [20,30), [30,40), [40,50), [50, \infty)$ intervals.}
\label{fig:EnergyCut_ge_100_TransPtCut_1.0_2.0_beam}
\end{figure}

\begin{figure}[ht]
\centering
\makebox[\textwidth][c]{
    \includegraphics[width=1.2\textwidth]{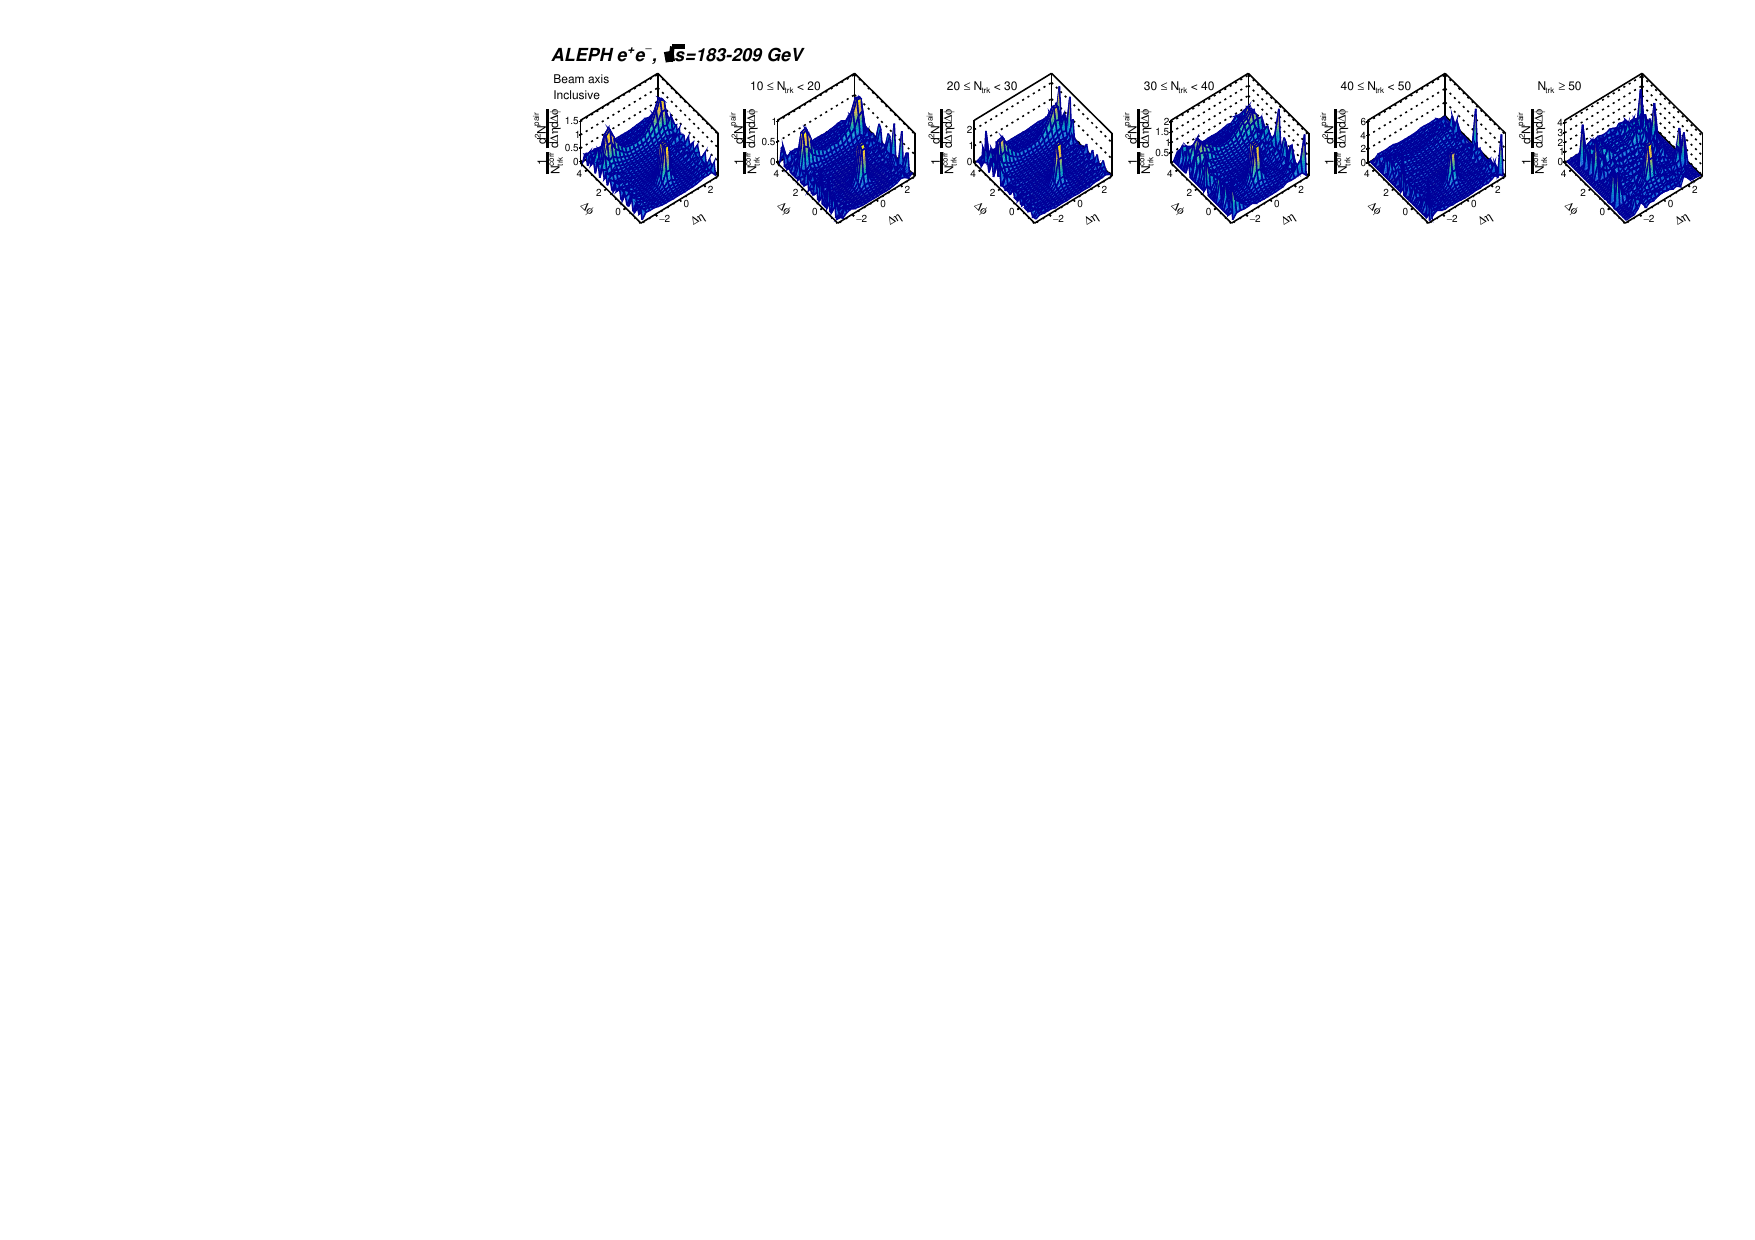}
}
\caption{Two-particle correlation function for $2 < p_T < 3$~GeV with the high-energy sample in the beam axis analysis. Results are shown multiplicity-inclusively and as a function of the offline multiplicity in $[10,20), [20,30), [30,40), [40,50), [50, \infty)$ intervals.}
\label{fig:EnergyCut_ge_100_TransPtCut_2.0_3.0_beam}
\end{figure}

\begin{figure}[ht]
\centering
\makebox[\textwidth][c]{
    \includegraphics[width=1.2\textwidth]{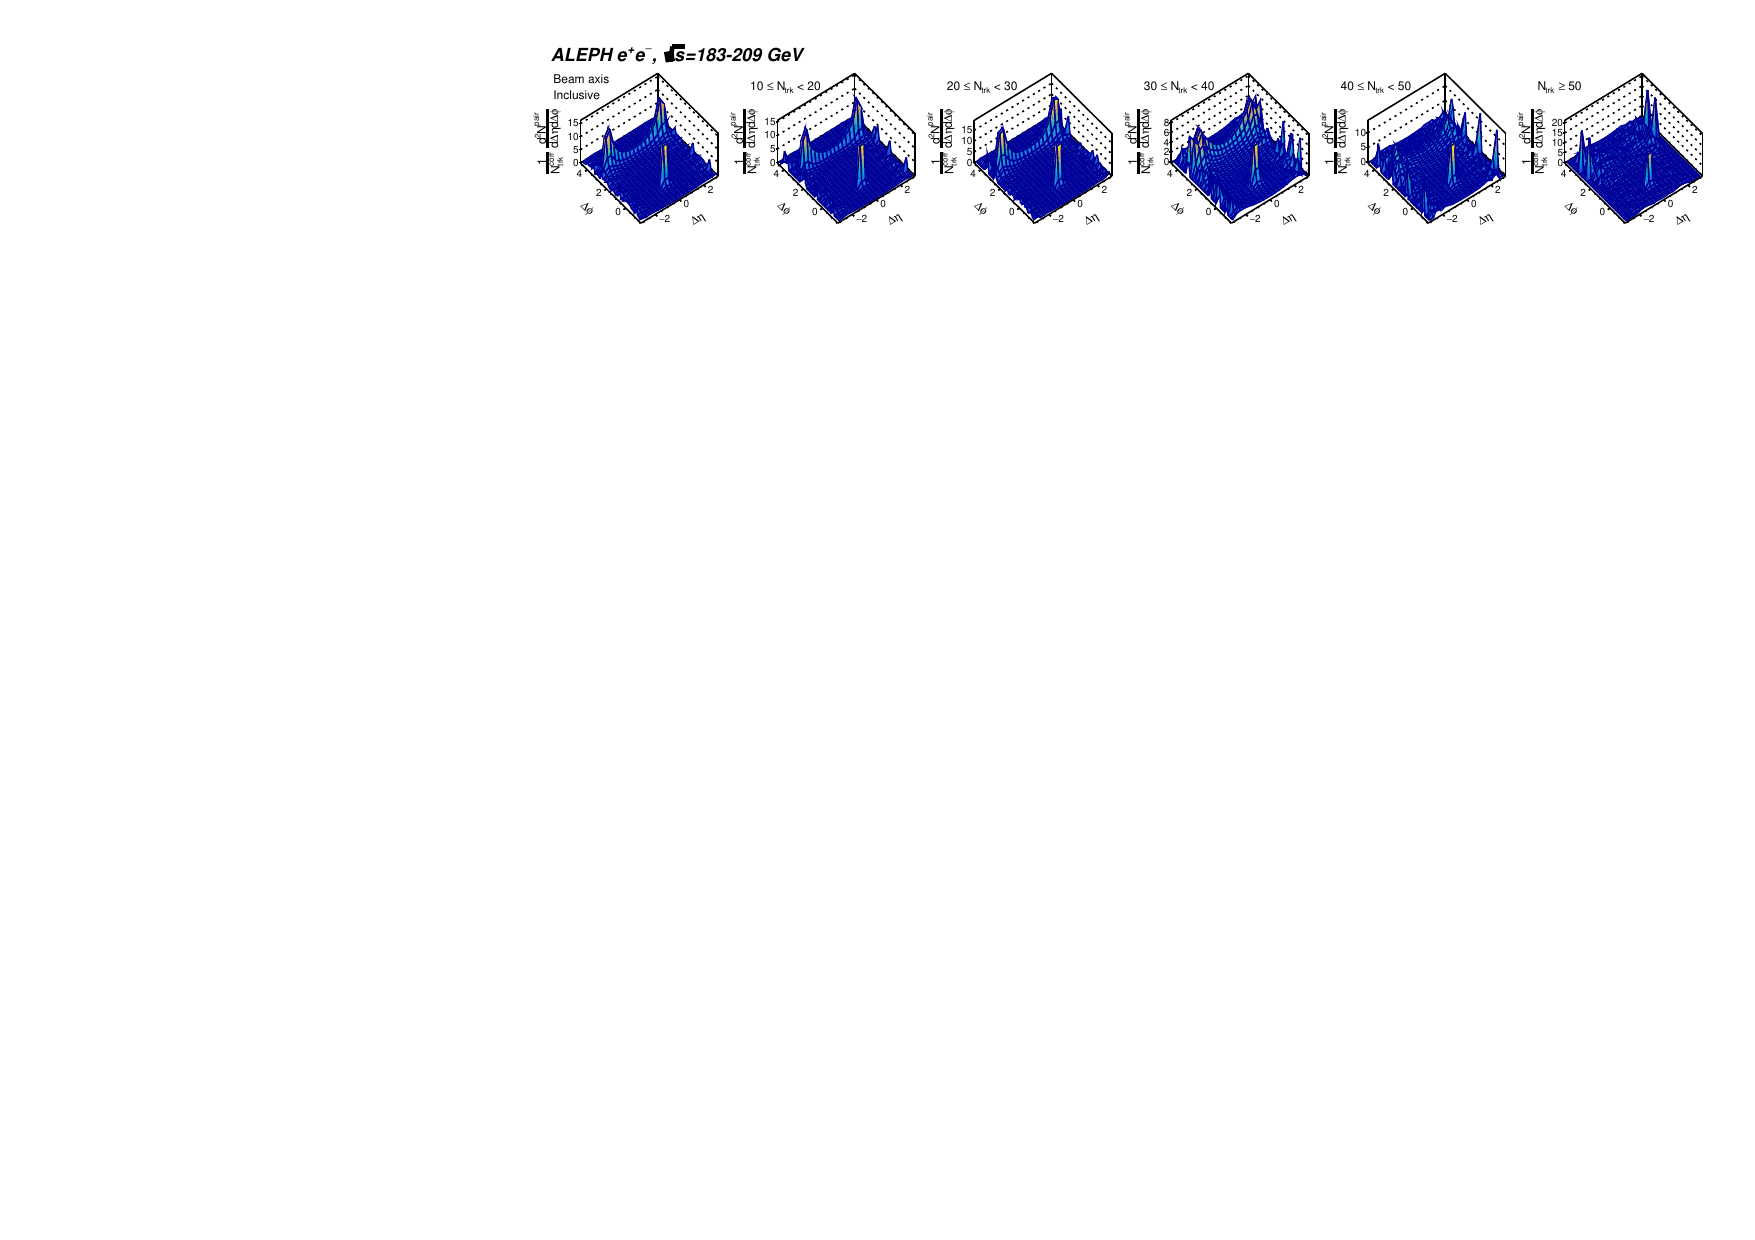}
}
\caption{Two-particle correlation function for $p_T > 3$~GeV with the high-energy sample in the beam axis analysis. Results are shown multiplicity-inclusively and as a function of the offline multiplicity in $[10,20), [20,30), [30,40), [40,50), [50, \infty)$ intervals.}
\label{fig:EnergyCut_ge_100_TransPtCut_3.0_beam}
\end{figure}
\clearpage

%%%%%%%%%%%%%%%%%%%%%%%%%%% 1D 
\begin{figure}[ht]
\centering
\makebox[\textwidth][c]{
    \includegraphics[width=1.2\textwidth]{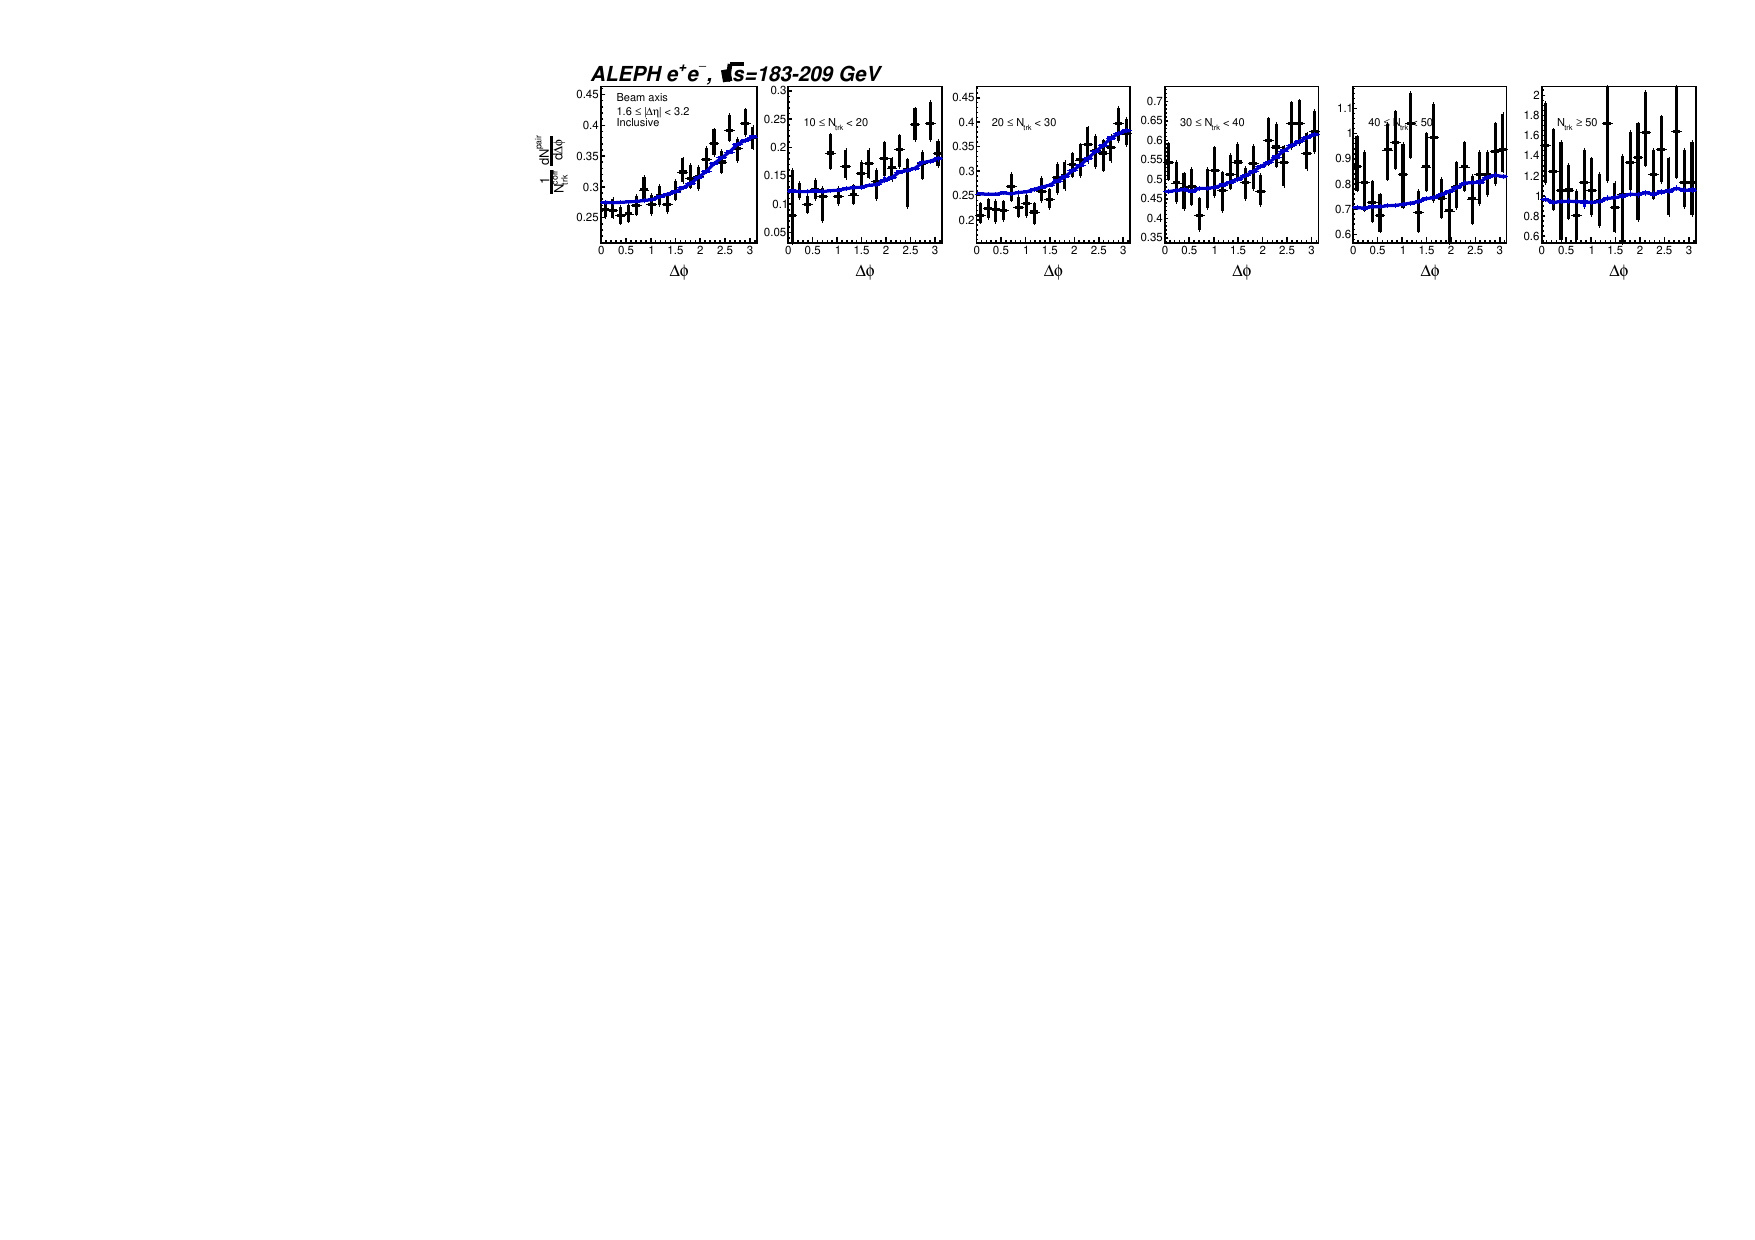}
}
\caption{Long-range azimuthal differential yields for $0 < p_T < 0.5$~GeV with the high-energy sample in the beam axis analysis. Results are shown multiplicity-inclusively and as a function of the offline multiplicity in $[10,20), [20,30), [30,40), [40,50), [50, \infty)$ intervals.}
\label{fig:EnergyCut_ge_100_TransPtCut_0.0_0.5_beam_1d}
\end{figure}

\begin{figure}[ht]
\centering
\makebox[\textwidth][c]{
    \includegraphics[width=1.2\textwidth]{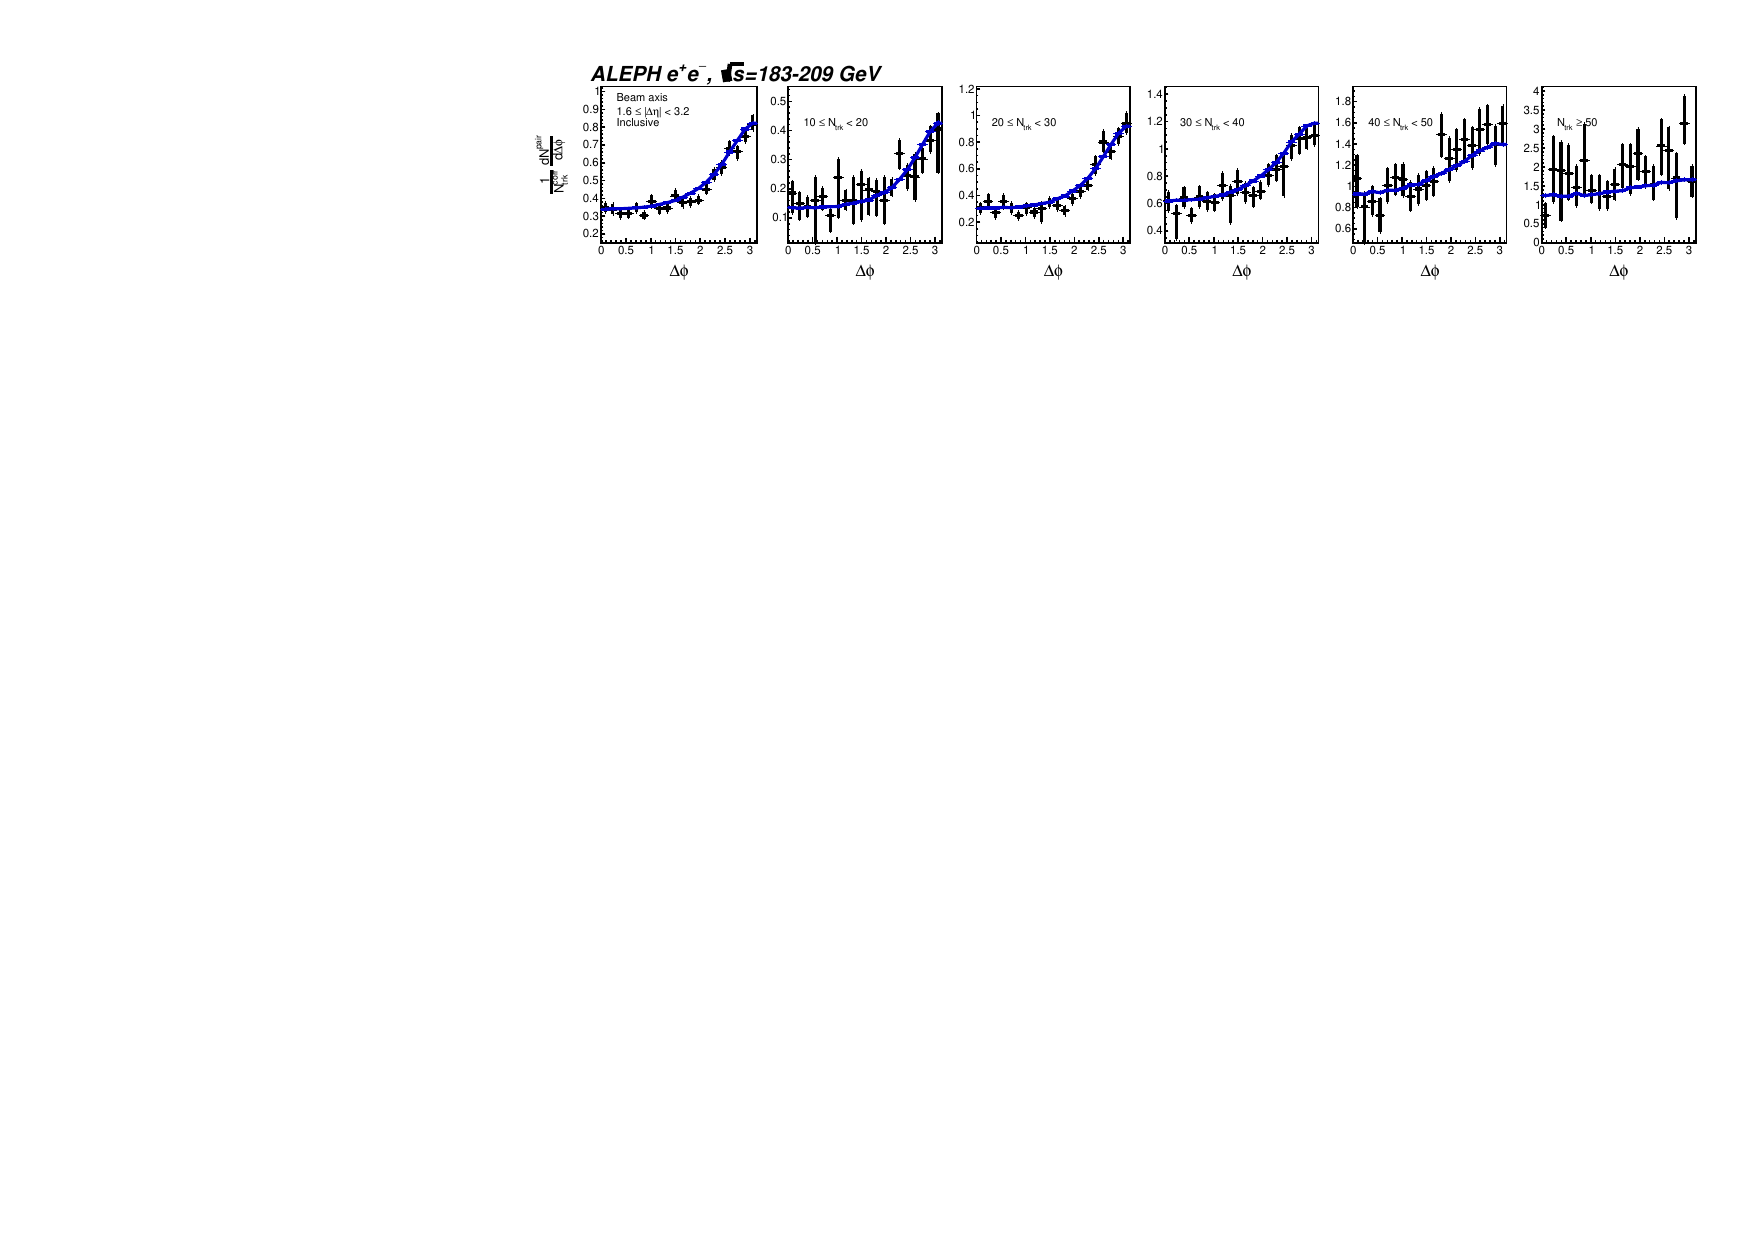}
}
\caption{Long-range azimuthal differential yields for $0.5 < p_T < 1$~GeV with the high-energy sample in the beam axis analysis. Results are shown multiplicity-inclusively and as a function of the offline multiplicity in $[10,20), [20,30), [30,40), [40,50), [50, \infty)$ intervals.}
\label{fig:EnergyCut_ge_100_TransPtCut_0.5_1.0_beam_1d}
\end{figure}

\begin{figure}[ht]
\centering
\makebox[\textwidth][c]{
    \includegraphics[width=1.2\textwidth]{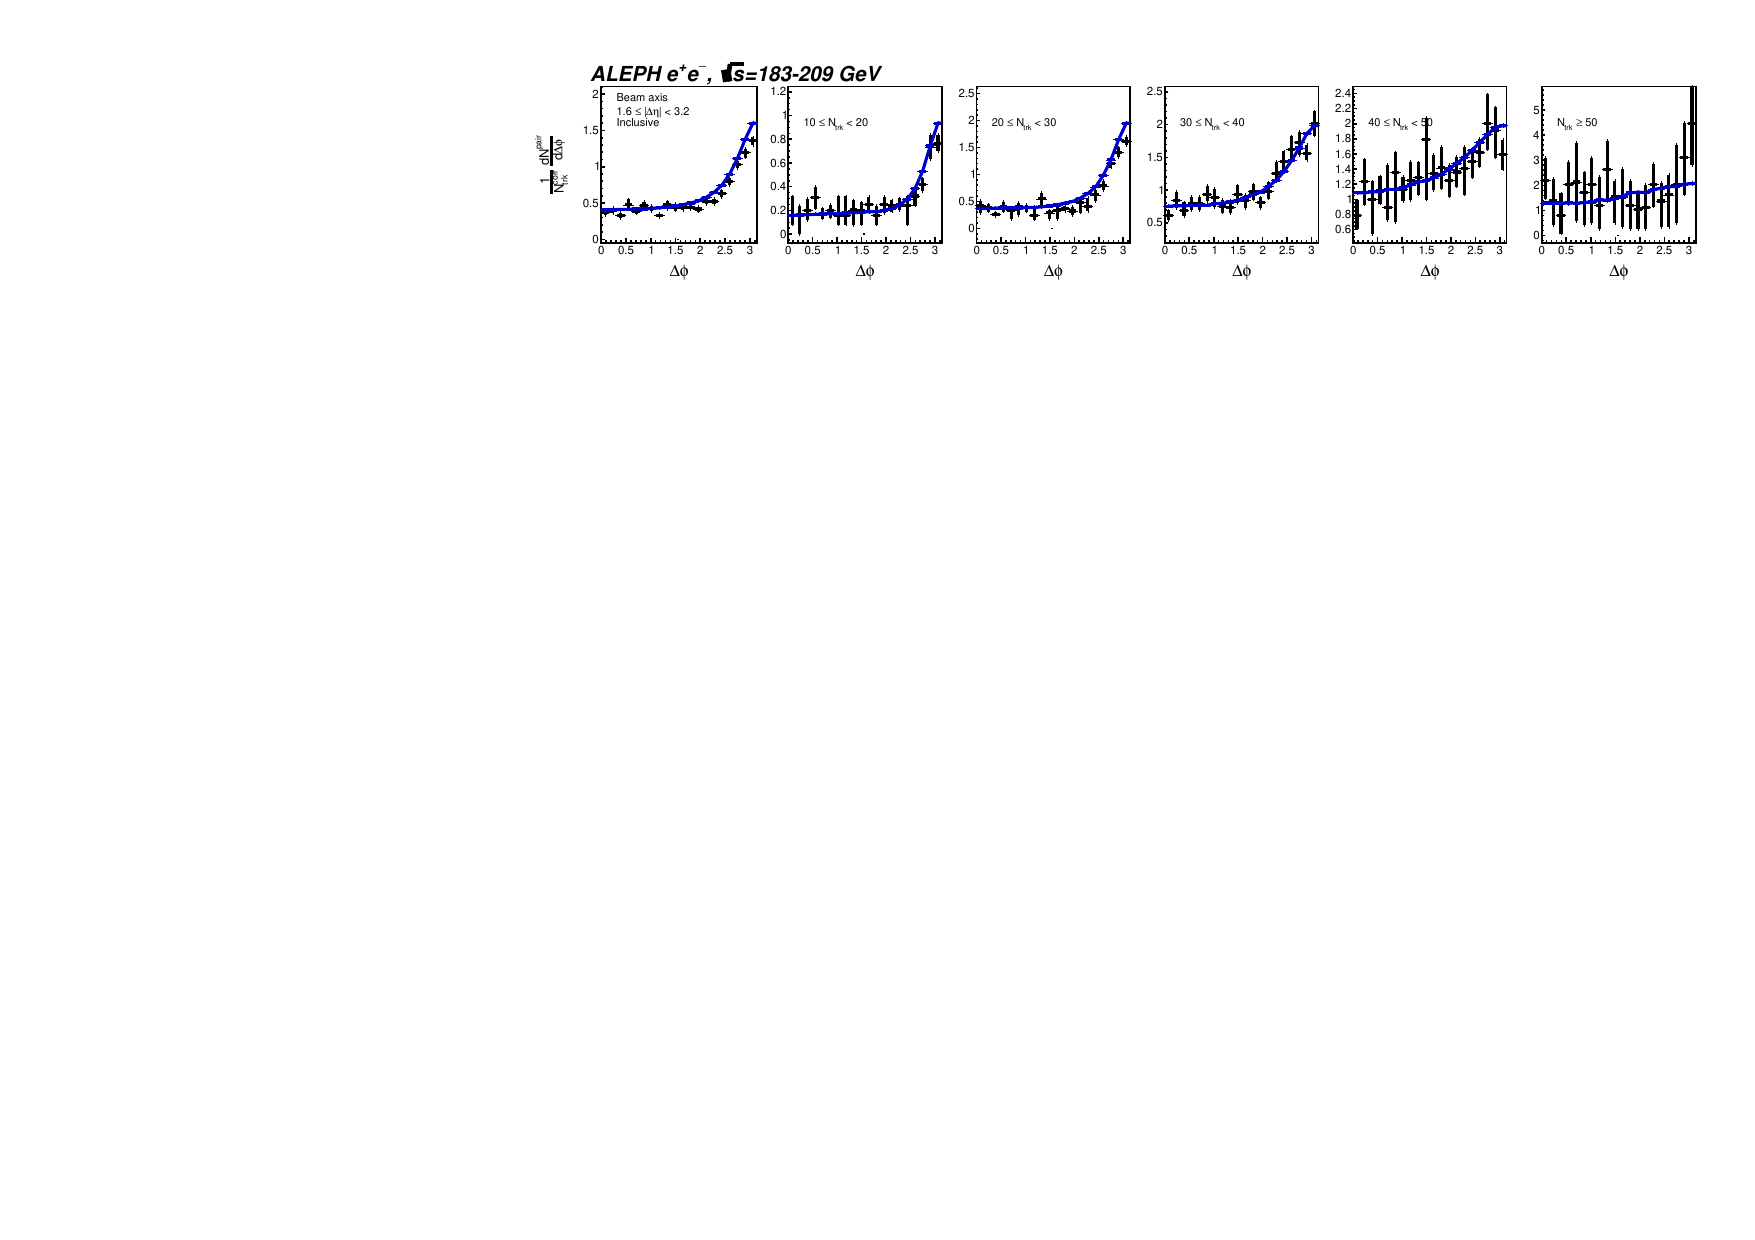}
}
\caption{Long-range azimuthal differential yields for $1 < p_T < 2$~GeV with the high-energy sample in the beam axis analysis. Results are shown multiplicity-inclusively and as a function of the offline multiplicity in $[10,20), [20,30), [30,40), [40,50), [50, \infty)$ intervals.}
\label{fig:EnergyCut_ge_100_TransPtCut_1.0_2.0_beam_1d}
\end{figure}

\begin{figure}[ht]
\centering
\makebox[\textwidth][c]{
    \includegraphics[width=1.2\textwidth]{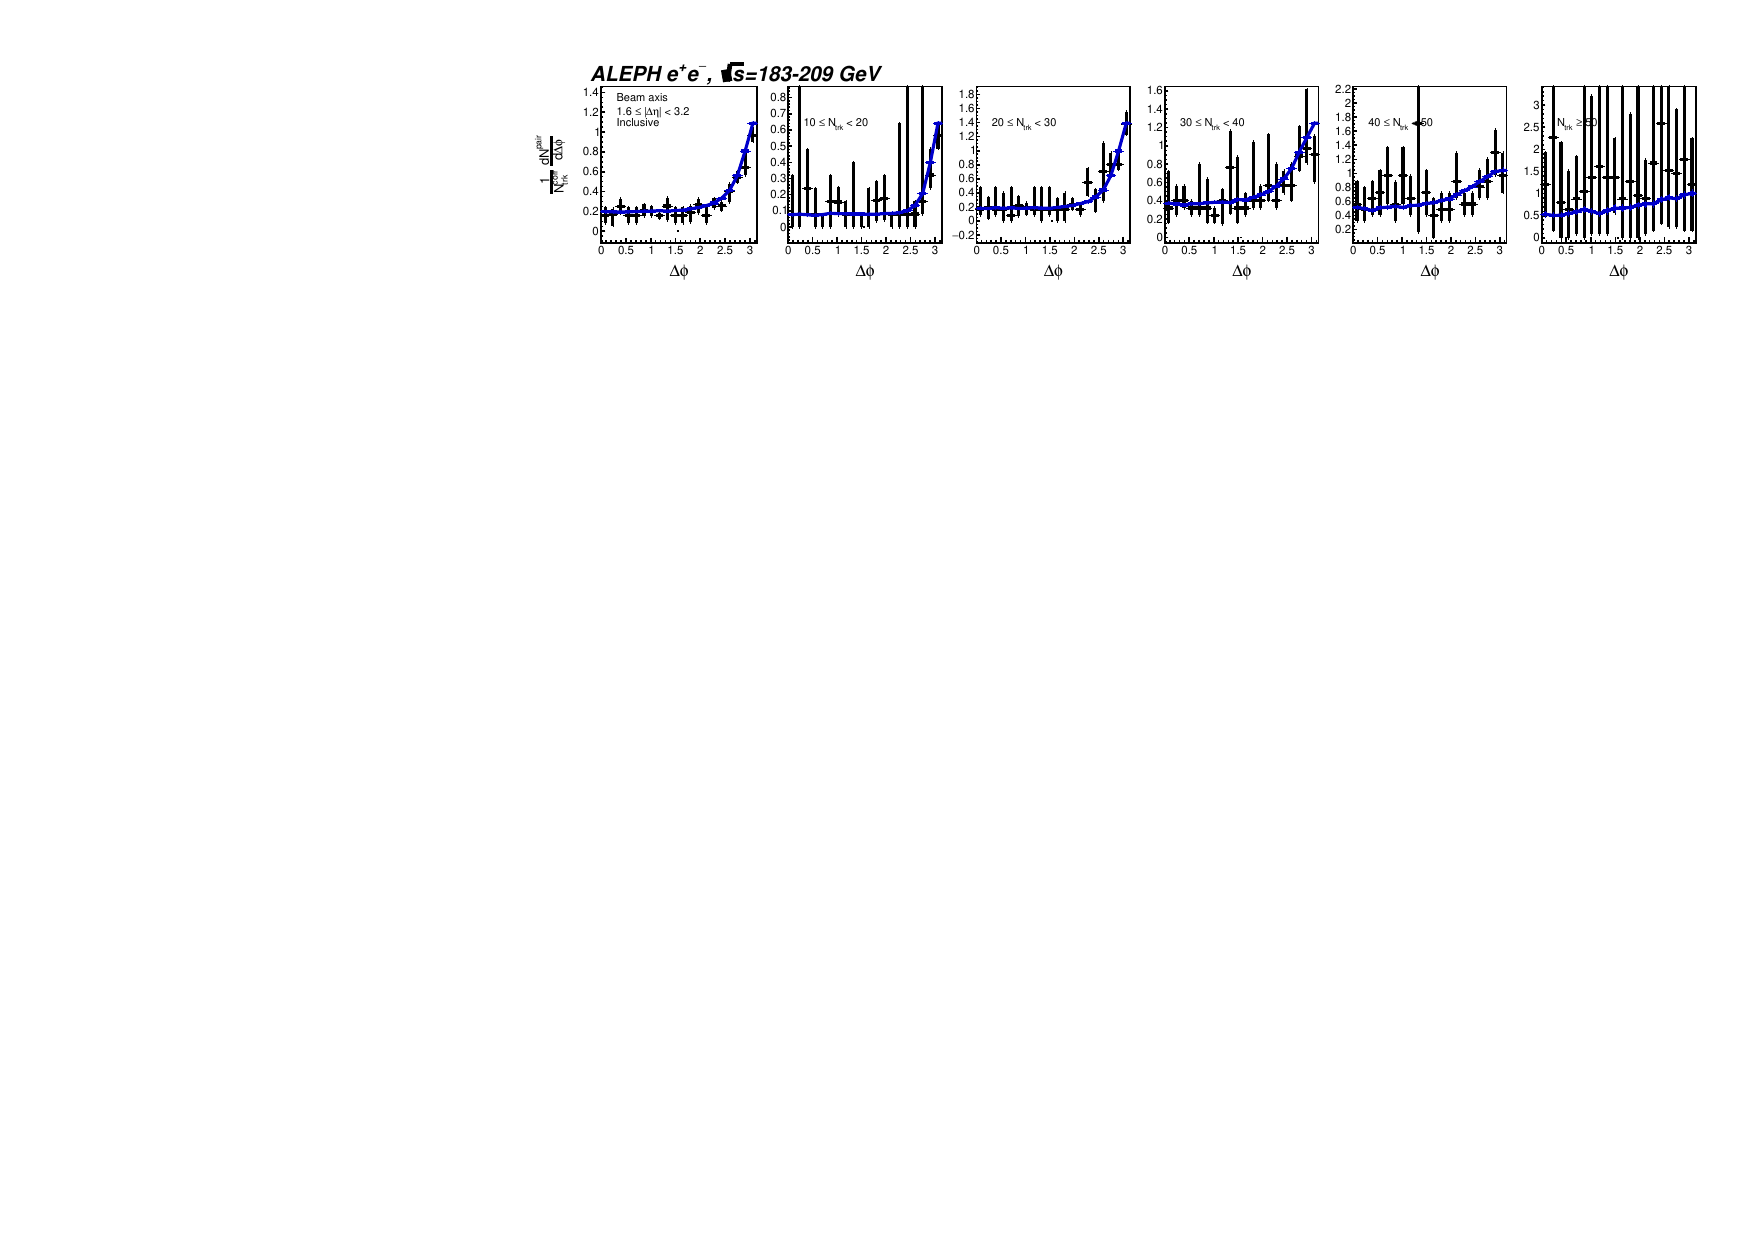}
}
\caption{Long-range azimuthal differential yields for $2 < p_T < 3$~GeV with the high-energy sample in the beam axis analysis. Results are shown multiplicity-inclusively and as a function of the offline multiplicity in $[10,20), [20,30), [30,40), [40,50), [50, \infty)$ intervals.}
\label{fig:EnergyCut_ge_100_TransPtCut_2.0_3.0_beam_1d}
\end{figure}

\begin{figure}[ht]
\centering
\makebox[\textwidth][c]{
    \includegraphics[width=1.2\textwidth]{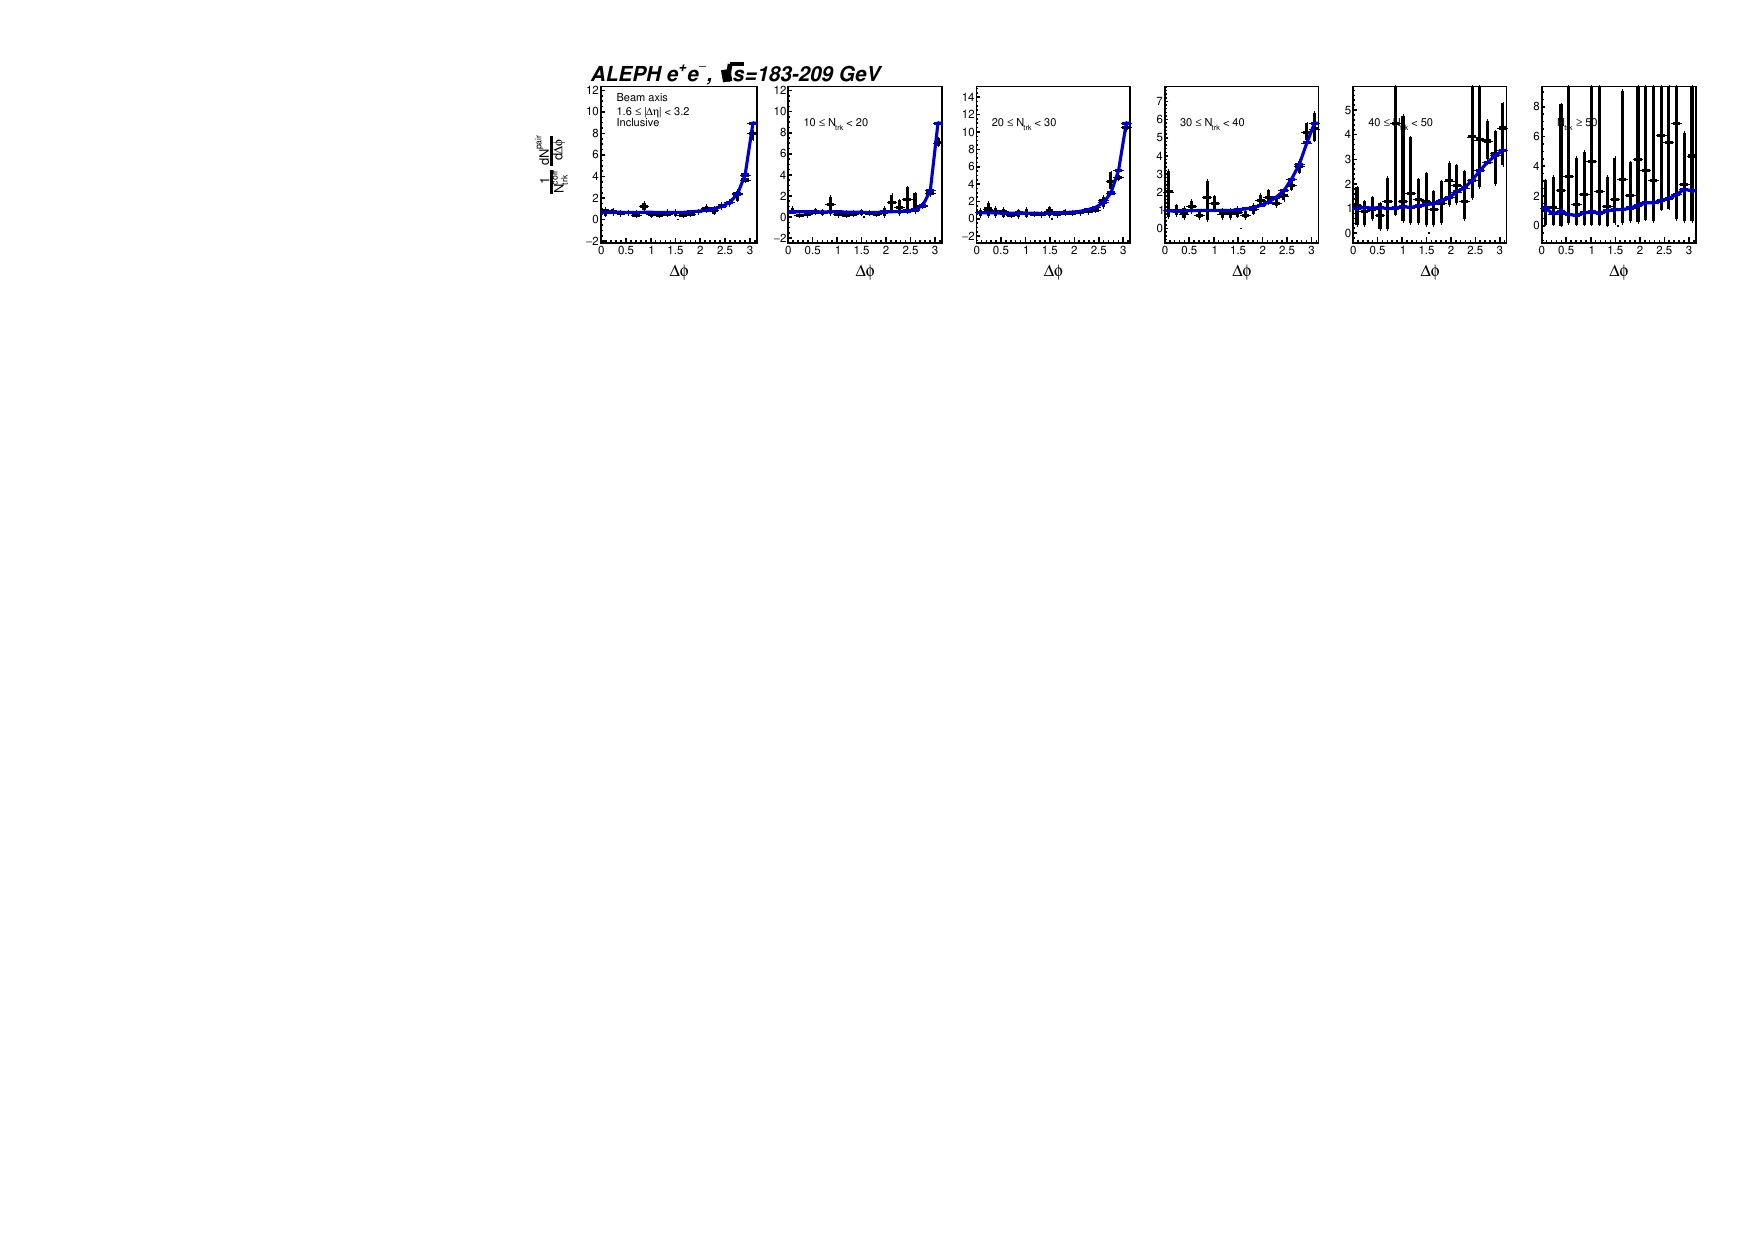}
}
\caption{Long-range azimuthal differential yields for $p_T > 3$~GeV with the high-energy sample in the beam axis analysis. Results are shown multiplicity-inclusively and as a function of the offline multiplicity in $[10,20), [20,30), [30,40), [40,50), [50, \infty)$ intervals.}
\label{fig:EnergyCut_ge_100_TransPtCut_3.0_beam_1d}
\end{figure}
\clearpage

%%%%%%%%%%%%%%% Thrust
%%%%%%%%%%%%%%%%%%%%%%%%%%% 2D 
\begin{figure}[ht]
\centering
\makebox[\textwidth][c]{
    \includegraphics[width=1.2\textwidth]{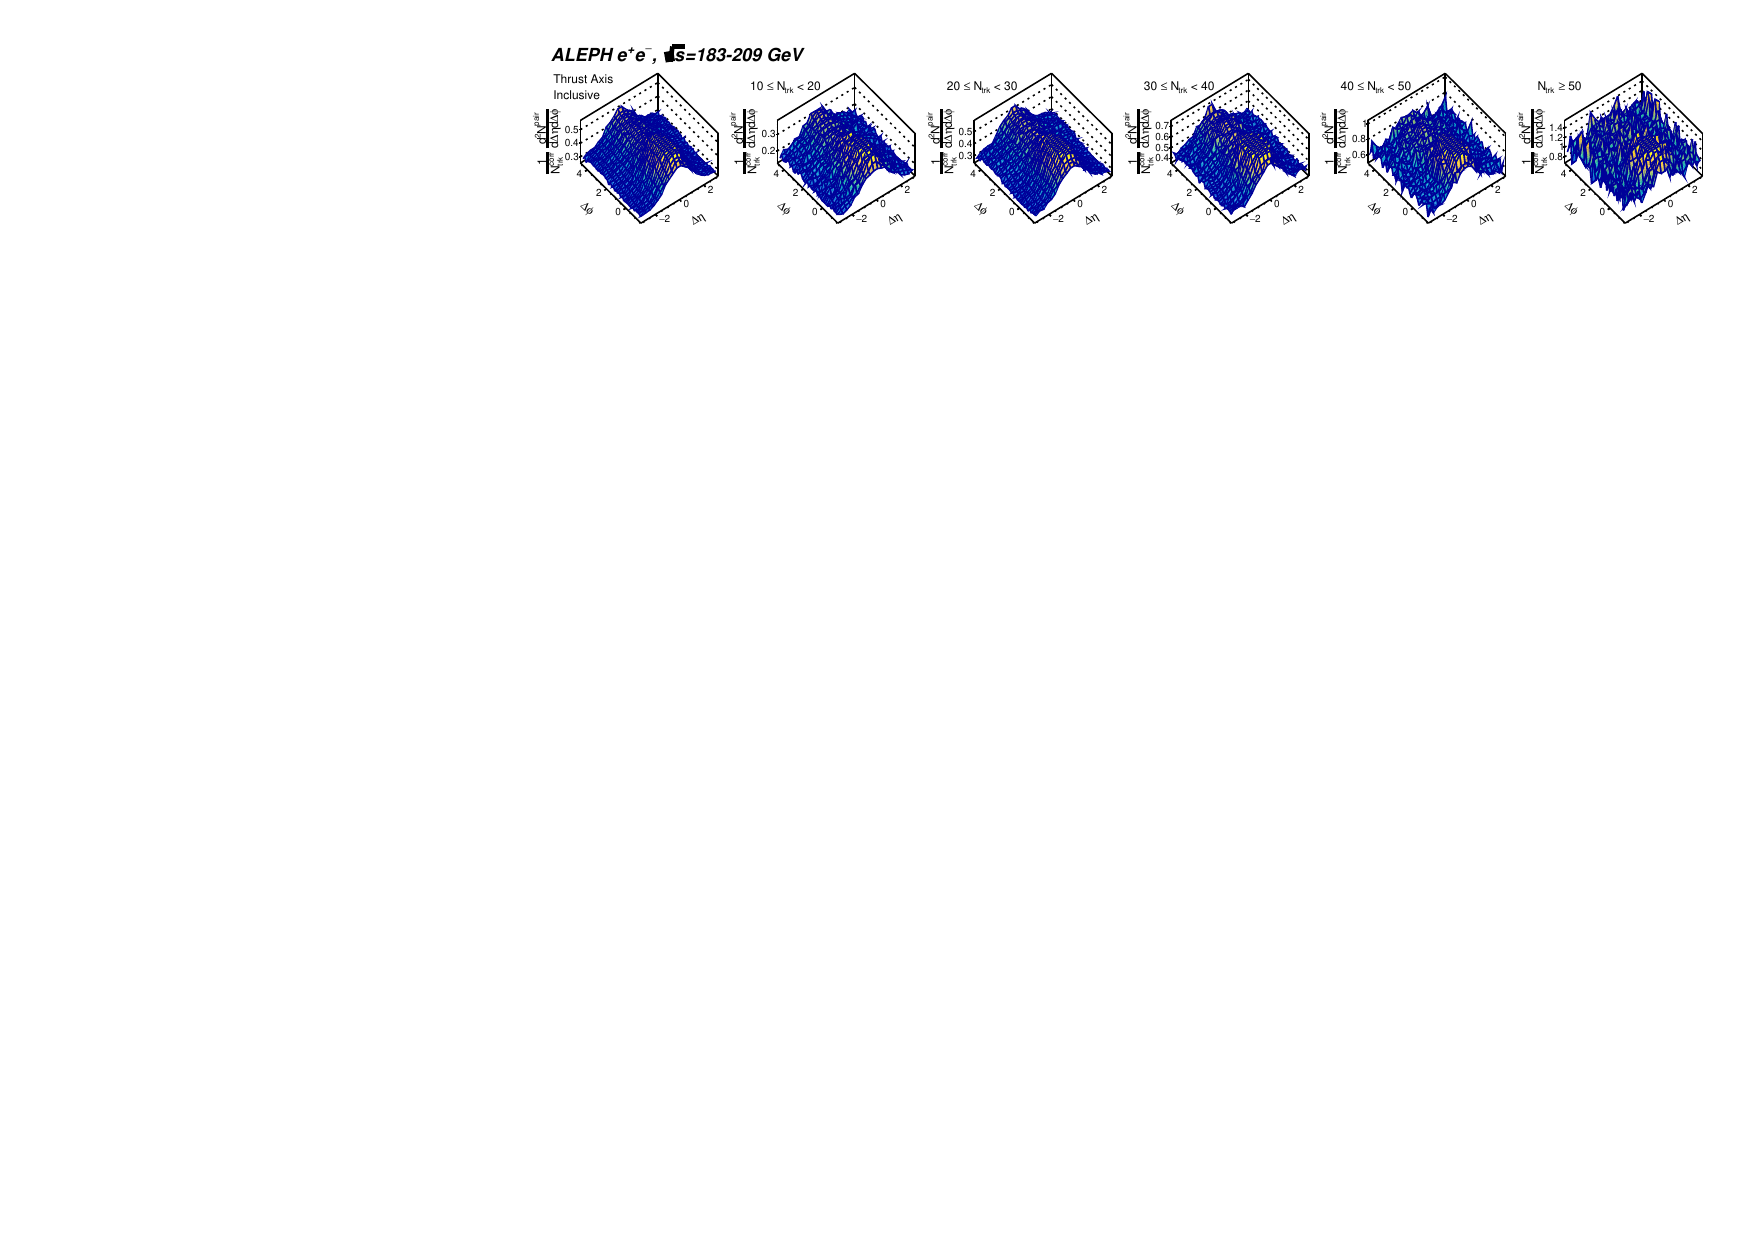}
}
\caption{Two-particle correlation function for $0 < p_T < 0.5$~GeV with the high-energy sample in the thrust axis analysis. Results are shown multiplicity-inclusively and as a function of the offline multiplicity in $[10,20), [20,30), [30,40), [40,50), [50, \infty)$ intervals.}
\label{fig:EnergyCut_ge_100_TransPtCut_0.0_0.5_thrust}
\end{figure}

\begin{figure}[ht]
\centering
\makebox[\textwidth][c]{
    \includegraphics[width=1.2\textwidth]{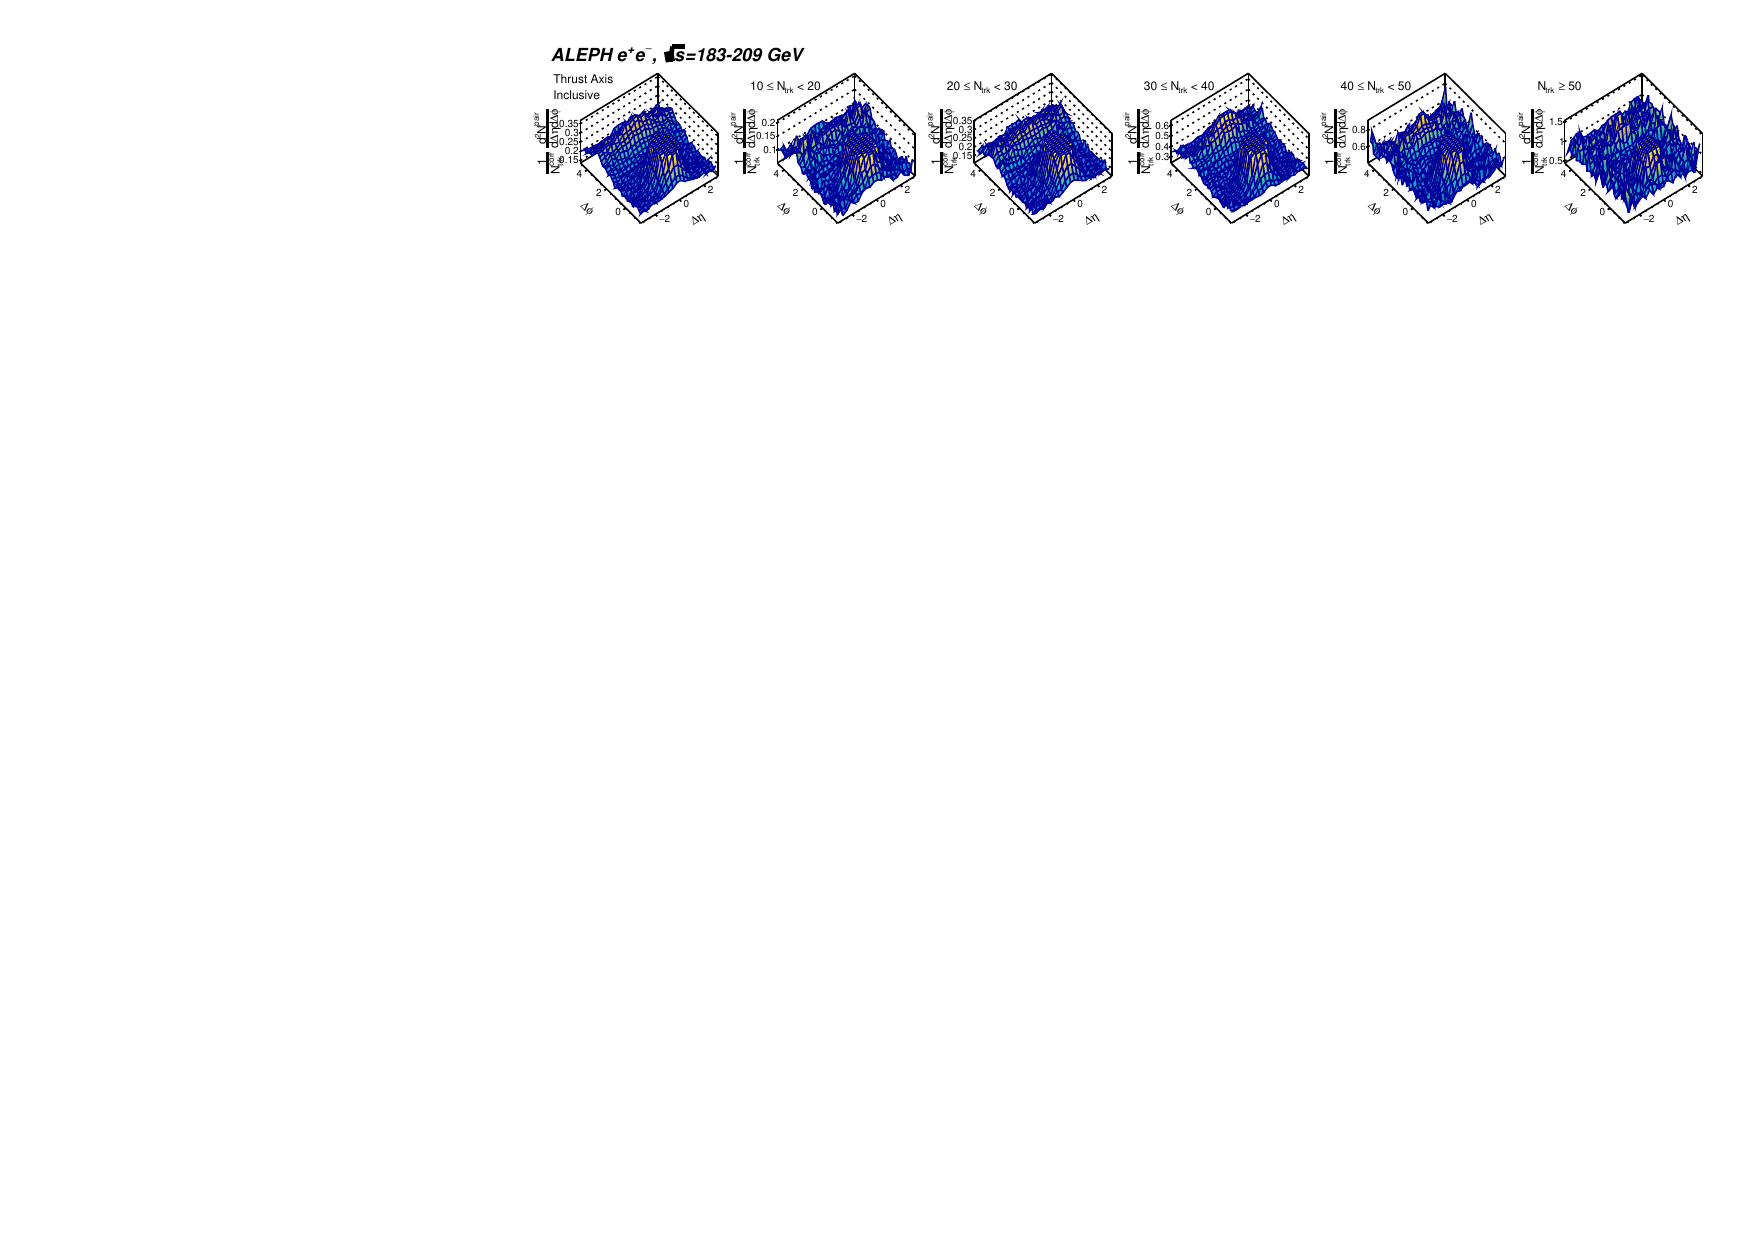}
}
\caption{Two-particle correlation function for $0.5 < p_T < 1$~GeV with the high-energy sample in the thrust axis analysis. Results are shown multiplicity-inclusively and as a function of the offline multiplicity in $[10,20), [20,30), [30,40), [40,50), [50, \infty)$ intervals.}
\label{fig:EnergyCut_ge_100_TransPtCut_0.5_1.0_thrust}
\end{figure}

\begin{figure}[ht]
\centering
\makebox[\textwidth][c]{
    \includegraphics[width=1.2\textwidth]{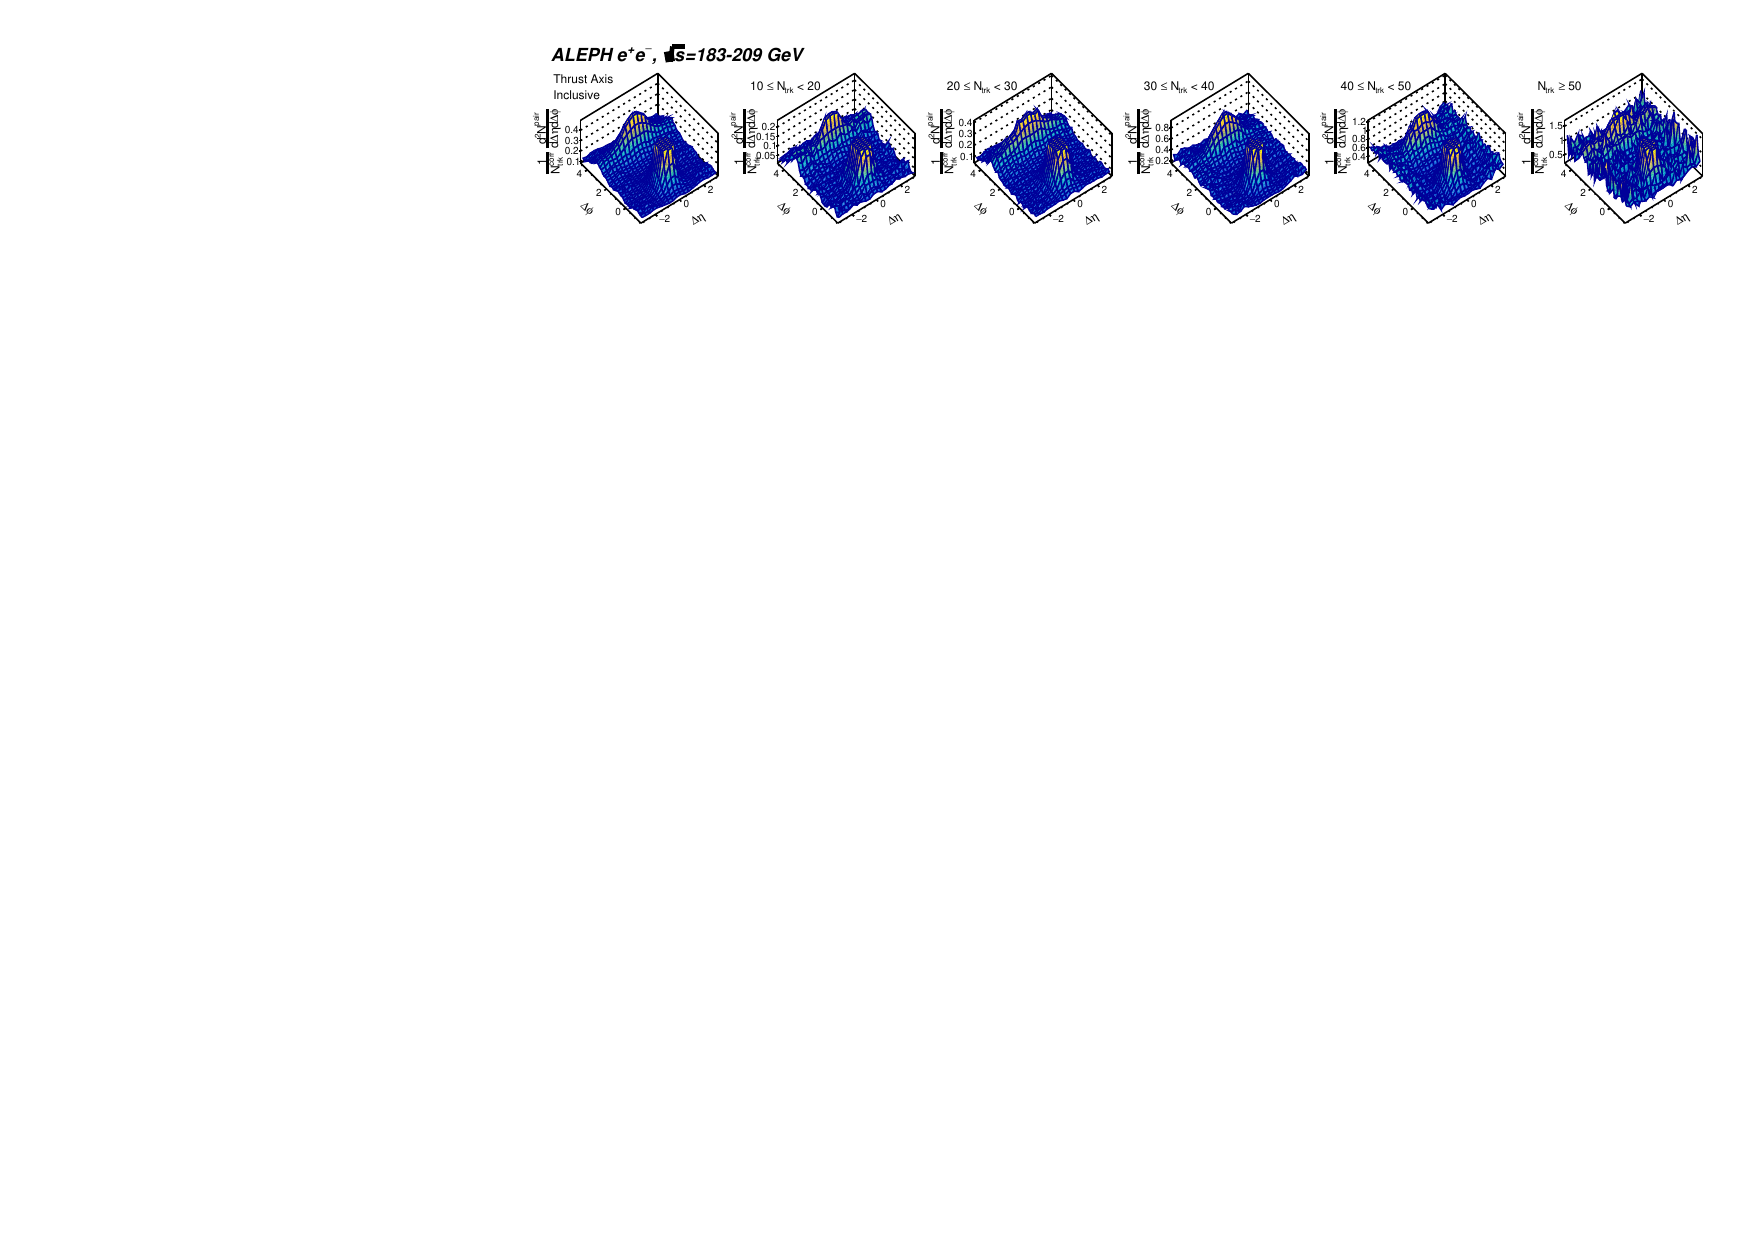}
}
\caption{Two-particle correlation function for $1 < p_T < 2$~GeV with the high-energy sample in the thrust axis analysis. Results are shown multiplicity-inclusively and as a function of the offline multiplicity in $[10,20), [20,30), [30,40), [40,50), [50, \infty)$ intervals.}
\label{fig:EnergyCut_ge_100_TransPtCut_1.0_2.0_thrust}
\end{figure}

\begin{figure}[ht]
\centering
\makebox[\textwidth][c]{
    \includegraphics[width=1.2\textwidth]{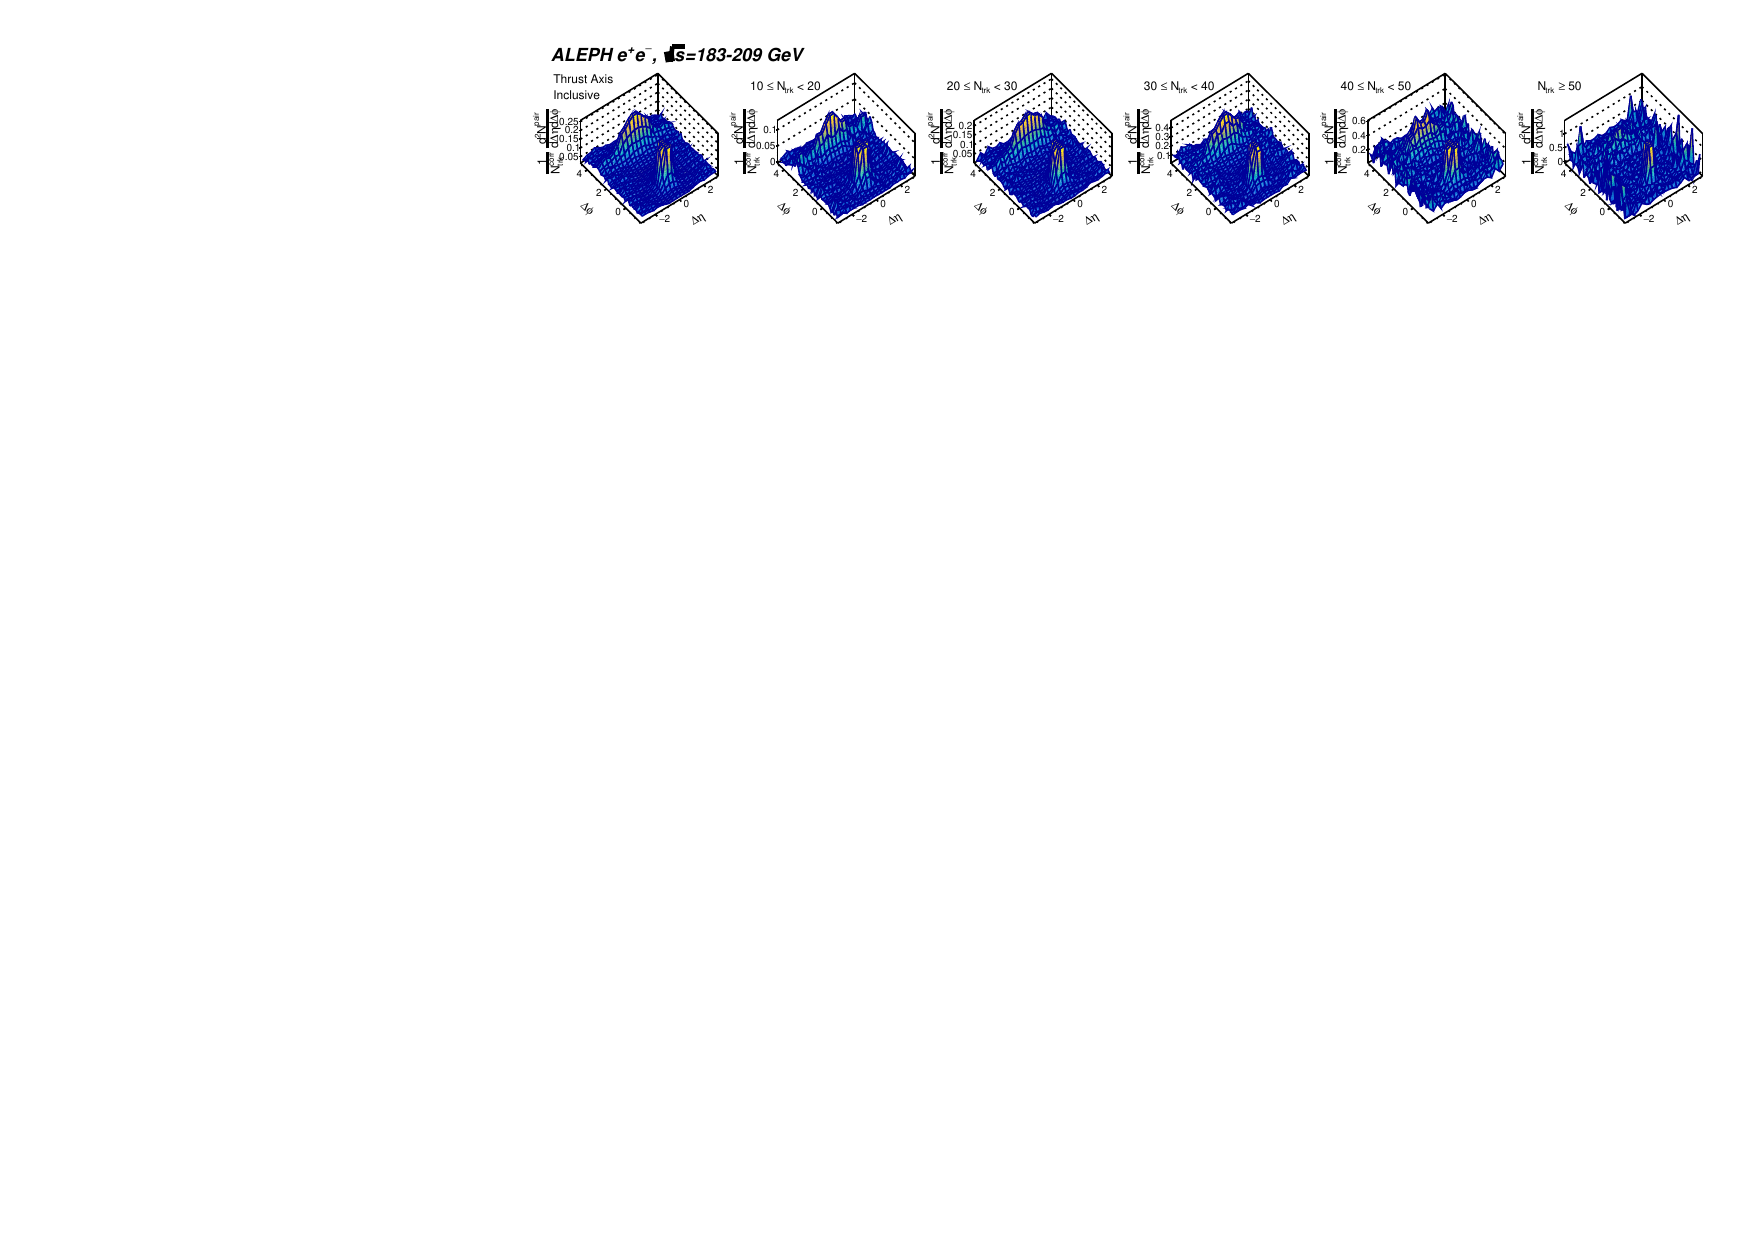}
}
\caption{Two-particle correlation function for $2 < p_T < 3$~GeV with the high-energy sample in the thrust axis analysis. Results are shown multiplicity-inclusively and as a function of the offline multiplicity in $[10,20), [20,30), [30,40), [40,50), [50, \infty)$ intervals.}
\label{fig:EnergyCut_ge_100_TransPtCut_2.0_3.0_thrust}
\end{figure}

\begin{figure}[ht]
\centering
\makebox[\textwidth][c]{
    \includegraphics[width=1.2\textwidth]{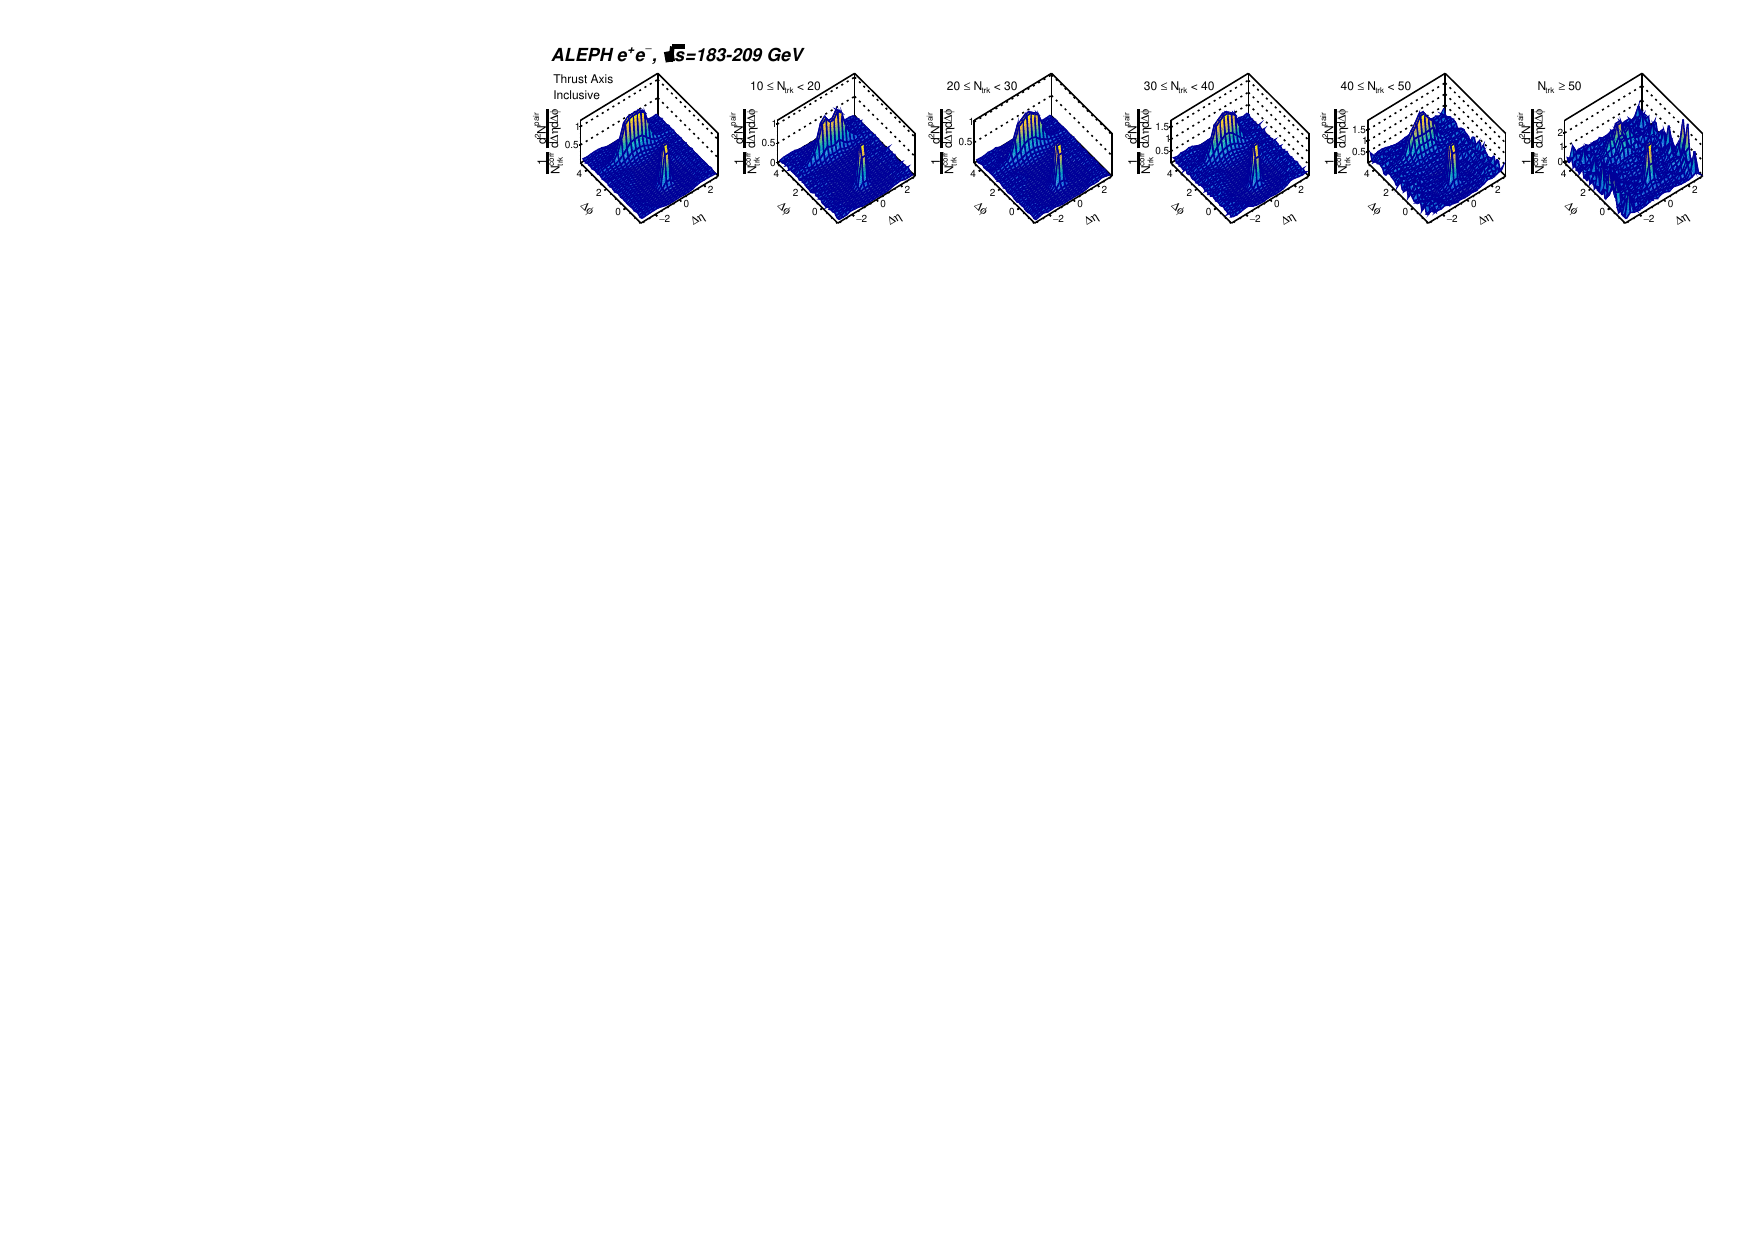}
}
\caption{Two-particle correlation function for $p_T > 3$~GeV with the high-energy sample in the thrust axis analysis. Results are shown multiplicity-inclusively and as a function of the offline multiplicity in $[10,20), [20,30), [30,40), [40,50), [50, \infty)$ intervals.}
\label{fig:EnergyCut_ge_100_TransPtCut_3.0_thrust}
\end{figure}
\clearpage

%%%%%%%%%%%%%%%%%%%%%%%%%%% 1D
\begin{figure}[ht]
\centering
\makebox[\textwidth][c]{
    \includegraphics[width=1.2\textwidth]{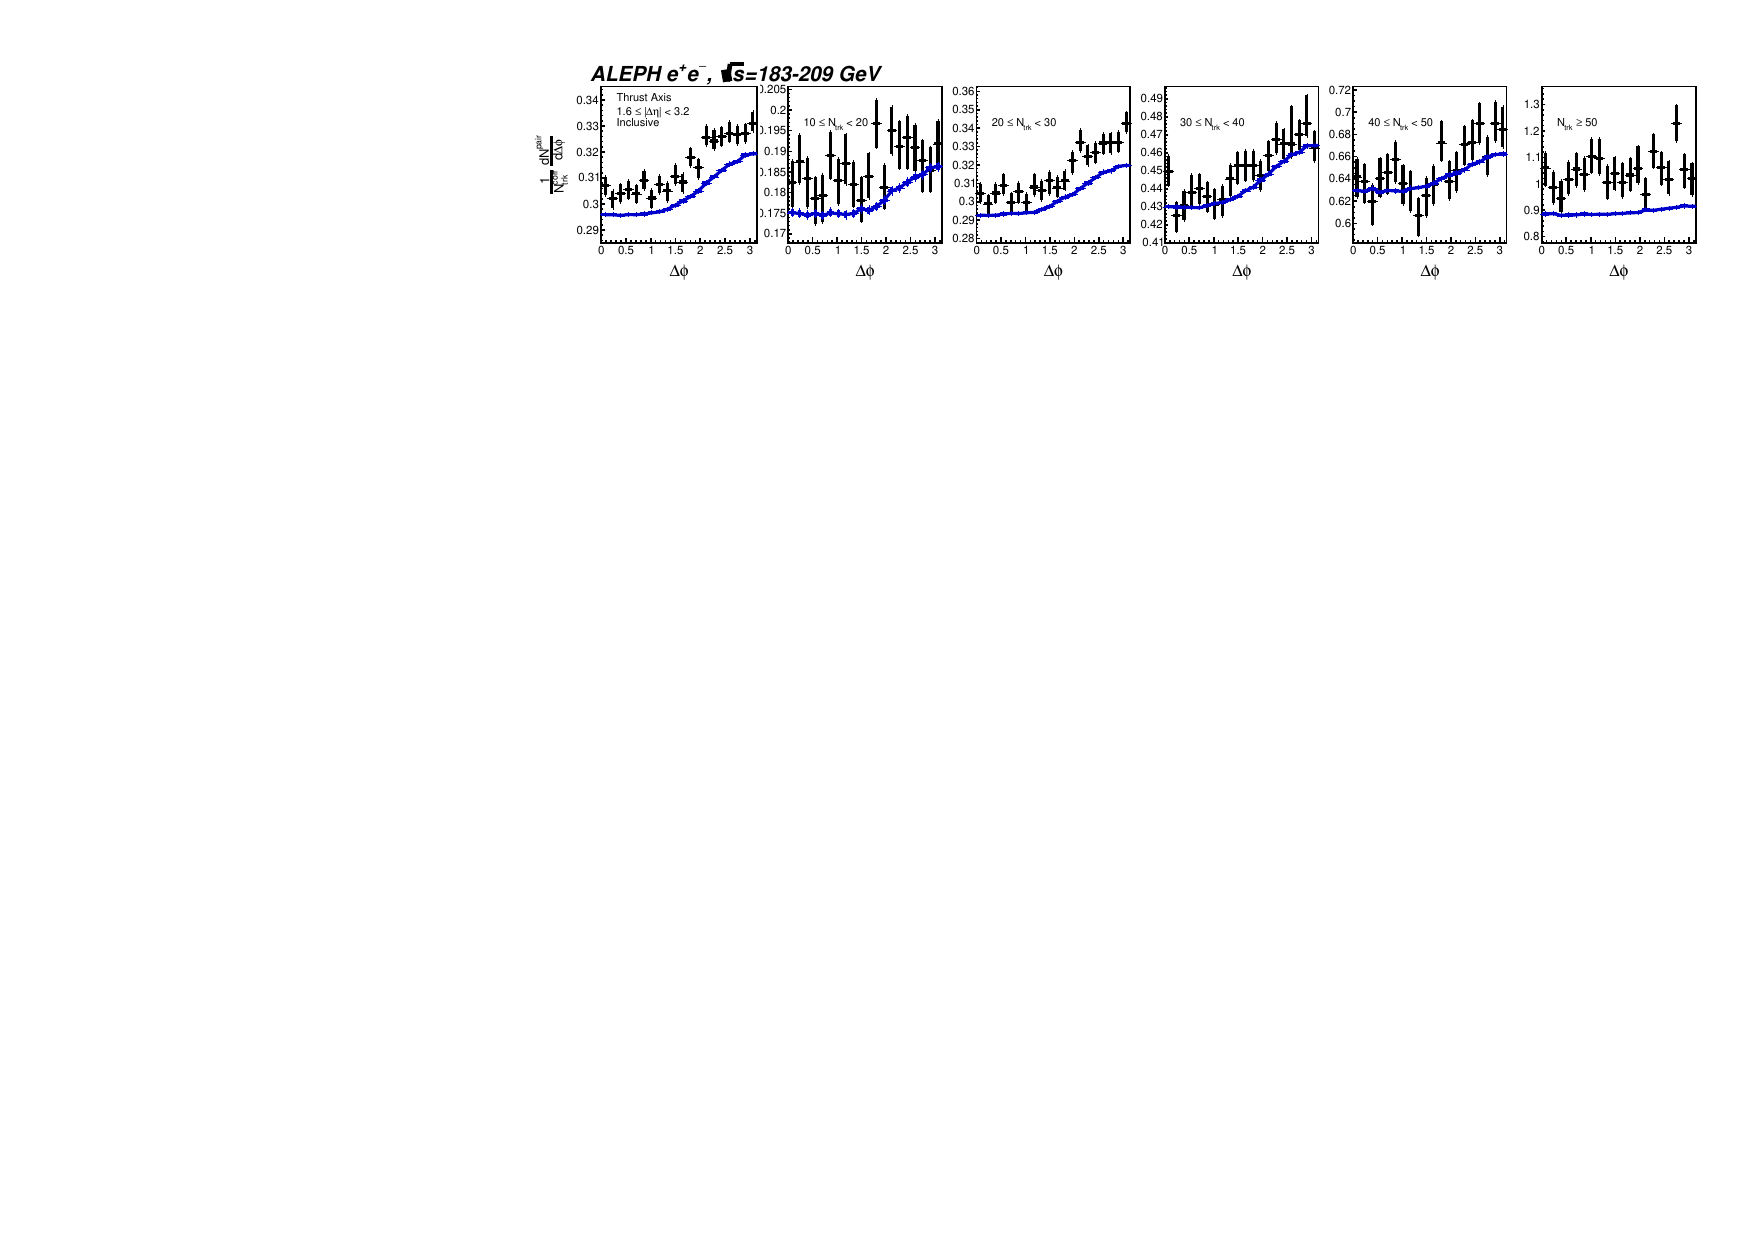}
}
\caption{Long-range azimuthal differential yields for $0 < p_T < 0.5$~GeV with the high-energy sample in the thrust axis analysis. Results are shown multiplicity-inclusively and as a function of the offline multiplicity in $[10,20), [20,30), [30,40), [40,50), [50, \infty)$ intervals.}
\label{fig:EnergyCut_ge_100_TransPtCut_0.0_0.5_thrust_1d}
\end{figure}

\begin{figure}[ht]
\centering
\makebox[\textwidth][c]{
    \includegraphics[width=1.2\textwidth]{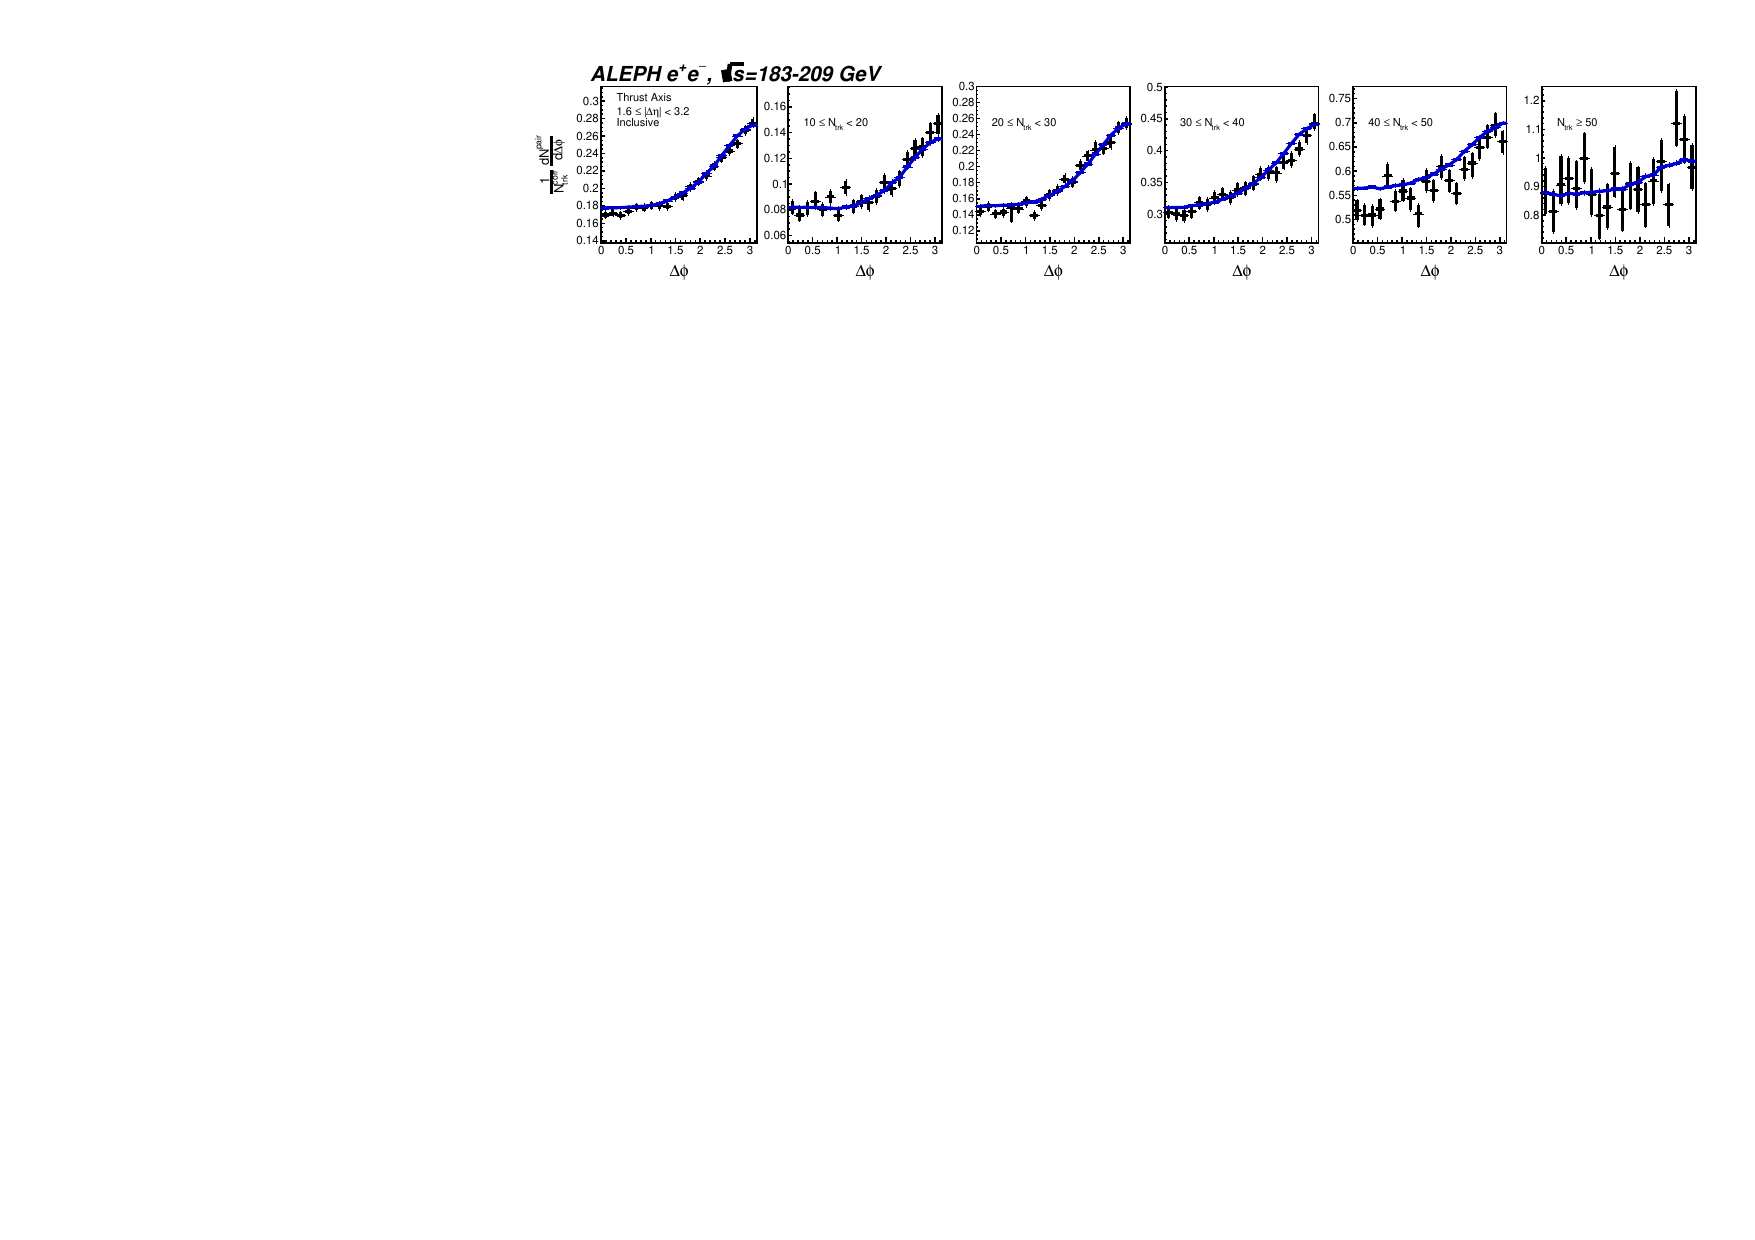}
}
\caption{Long-range azimuthal differential yields for $0.5 < p_T < 1$~GeV with the high-energy sample in the thrust axis analysis. Results are shown multiplicity-inclusively and as a function of the offline multiplicity in $[10,20), [20,30), [30,40), [40,50), [50, \infty)$ intervals.}
\label{fig:EnergyCut_ge_100_TransPtCut_0.5_1.0_thrust_1d}
\end{figure}

\begin{figure}[ht]
\centering
\makebox[\textwidth][c]{
    \includegraphics[width=1.2\textwidth]{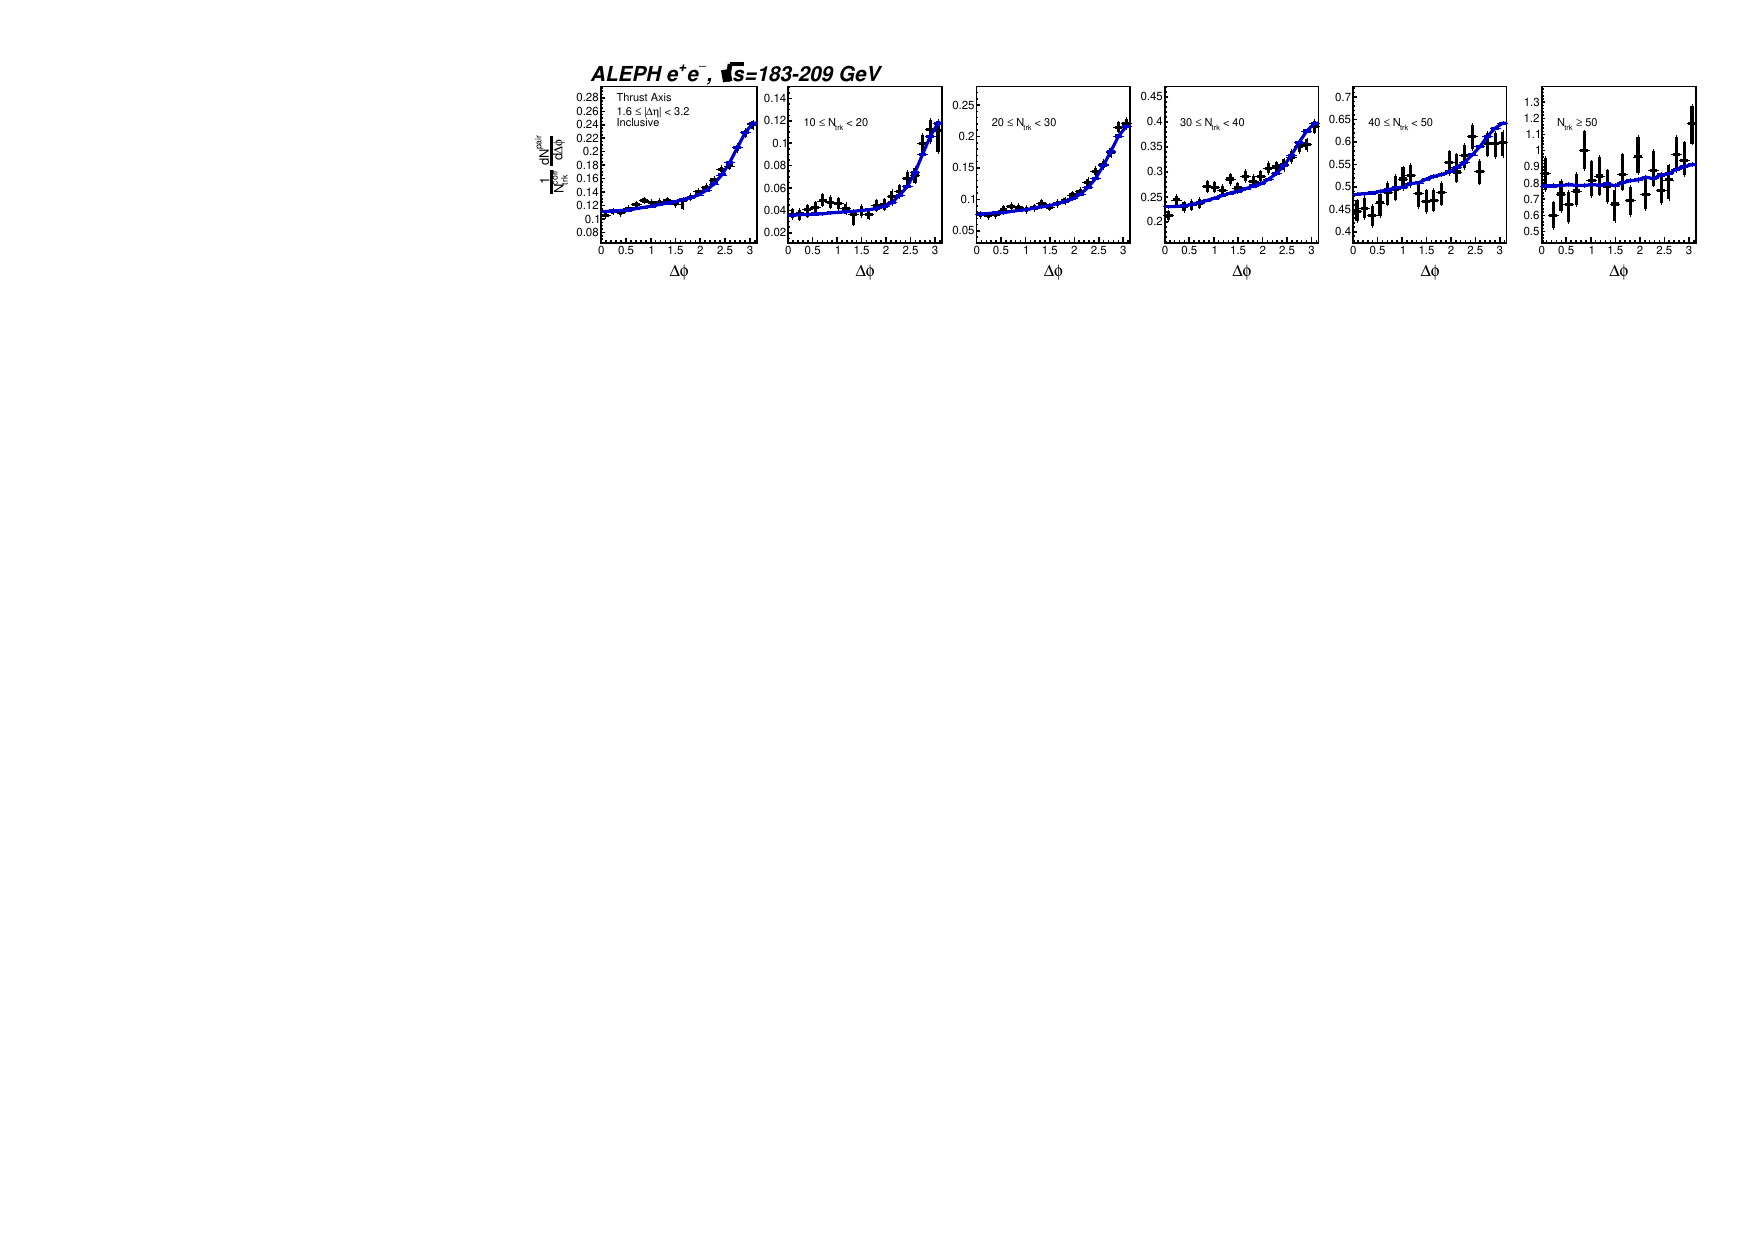}
}
\caption{Long-range azimuthal differential yields for $1 < p_T < 2$~GeV with the high-energy sample in the thrust axis analysis. Results are shown multiplicity-inclusively and as a function of the offline multiplicity in $[10,20), [20,30), [30,40), [40,50), [50, \infty)$ intervals.}
\label{fig:EnergyCut_ge_100_TransPtCut_1.0_2.0_thrust_1d}
\end{figure}

\begin{figure}[ht]
\centering
\makebox[\textwidth][c]{
    \includegraphics[width=1.2\textwidth]{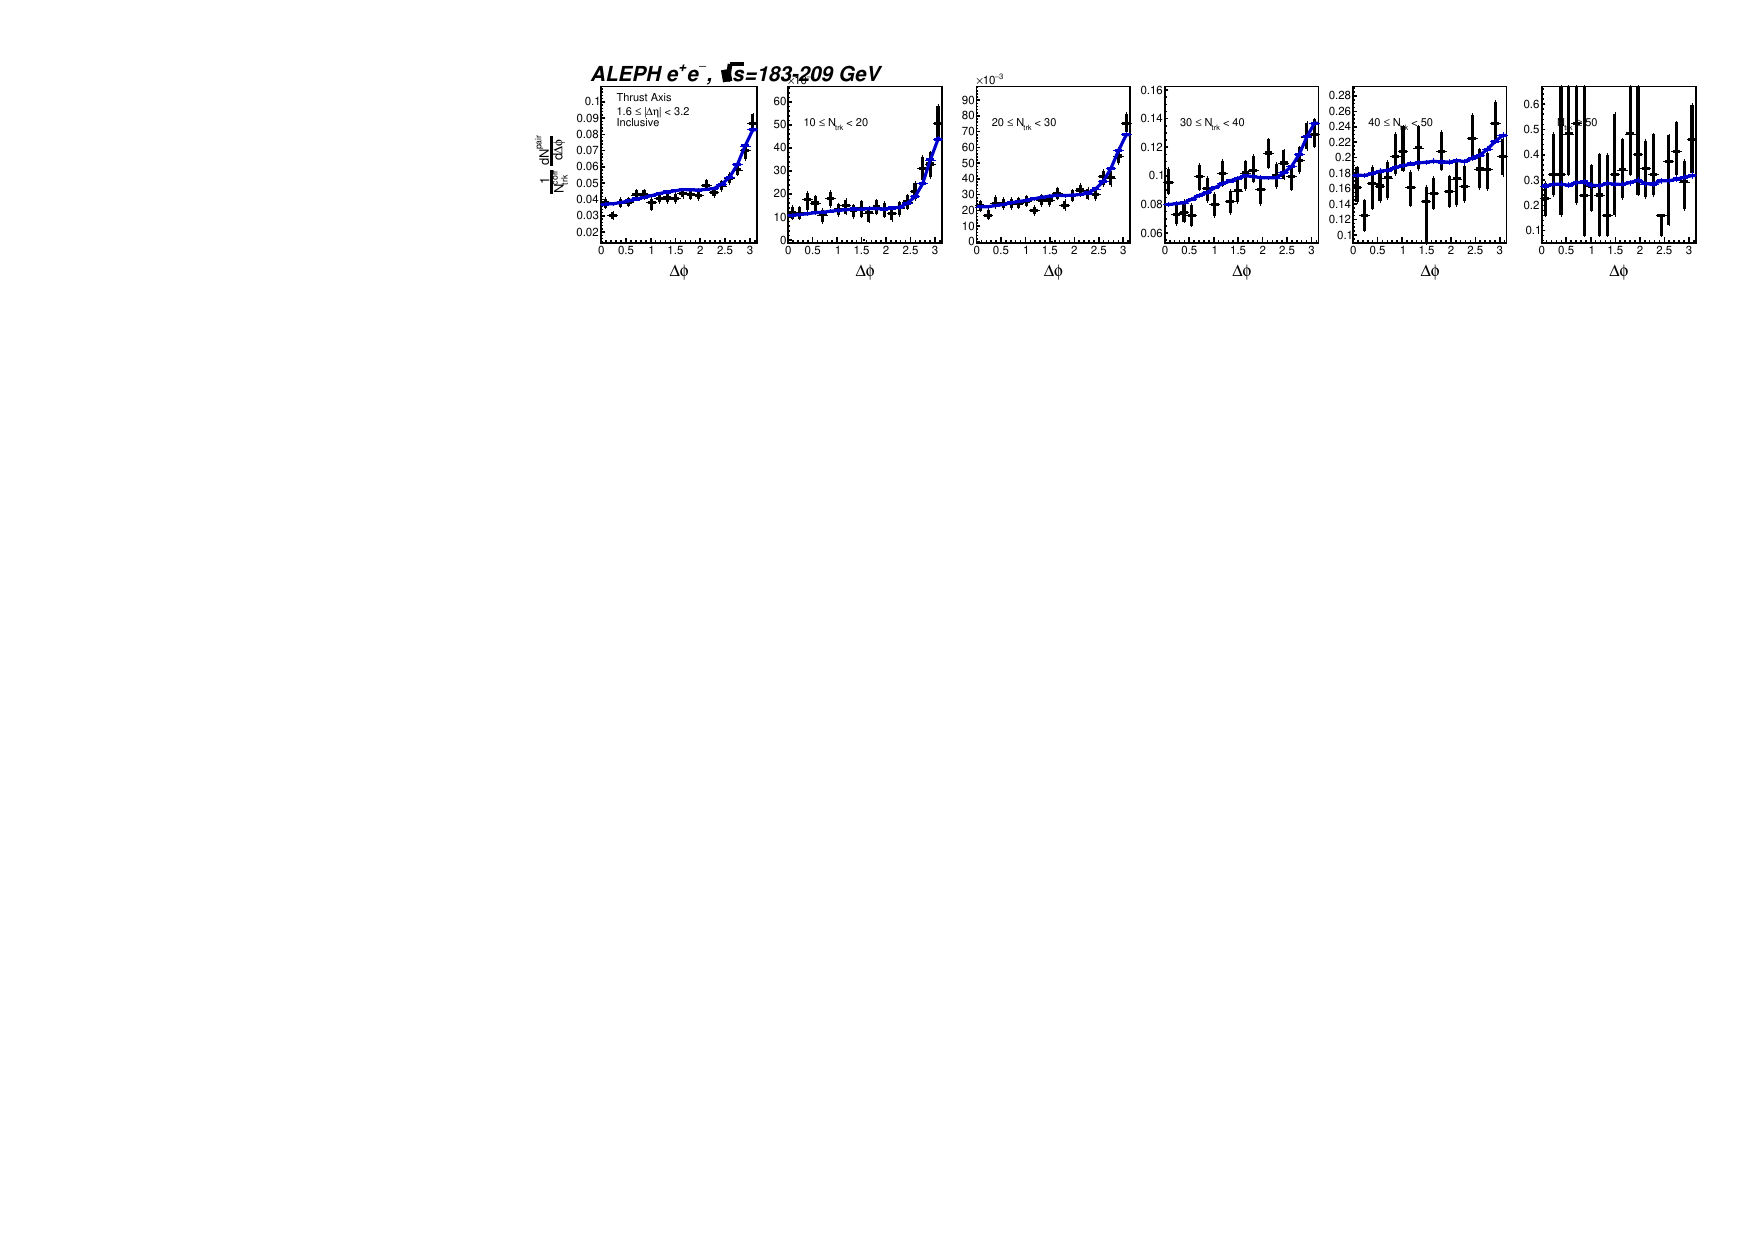}
}
\caption{Long-range azimuthal differential yields for $2 < p_T < 3$~GeV with the high-energy sample in the thrust axis analysis. Results are shown multiplicity-inclusively and as a function of the offline multiplicity in $[10,20), [20,30), [30,40), [40,50), [50, \infty)$ intervals.}
\label{fig:EnergyCut_ge_100_TransPtCut_2.0_3.0_thrust_1d}
\end{figure}

\begin{figure}[ht]
\centering
\makebox[\textwidth][c]{
    \includegraphics[width=1.2\textwidth]{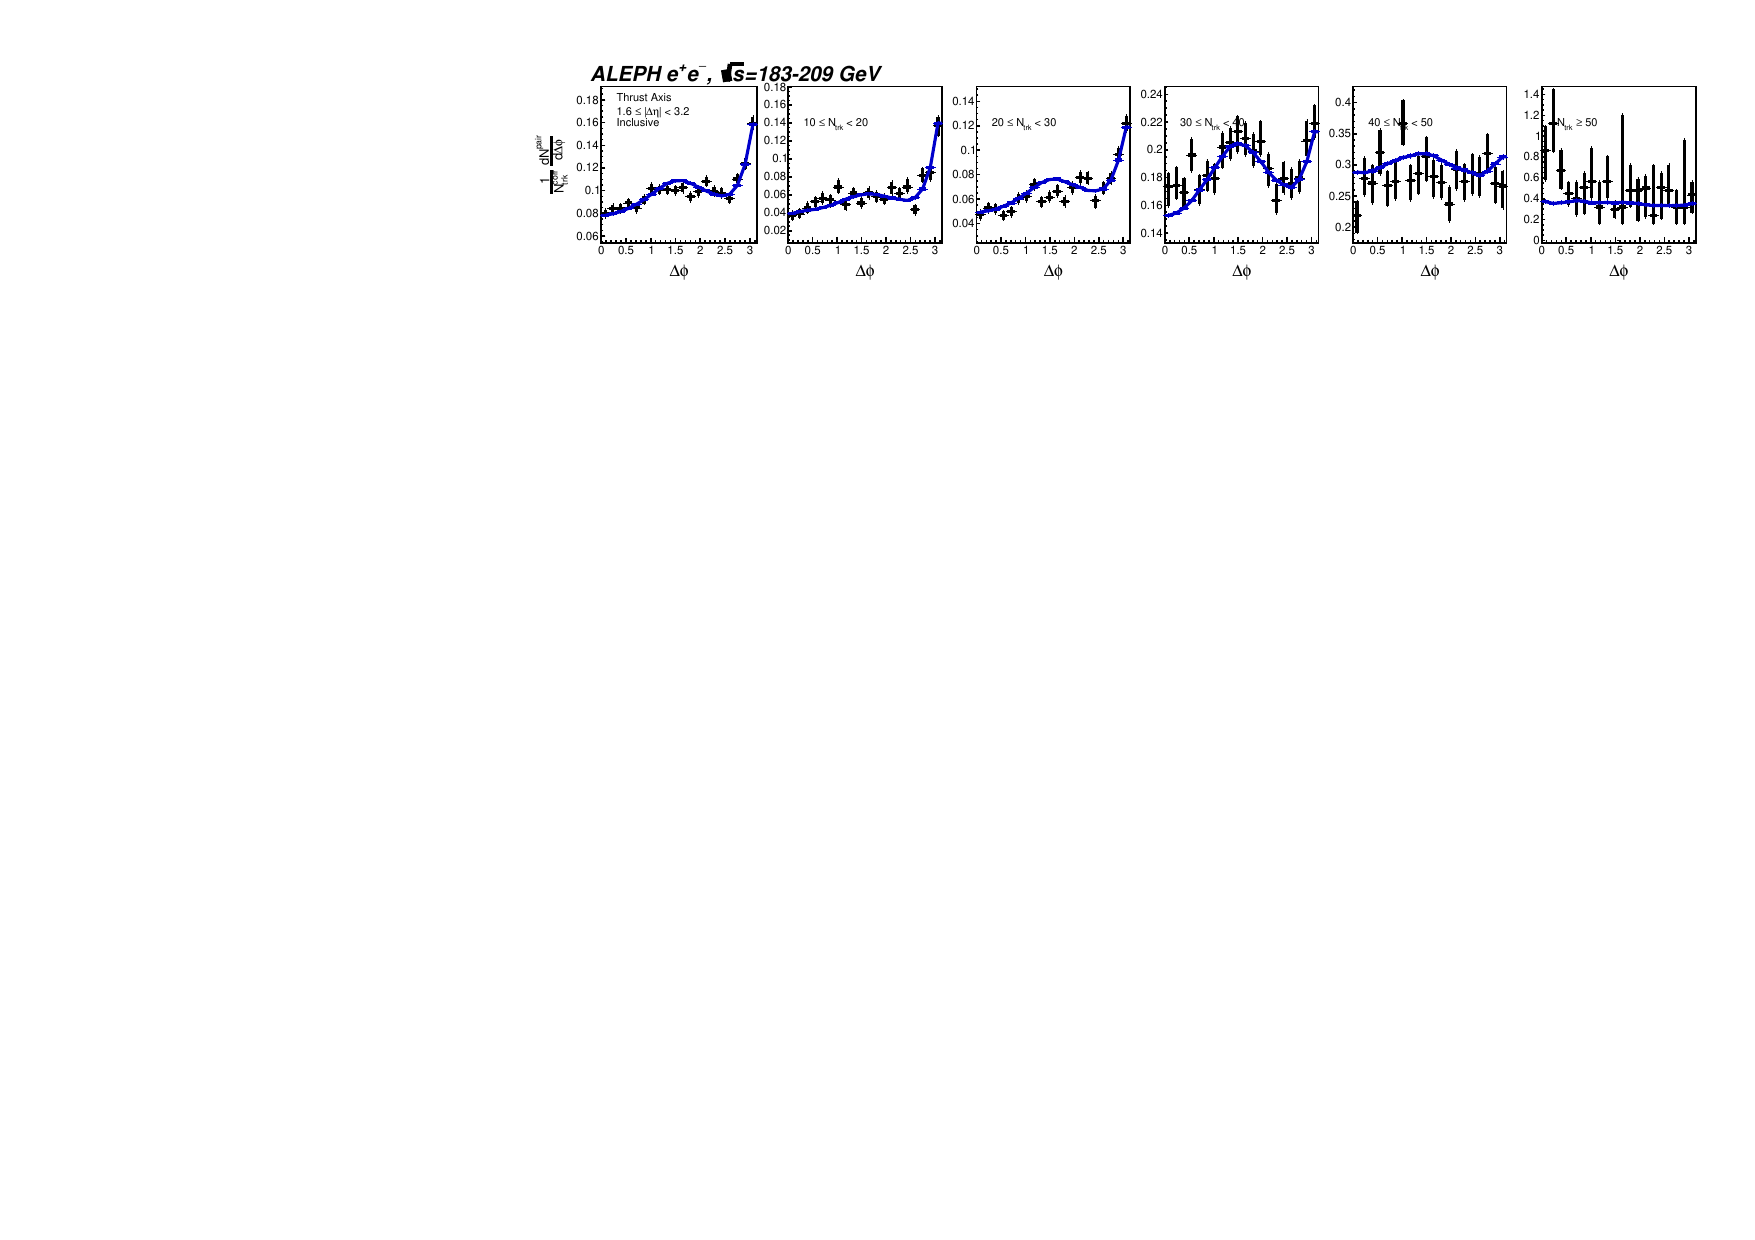}
}
\caption{Long-range azimuthal differential yields for $p_T < 3$~GeV with the high-energy sample in the thrust axis analysis. Results are shown multiplicity-inclusively and as a function of the offline multiplicity in $[10,20), [20,30), [30,40), [40,50), [50, \infty)$ intervals.}
\label{fig:EnergyCut_ge_100_TransPtCut_3.0_thrust_1d}
\end{figure}
\clearpage

\section{Single-particle anisotropy coefficients}
\label{app:flow}
\subsection*{${\rm sign}(\Delta V_1) \sqrt{\Delta V_1}$}
%%%%%%%%%%%%%%%%%%%% Beam axis: Delta v1 vs pt
\begin{figure}[ht]
\centering
    \begin{subfigure}[b]{0.48\textwidth}
    \includegraphics[width=\textwidth]{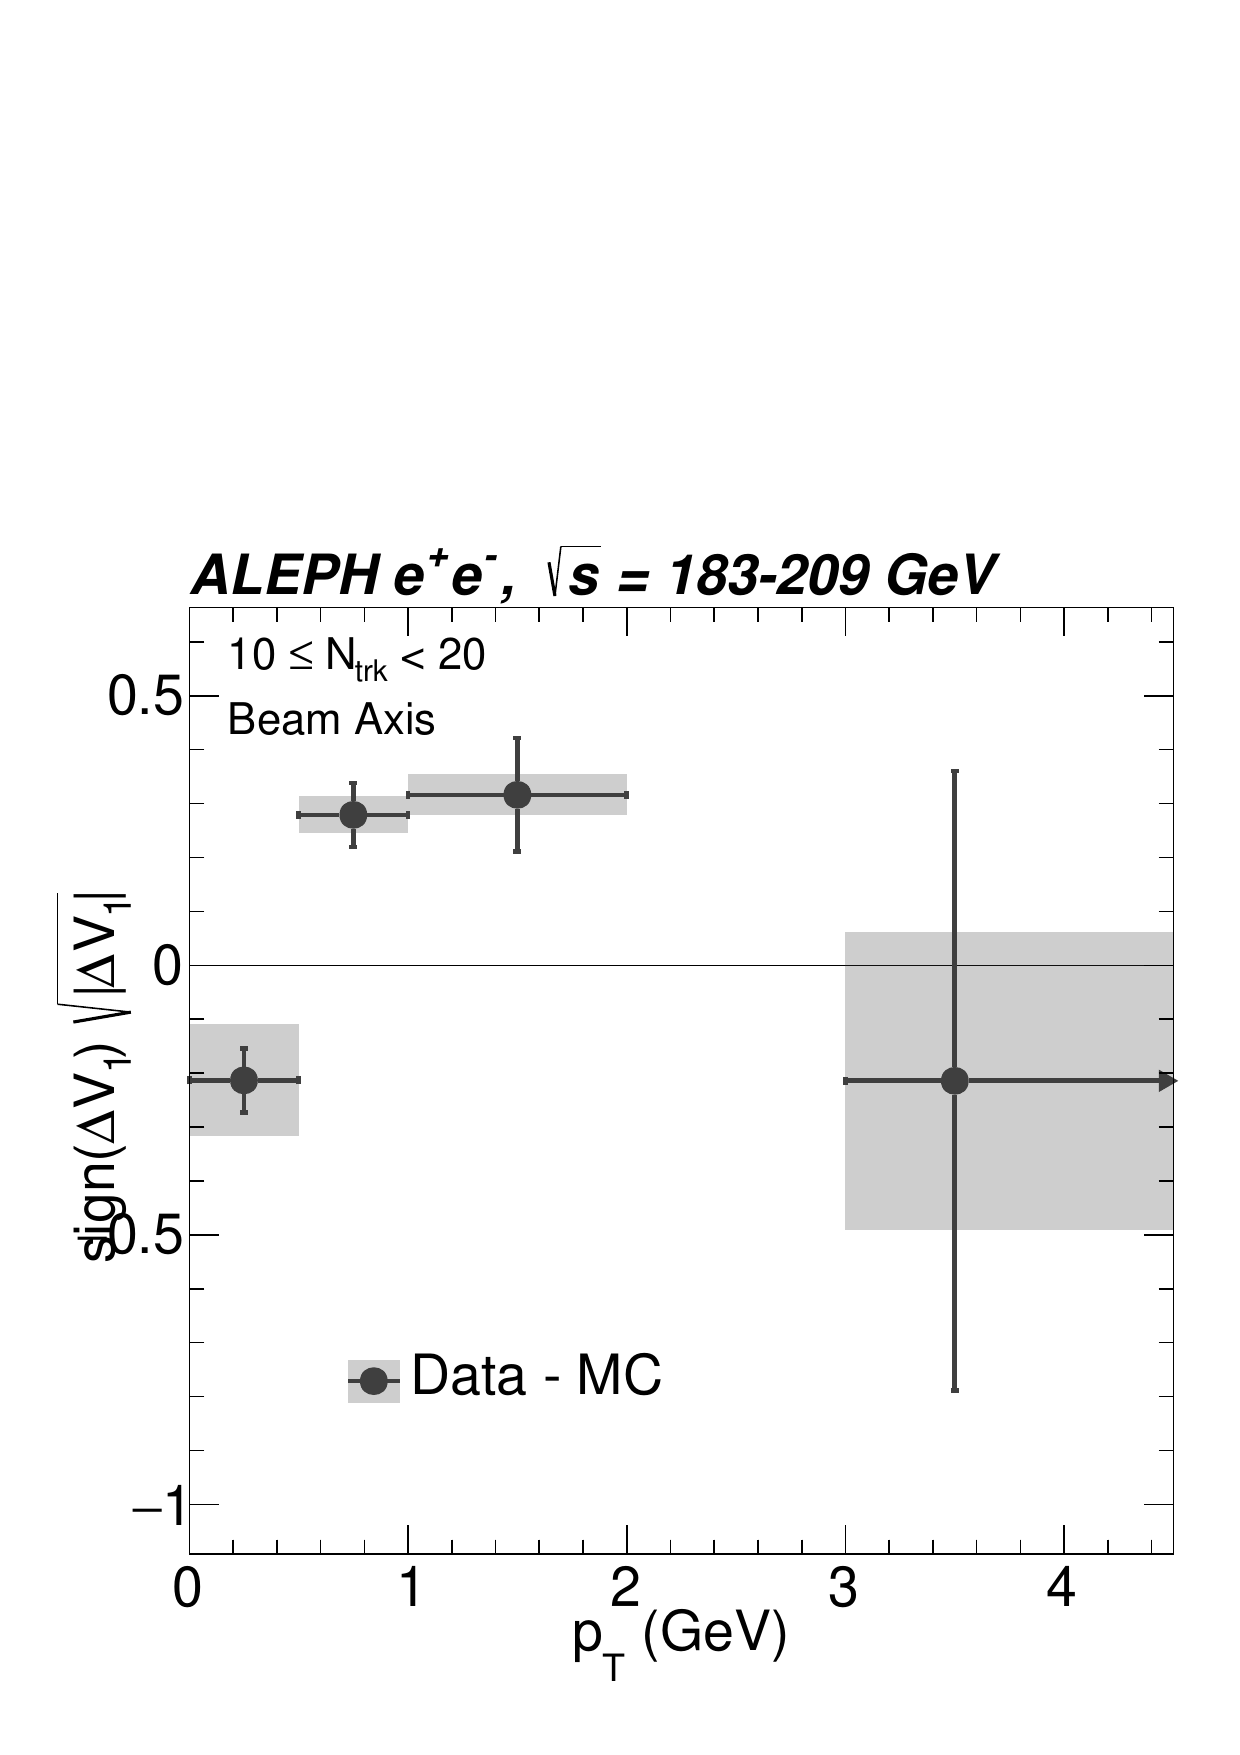}
    \caption{$10 \le {\rm N}_{\rm trk} < 20$}
        %\label{fig:}
    \end{subfigure}
    \begin{subfigure}[b]{0.48\textwidth}
    \includegraphics[width=\textwidth]{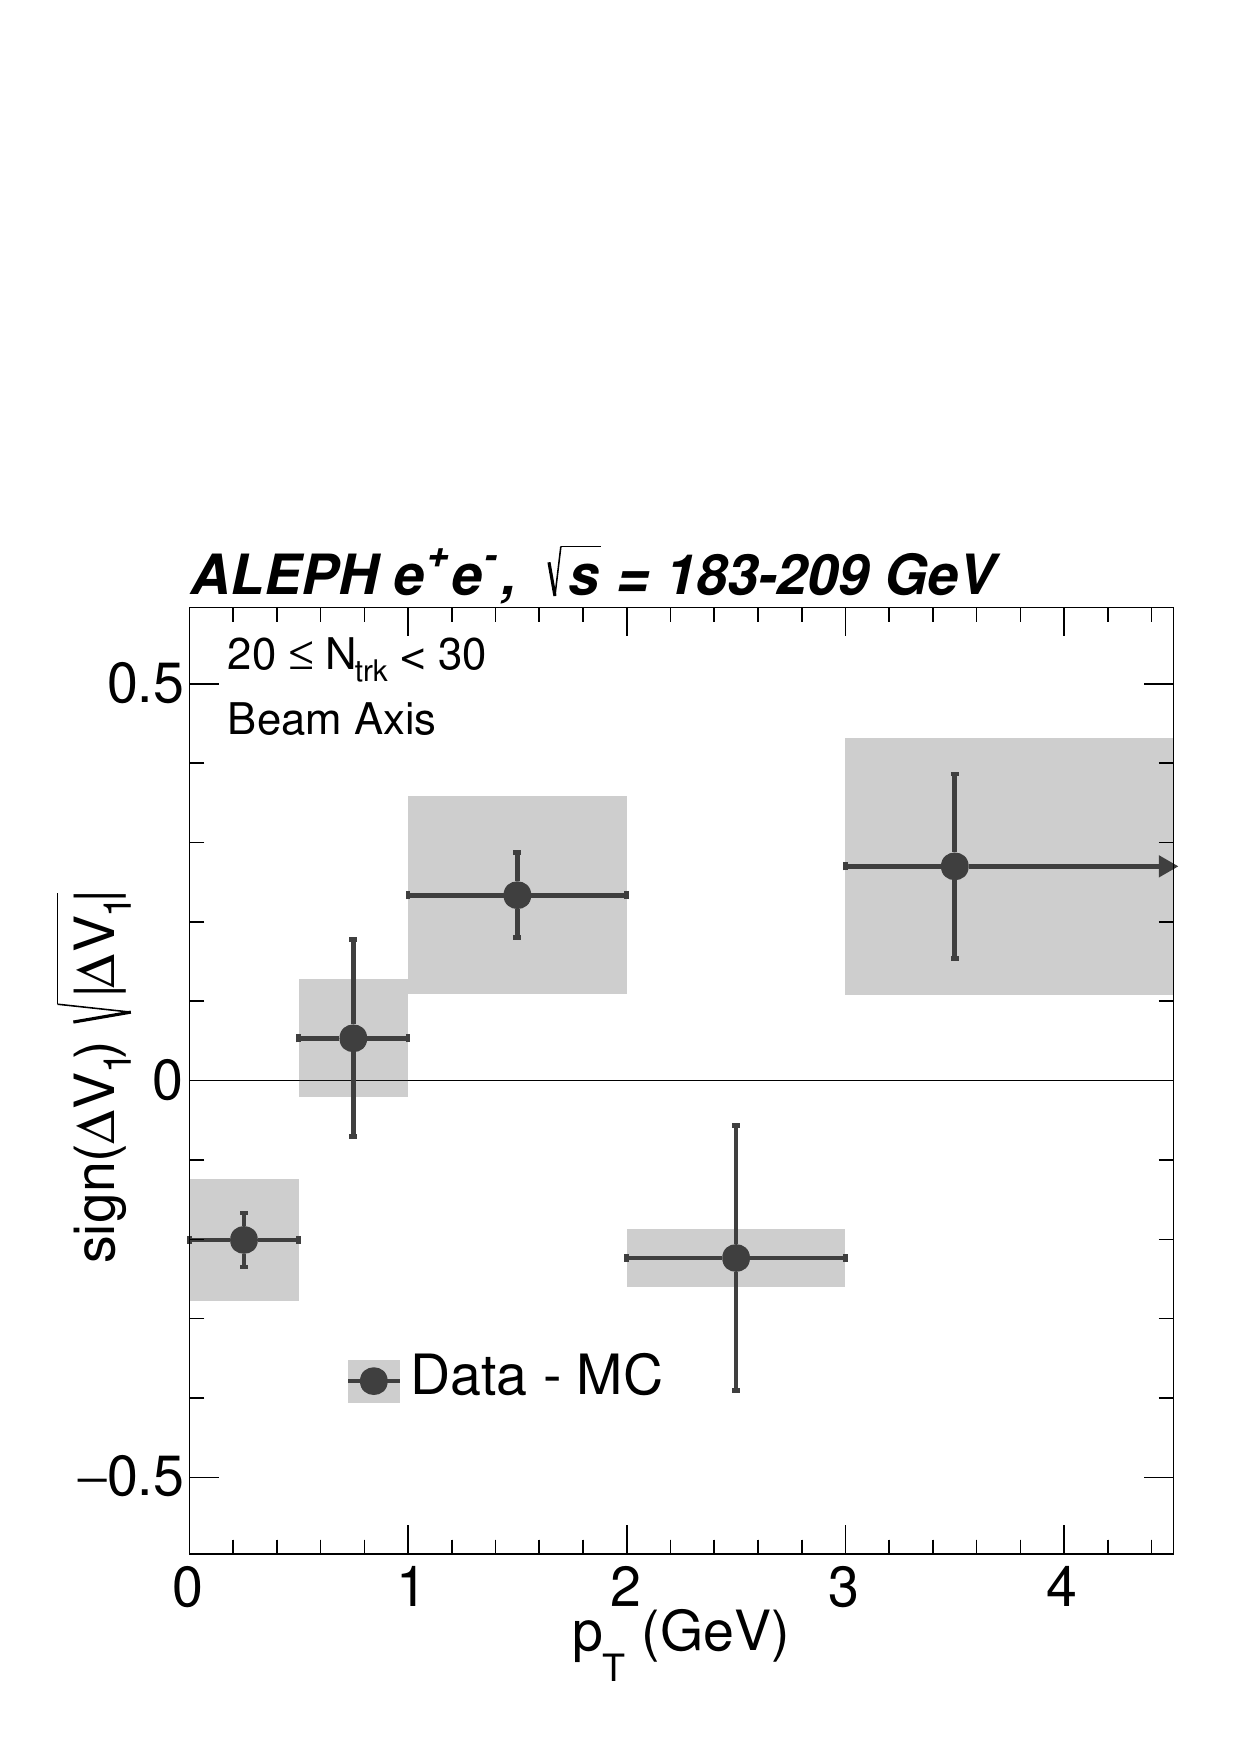}
    \caption{$20 \le {\rm N}_{\rm trk} < 30$}
        %\label{fig:}
    \end{subfigure}
    \begin{subfigure}[b]{0.48\textwidth}
    \includegraphics[width=\textwidth]{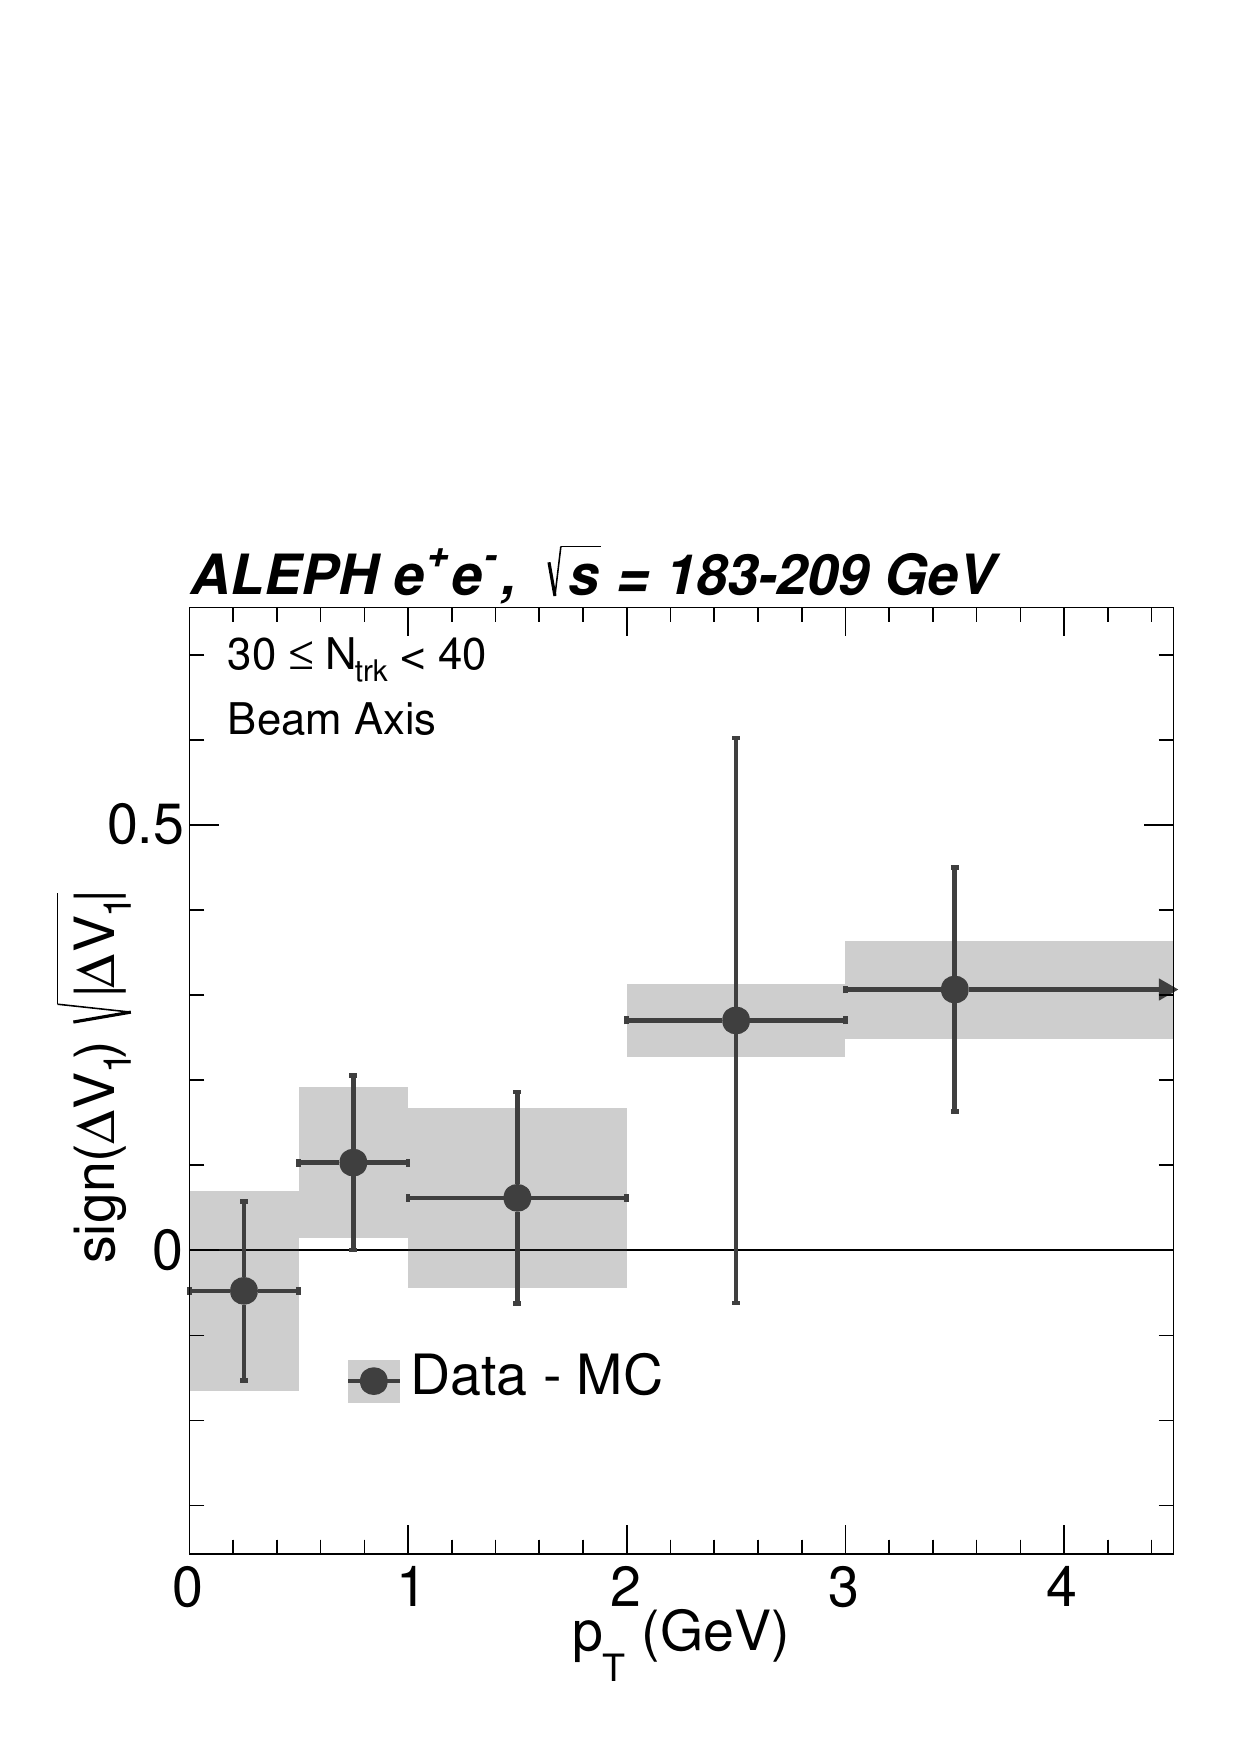}
    \caption{$30 \le {\rm N}_{\rm trk} < 40$}
        %\label{fig:}
    \end{subfigure}
    \begin{subfigure}[b]{0.48\textwidth}
    \includegraphics[width=\textwidth]{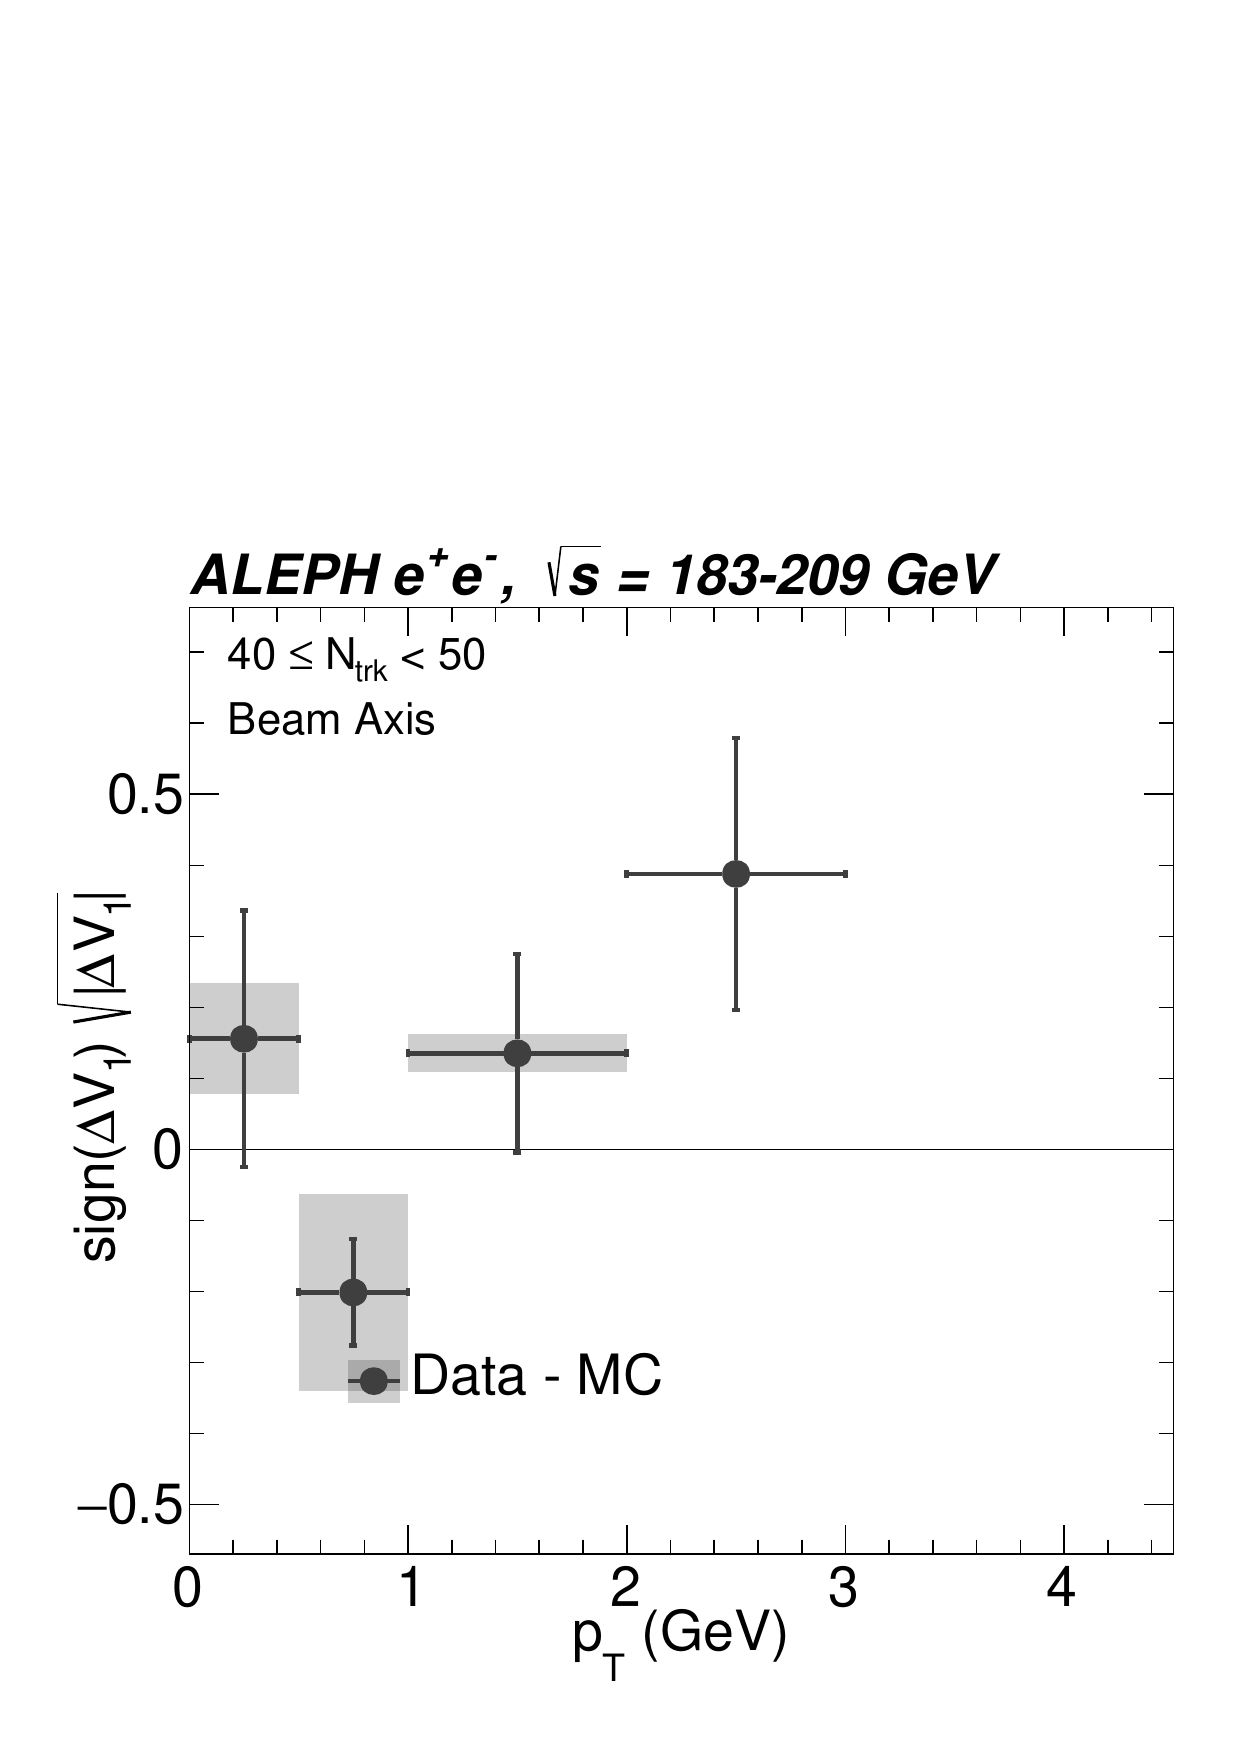}
    \caption{$40 \le {\rm N}_{\rm trk} < 50$}
        %\label{fig:}
    \end{subfigure}
    \begin{subfigure}[b]{0.48\textwidth}
    \includegraphics[width=\textwidth]{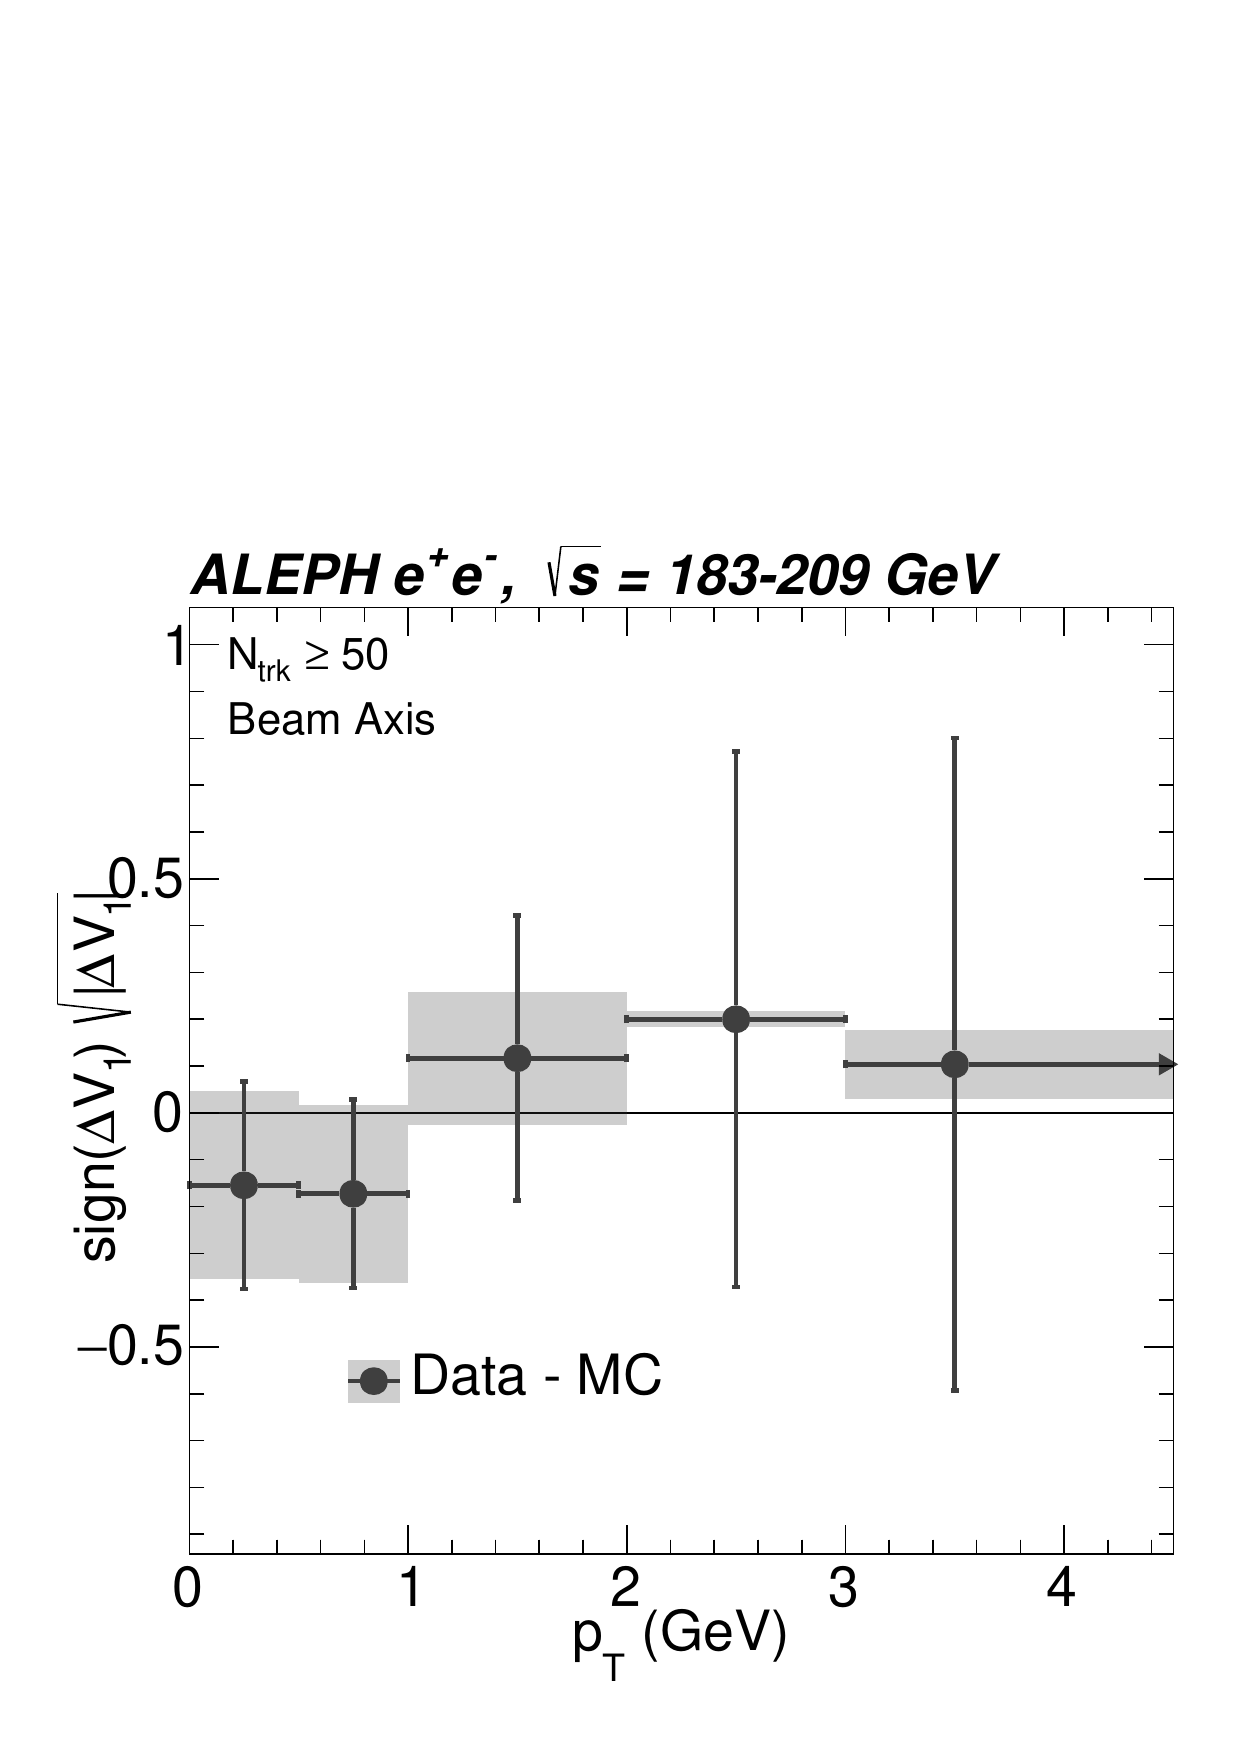}
    \caption{${\rm N}_{\rm trk} \ge 50$}
        %\label{fig:}
    \end{subfigure}
\caption{$\Delta v_{1}$ as a function of the track pairs' $p_{T}$ requirement in different  multiplicity intervals for the beam axis analysis for LEP-II high-energy sample.}
\label{fig:Dv1VsPt_beam}
\end{figure}

%%%%%%%%%%%%%%%%%%%% Thrust axis: Delta v1 vs pt
\begin{figure}[ht]
\centering
    \begin{subfigure}[b]{0.48\textwidth}
    \includegraphics[width=\textwidth]{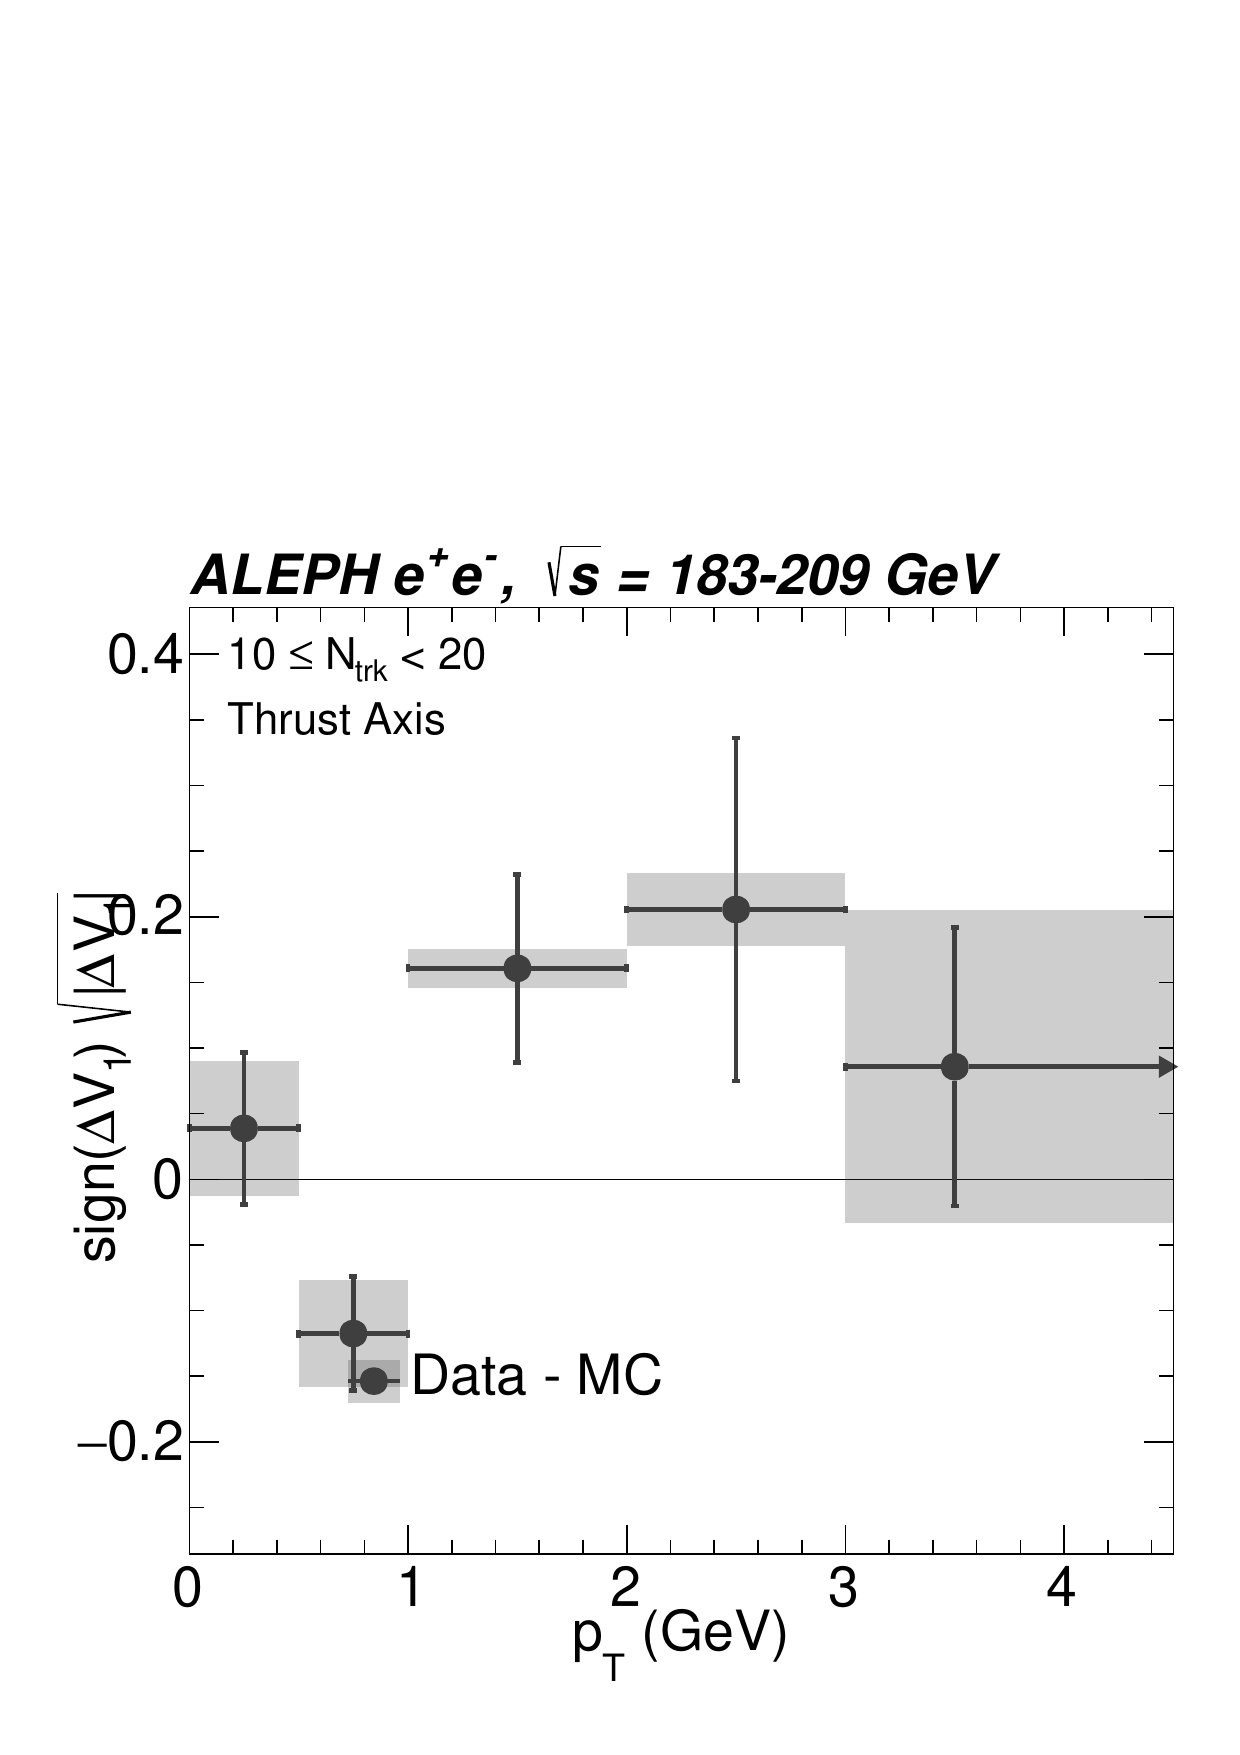}
    \caption{$10 \le {\rm N}_{\rm trk} < 20$}
        %\label{fig:}
    \end{subfigure}
    \begin{subfigure}[b]{0.48\textwidth}
    \includegraphics[width=\textwidth]{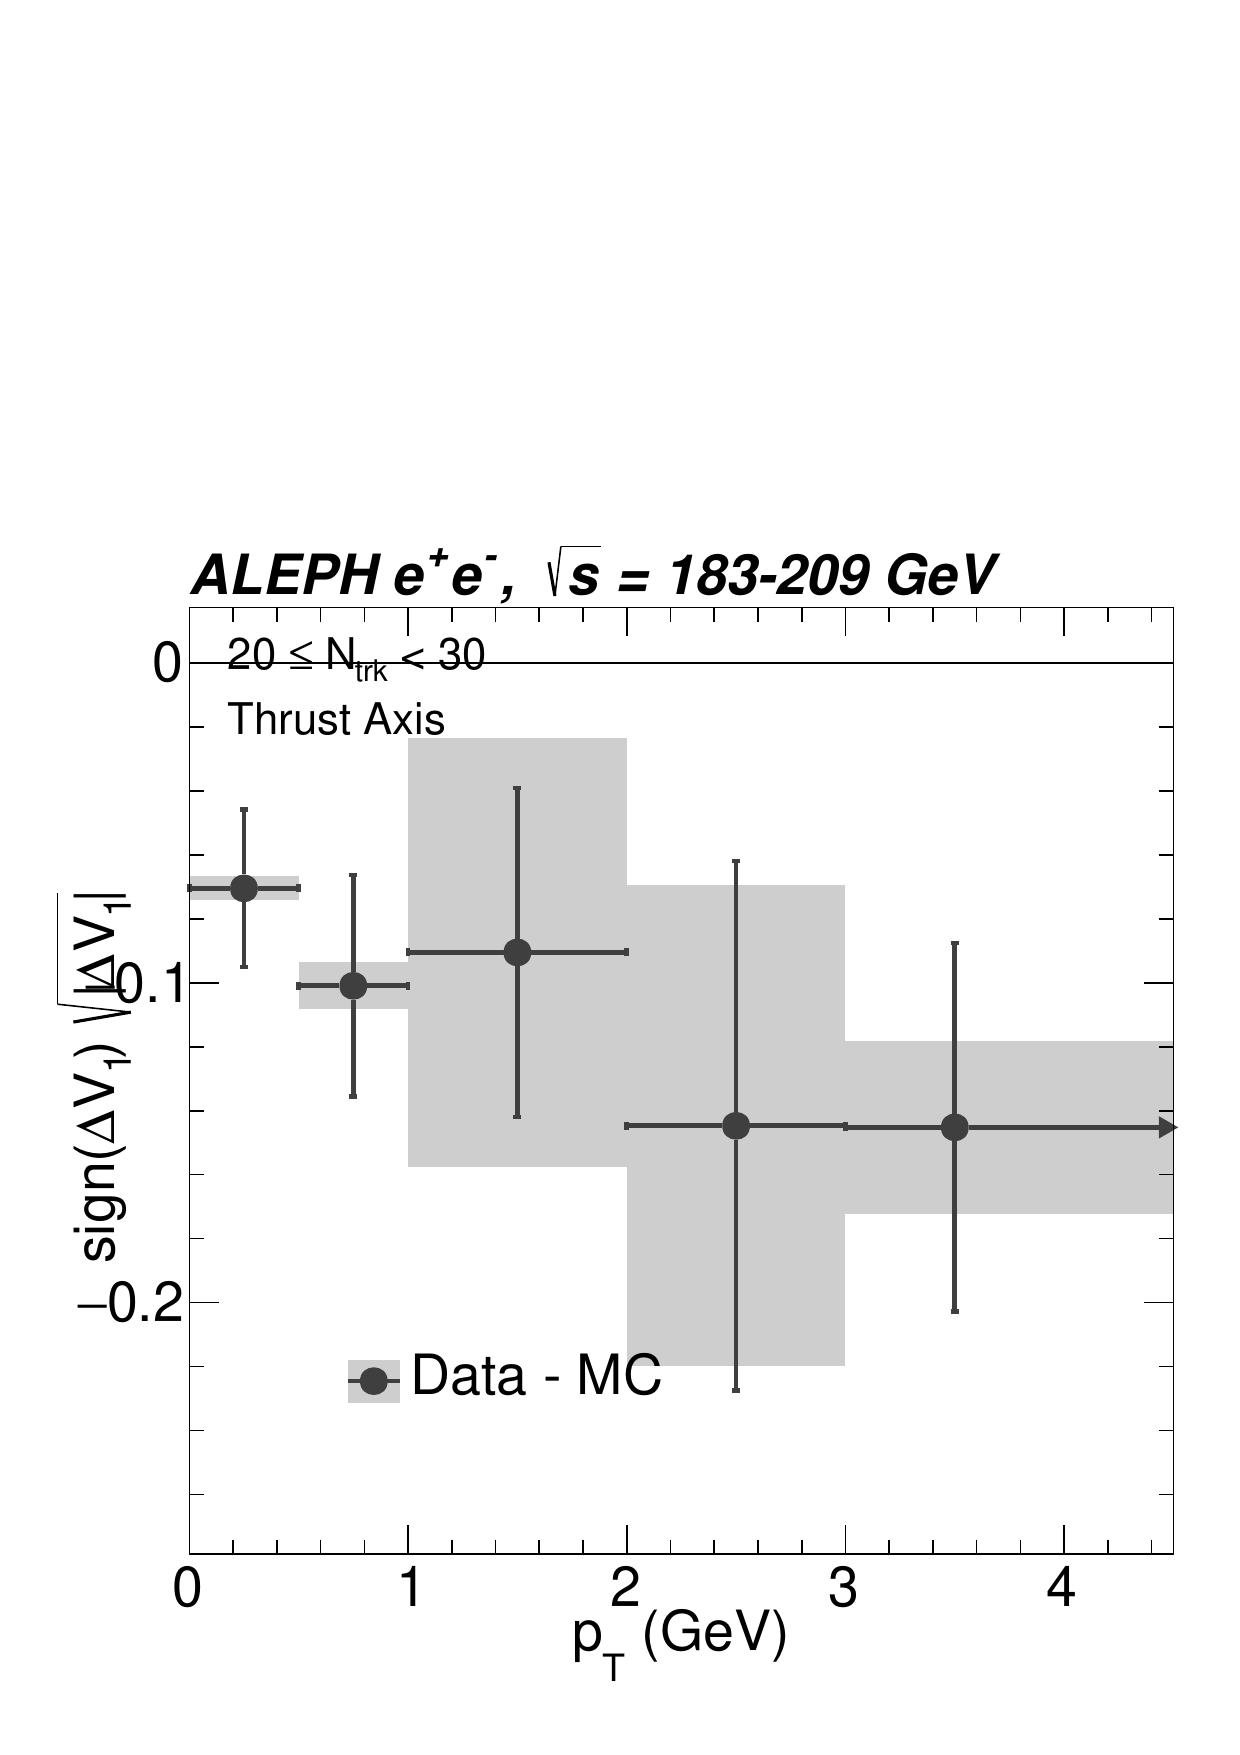}
    \caption{$20 \le {\rm N}_{\rm trk} < 30$}
        %\label{fig:}
    \end{subfigure}
    \begin{subfigure}[b]{0.48\textwidth}
    \includegraphics[width=\textwidth]{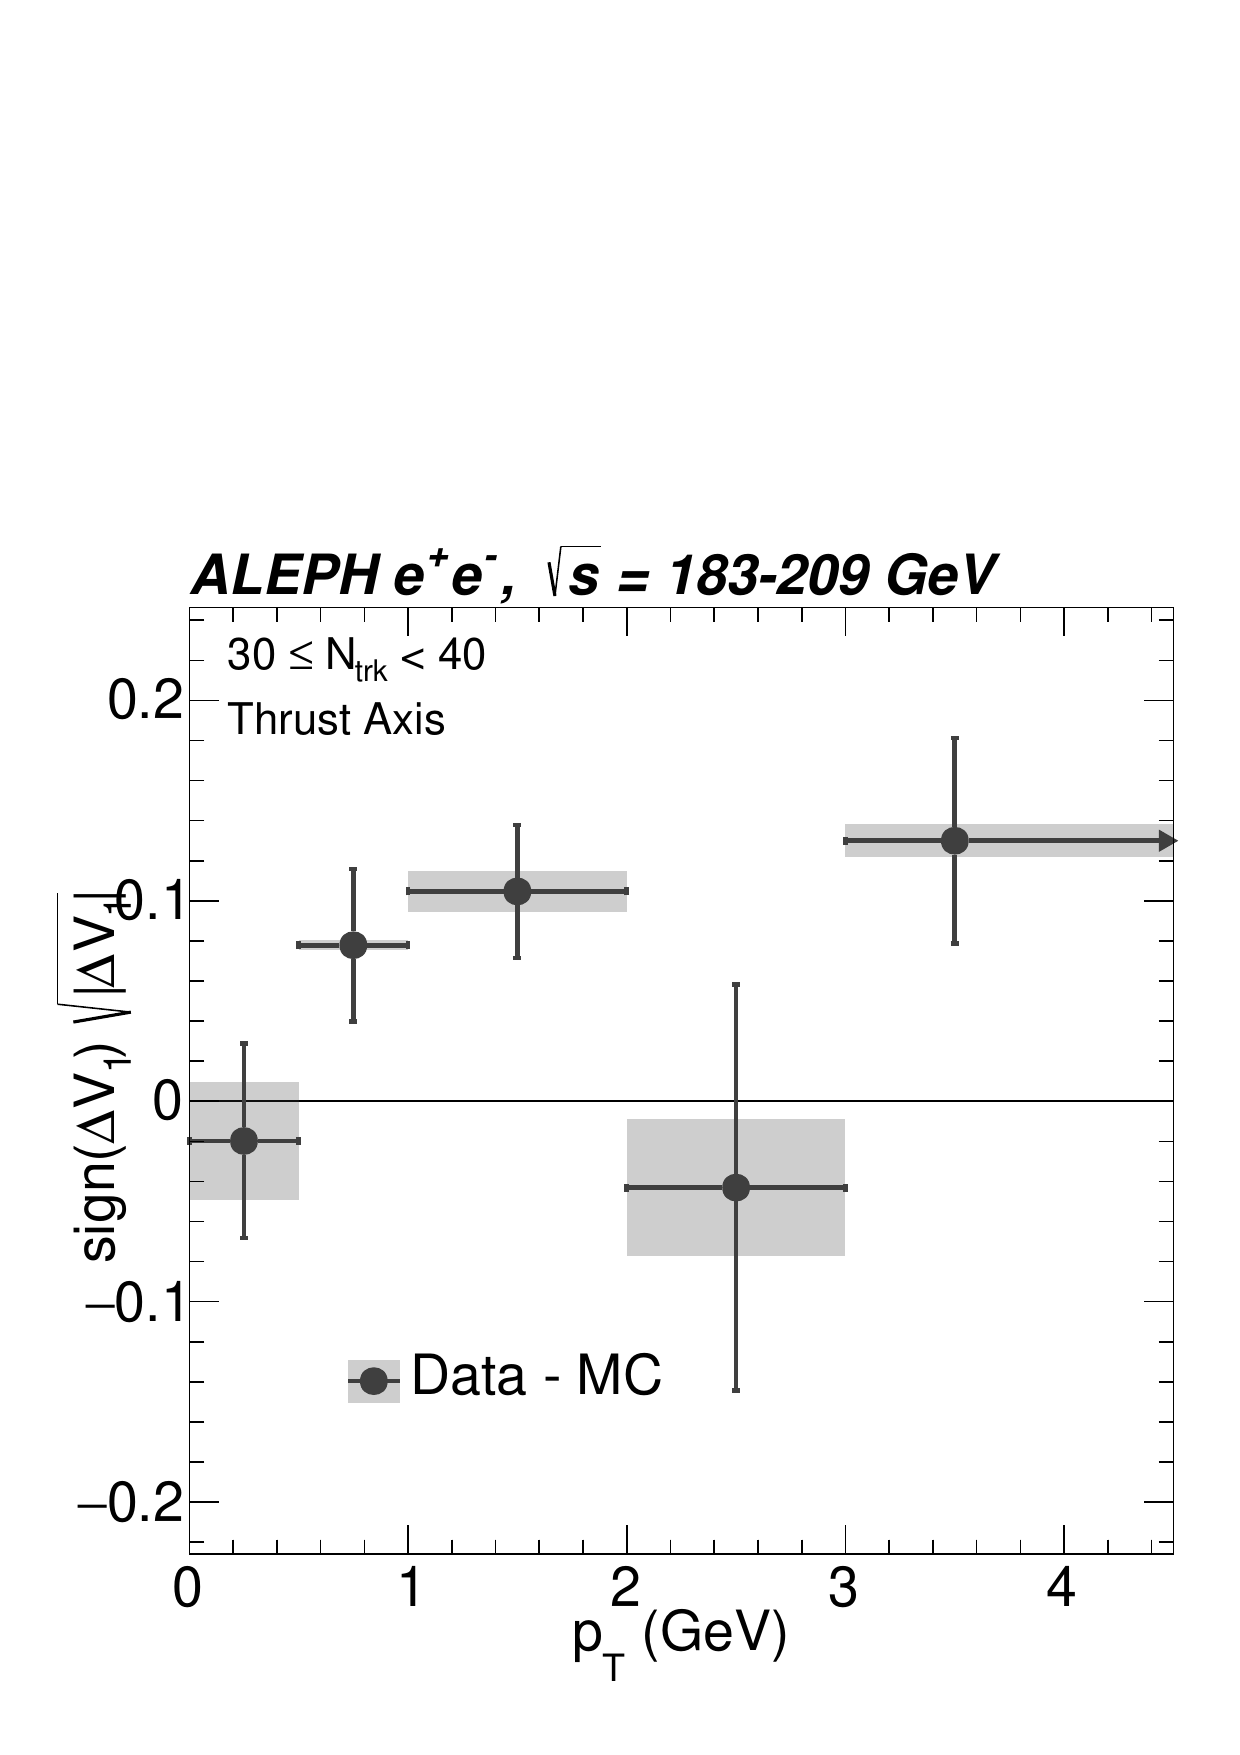}
    \caption{$30 \le {\rm N}_{\rm trk} < 40$}
        %\label{fig:}
    \end{subfigure}
    \begin{subfigure}[b]{0.48\textwidth}
    \includegraphics[width=\textwidth]{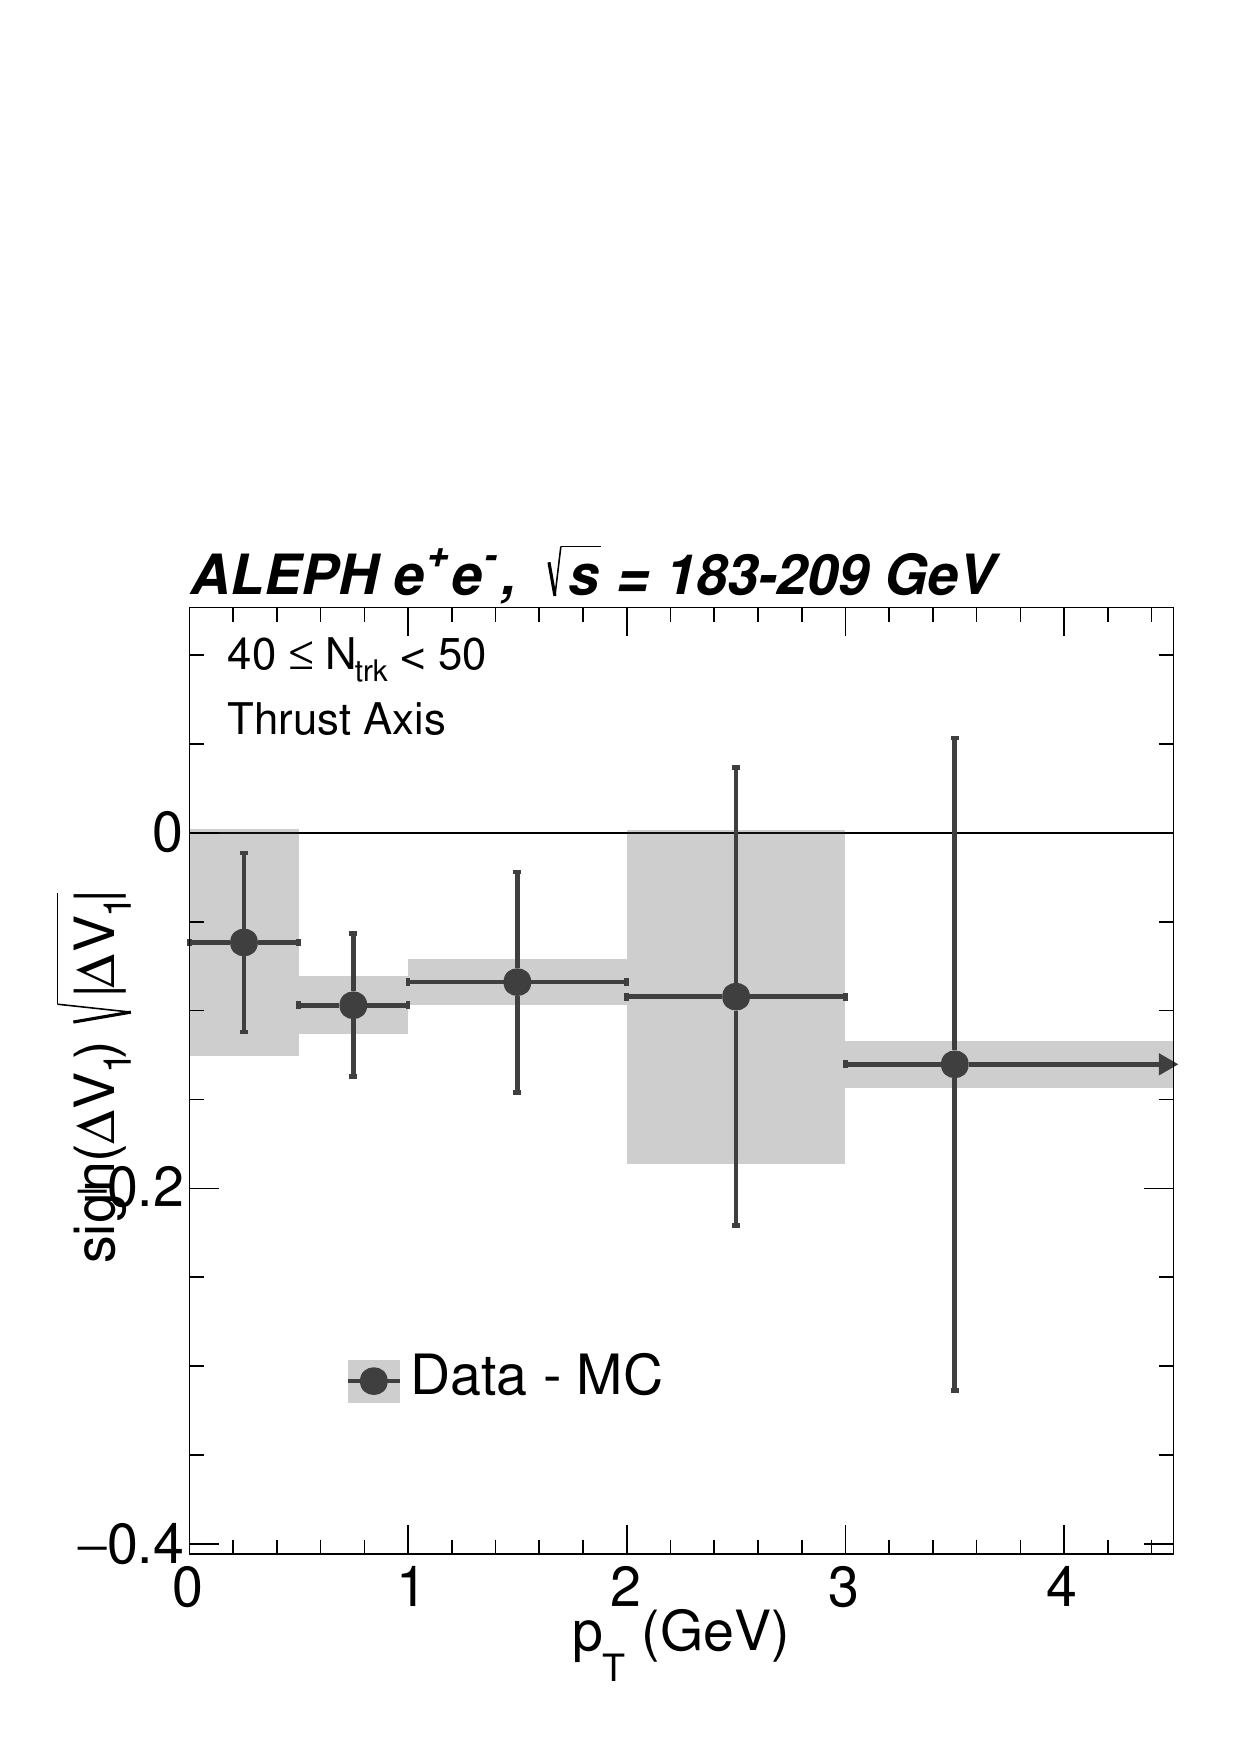}
    \caption{$40 \le {\rm N}_{\rm trk} < 50$}
        %\label{fig:}
    \end{subfigure}
    \begin{subfigure}[b]{0.48\textwidth}
    \includegraphics[width=\textwidth]{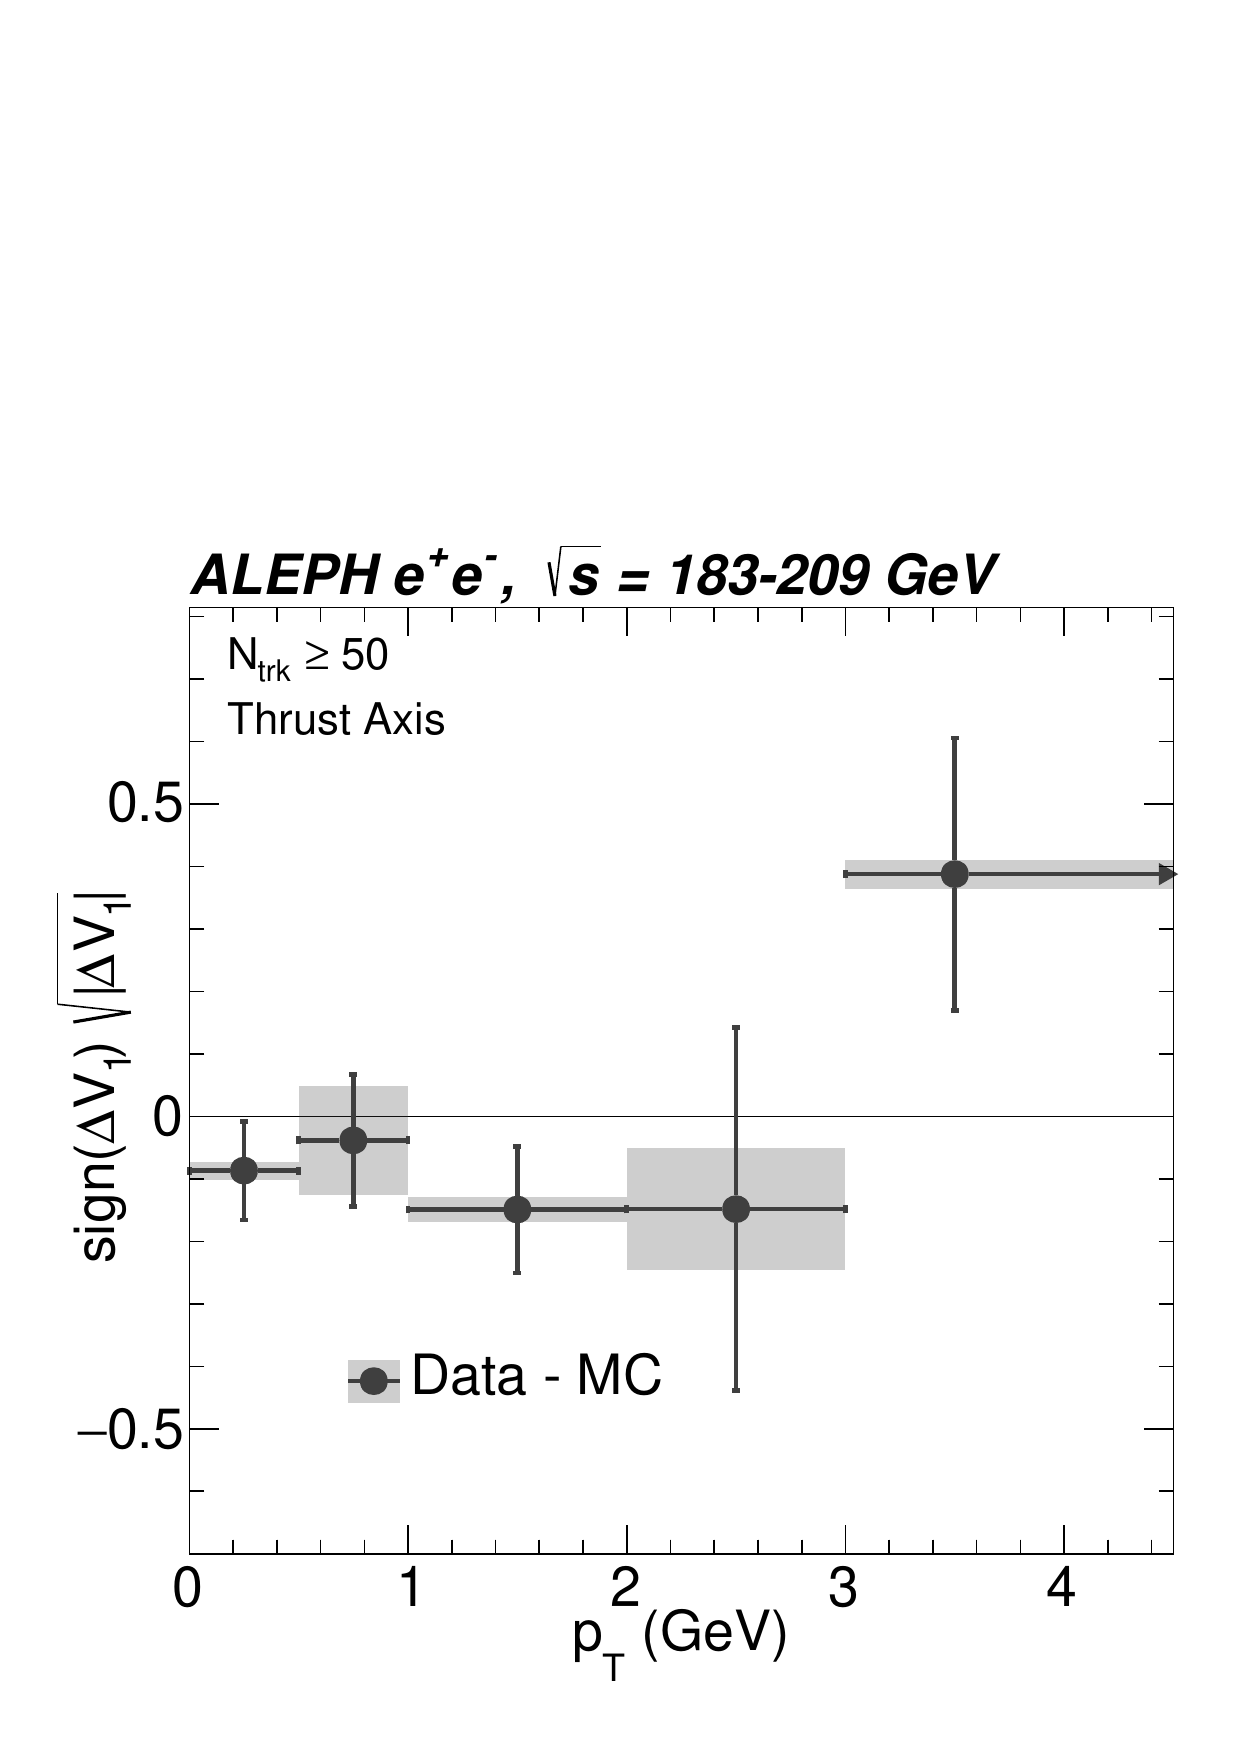}
    \caption{${\rm N}_{\rm trk} \ge 50$}
        %\label{fig:}
    \end{subfigure}
\caption{$\Delta v_{1}$ as a function of the track pairs' $p_{T}$ requirement in different  multiplicity intervals for the thrust axis analysis for LEP-II high-energy sample.}
\label{fig:Dv1VsPt_thrust}
\end{figure}
\clearpage

\subsection*{${\rm sign}(\Delta V_3) \sqrt{\Delta V_3}$}
%%%%%%%%%%%%%%%%%%%% Beam axis: Delta v3 vs pt
\begin{figure}[ht]
\centering
    \begin{subfigure}[b]{0.48\textwidth}
    \includegraphics[width=\textwidth]{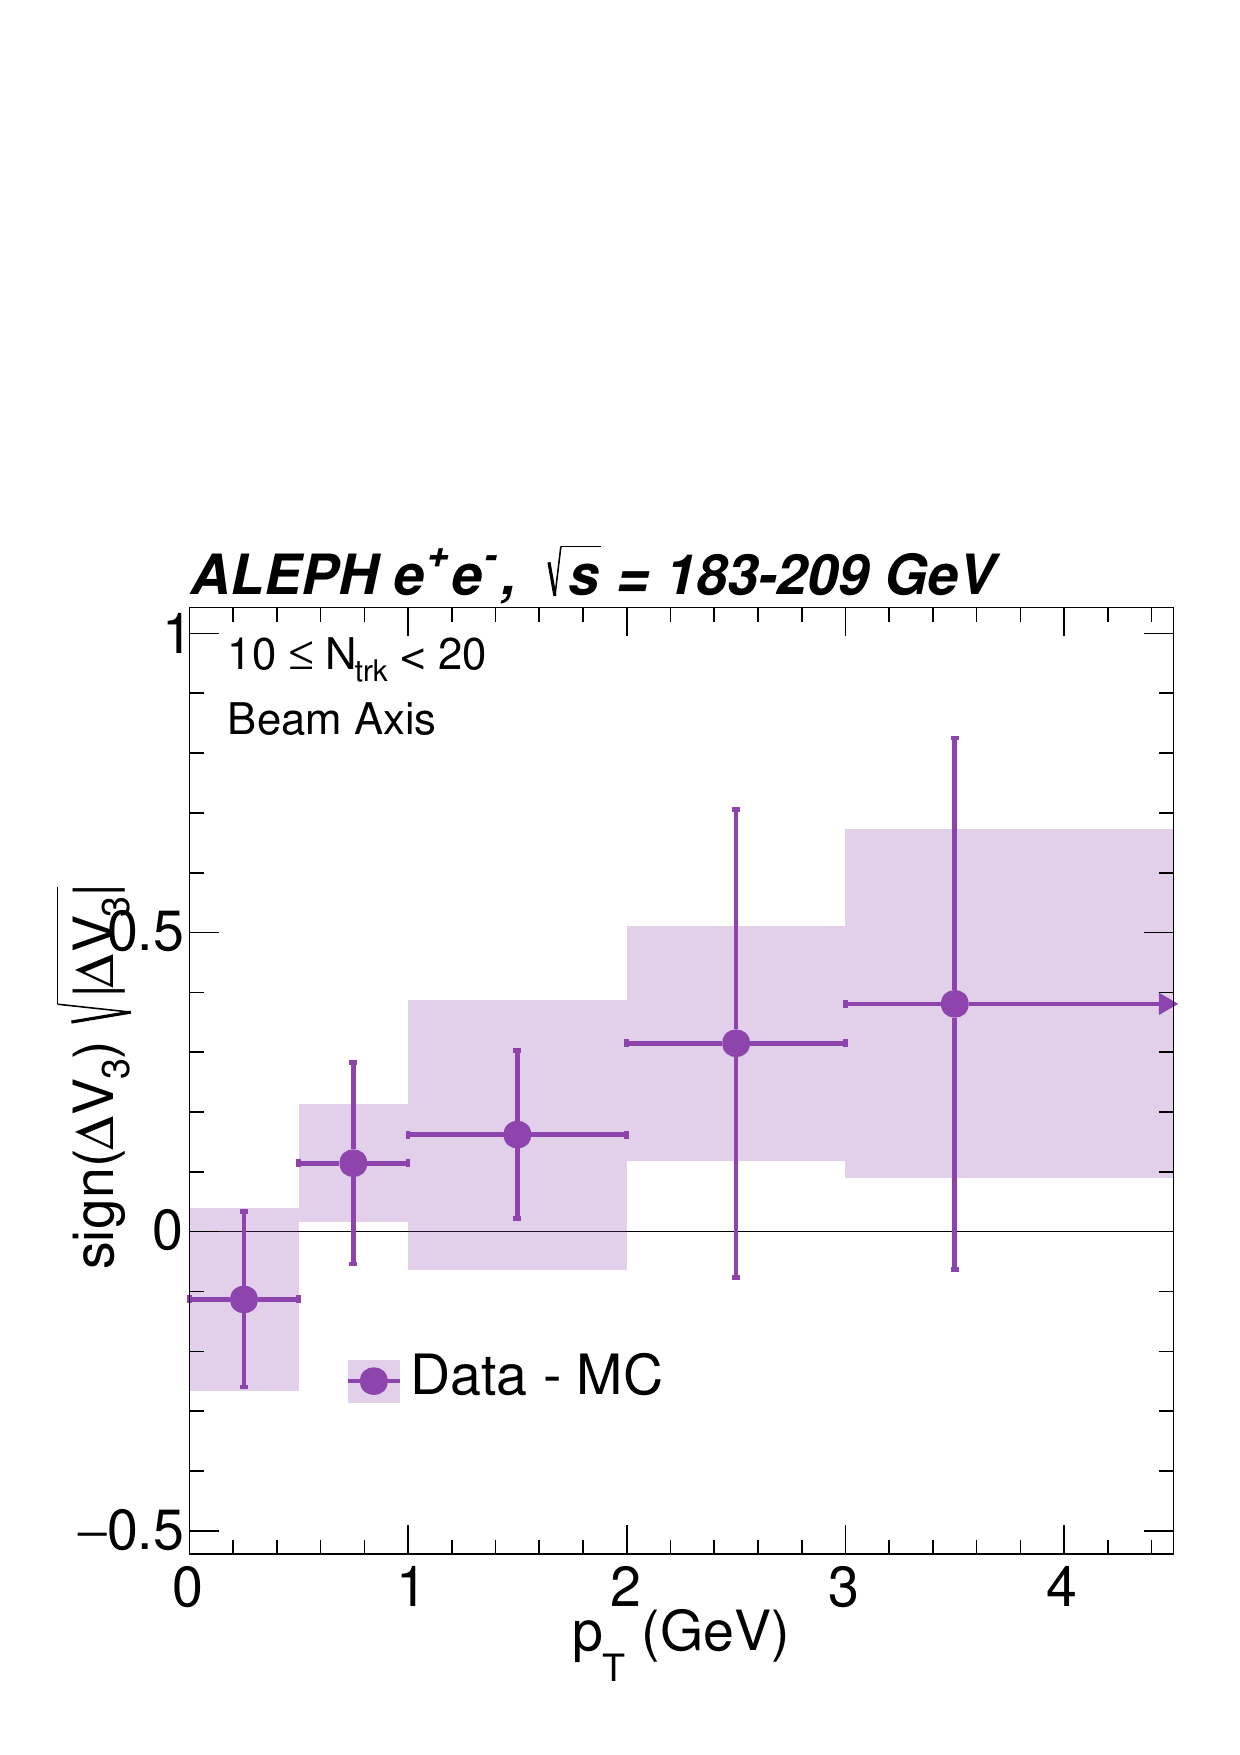}
    \caption{$10 \le {\rm N}_{\rm trk} < 20$}
        %\label{fig:}
    \end{subfigure}
    \begin{subfigure}[b]{0.48\textwidth}
    \includegraphics[width=\textwidth]{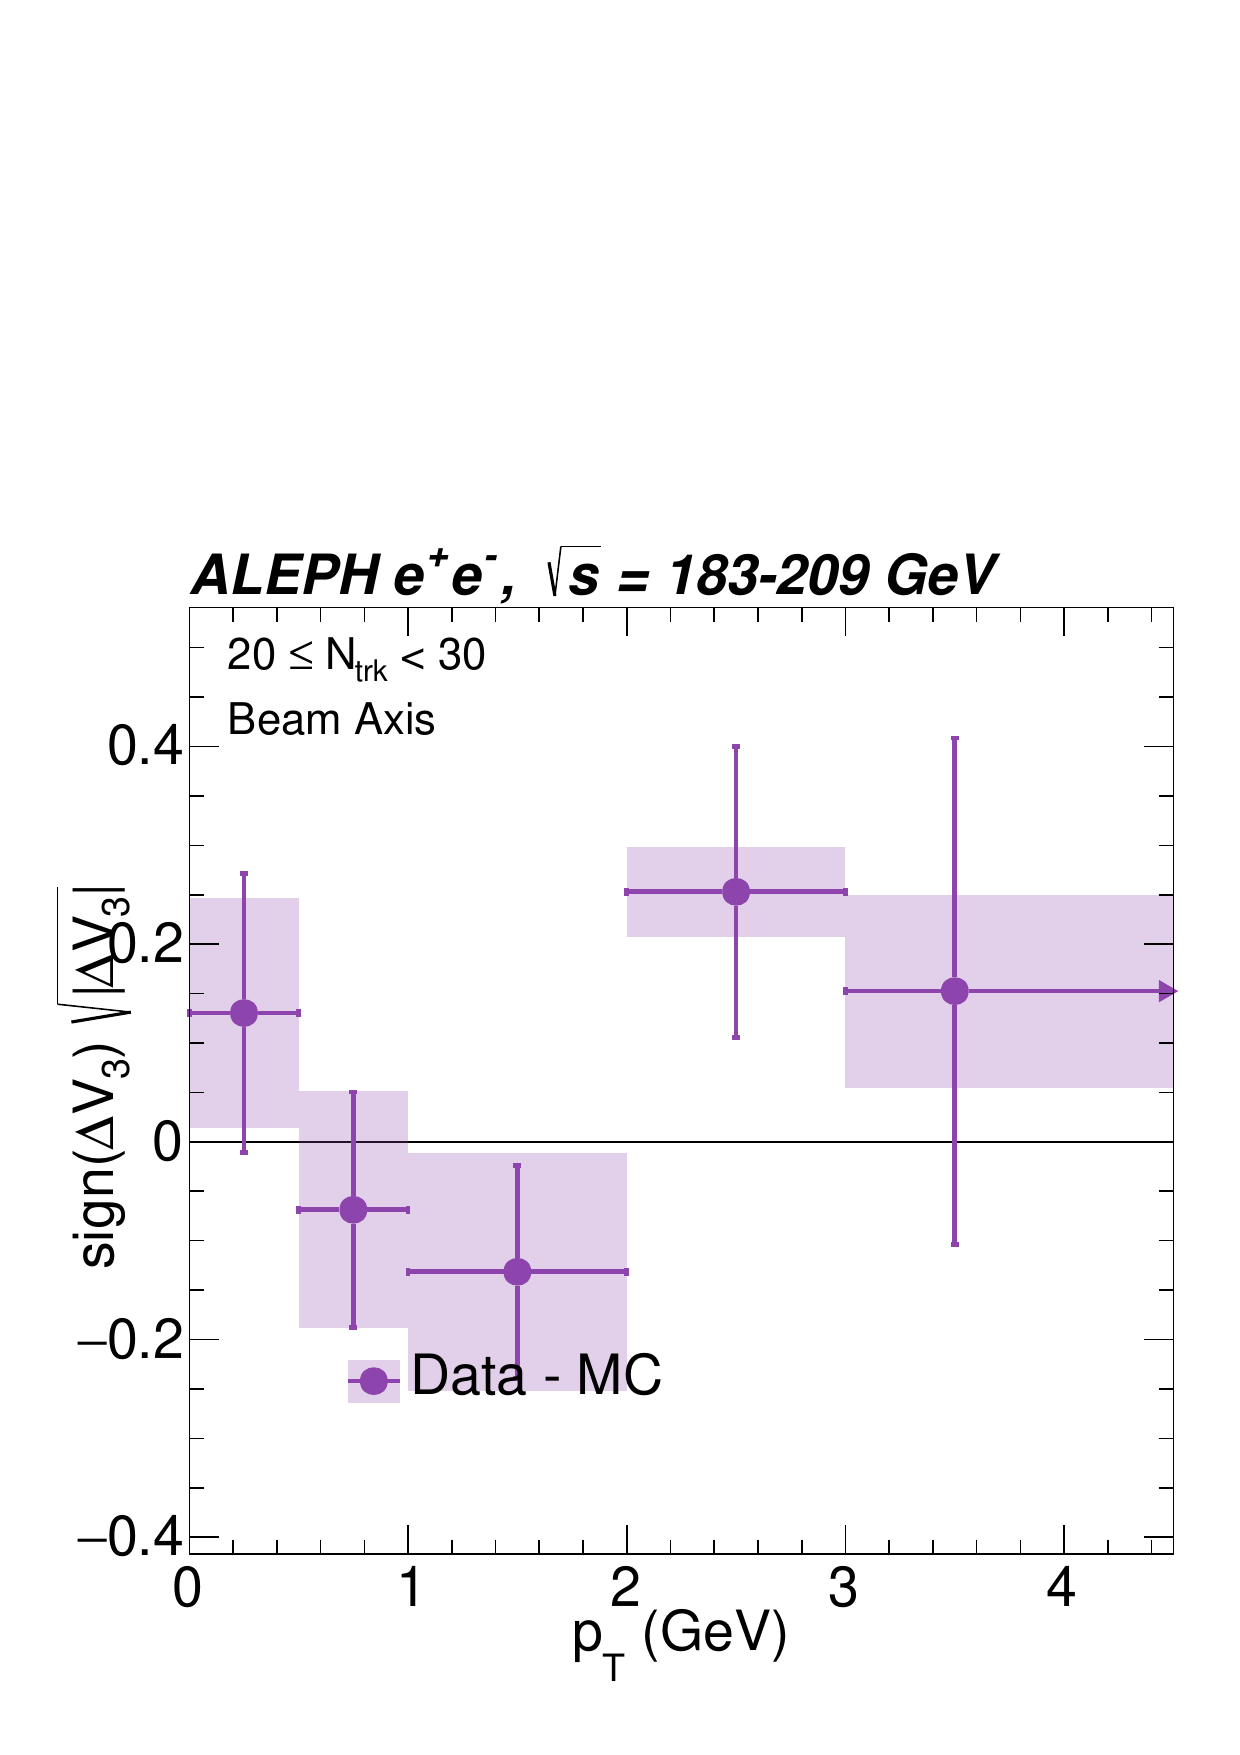}
    \caption{$20 \le {\rm N}_{\rm trk} < 30$}
        %\label{fig:}
    \end{subfigure}
    \begin{subfigure}[b]{0.48\textwidth}
    \includegraphics[width=\textwidth]{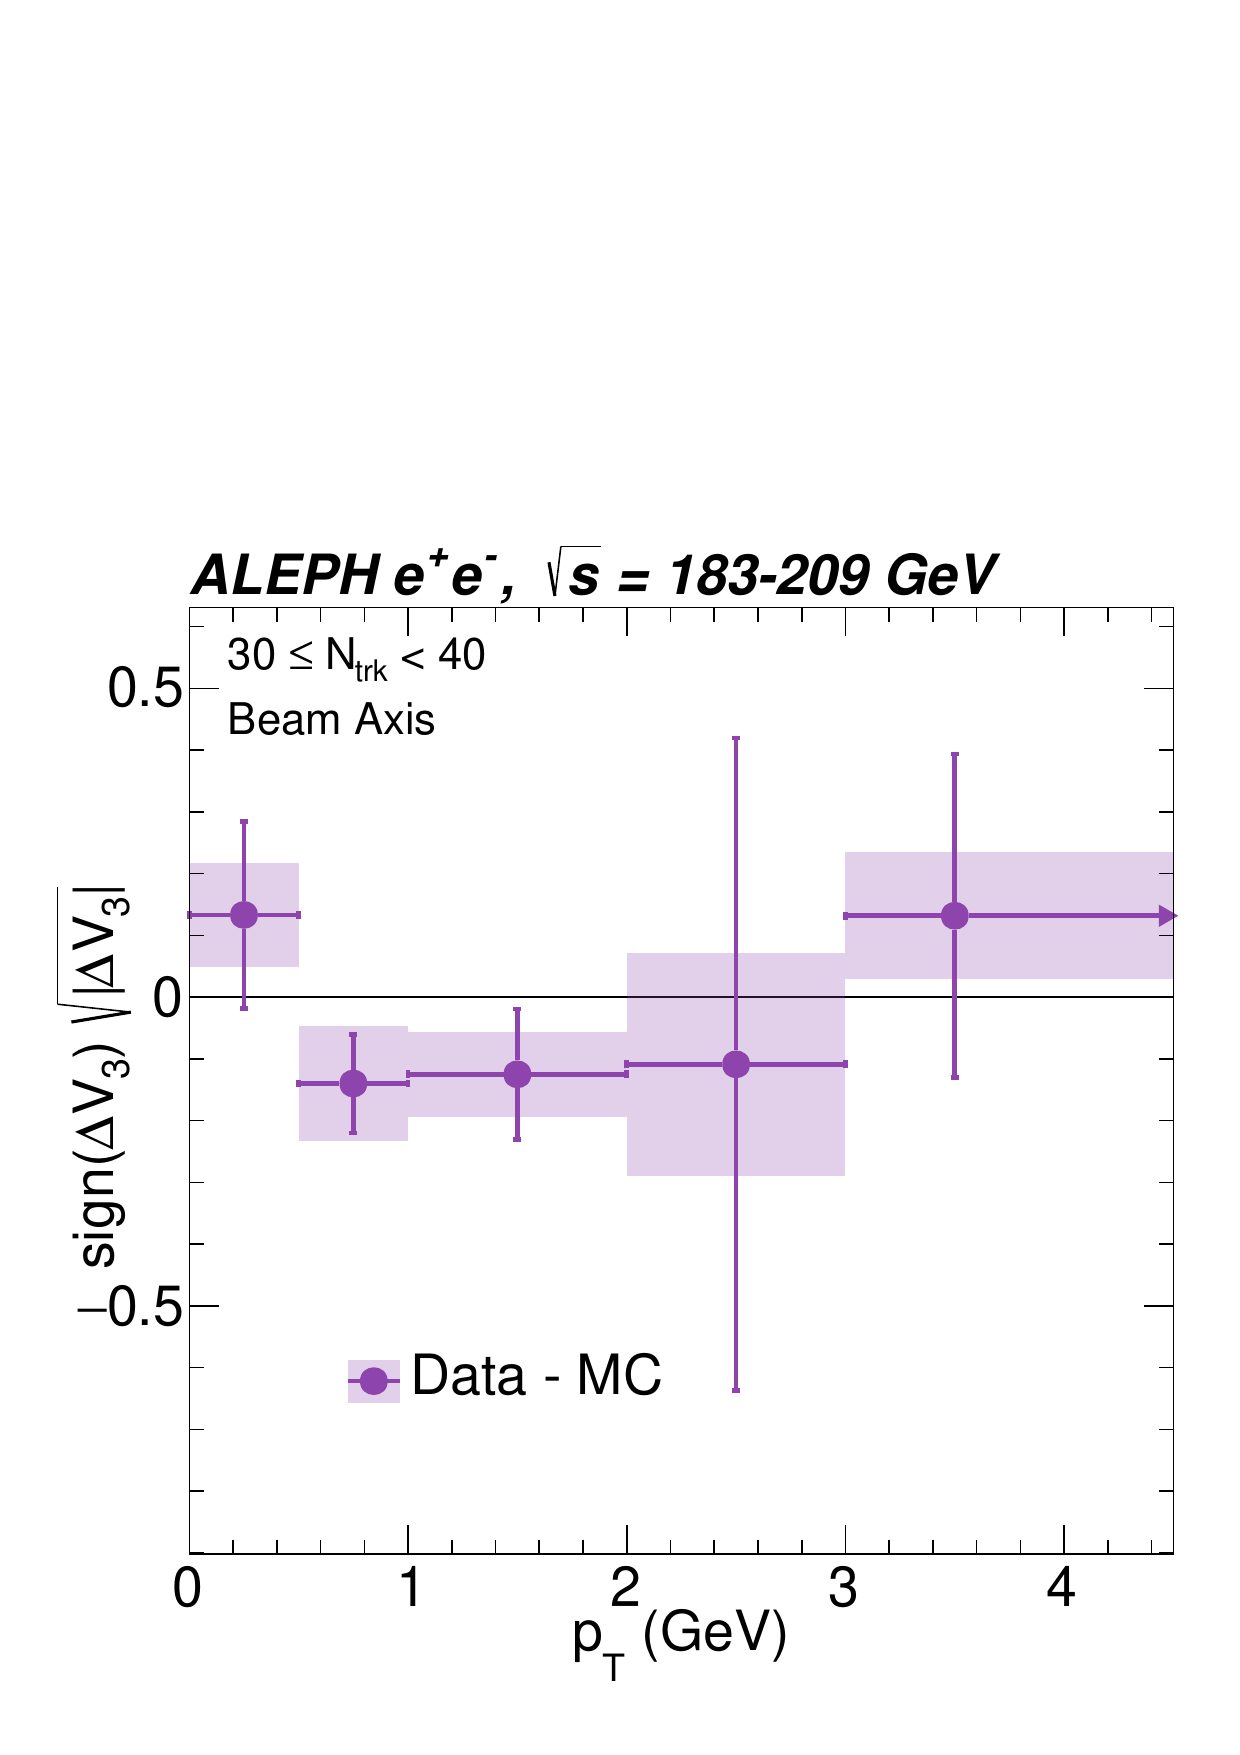}
    \caption{$30 \le {\rm N}_{\rm trk} < 40$}
        %\label{fig:}
    \end{subfigure}
    \begin{subfigure}[b]{0.48\textwidth}
    \includegraphics[width=\textwidth]{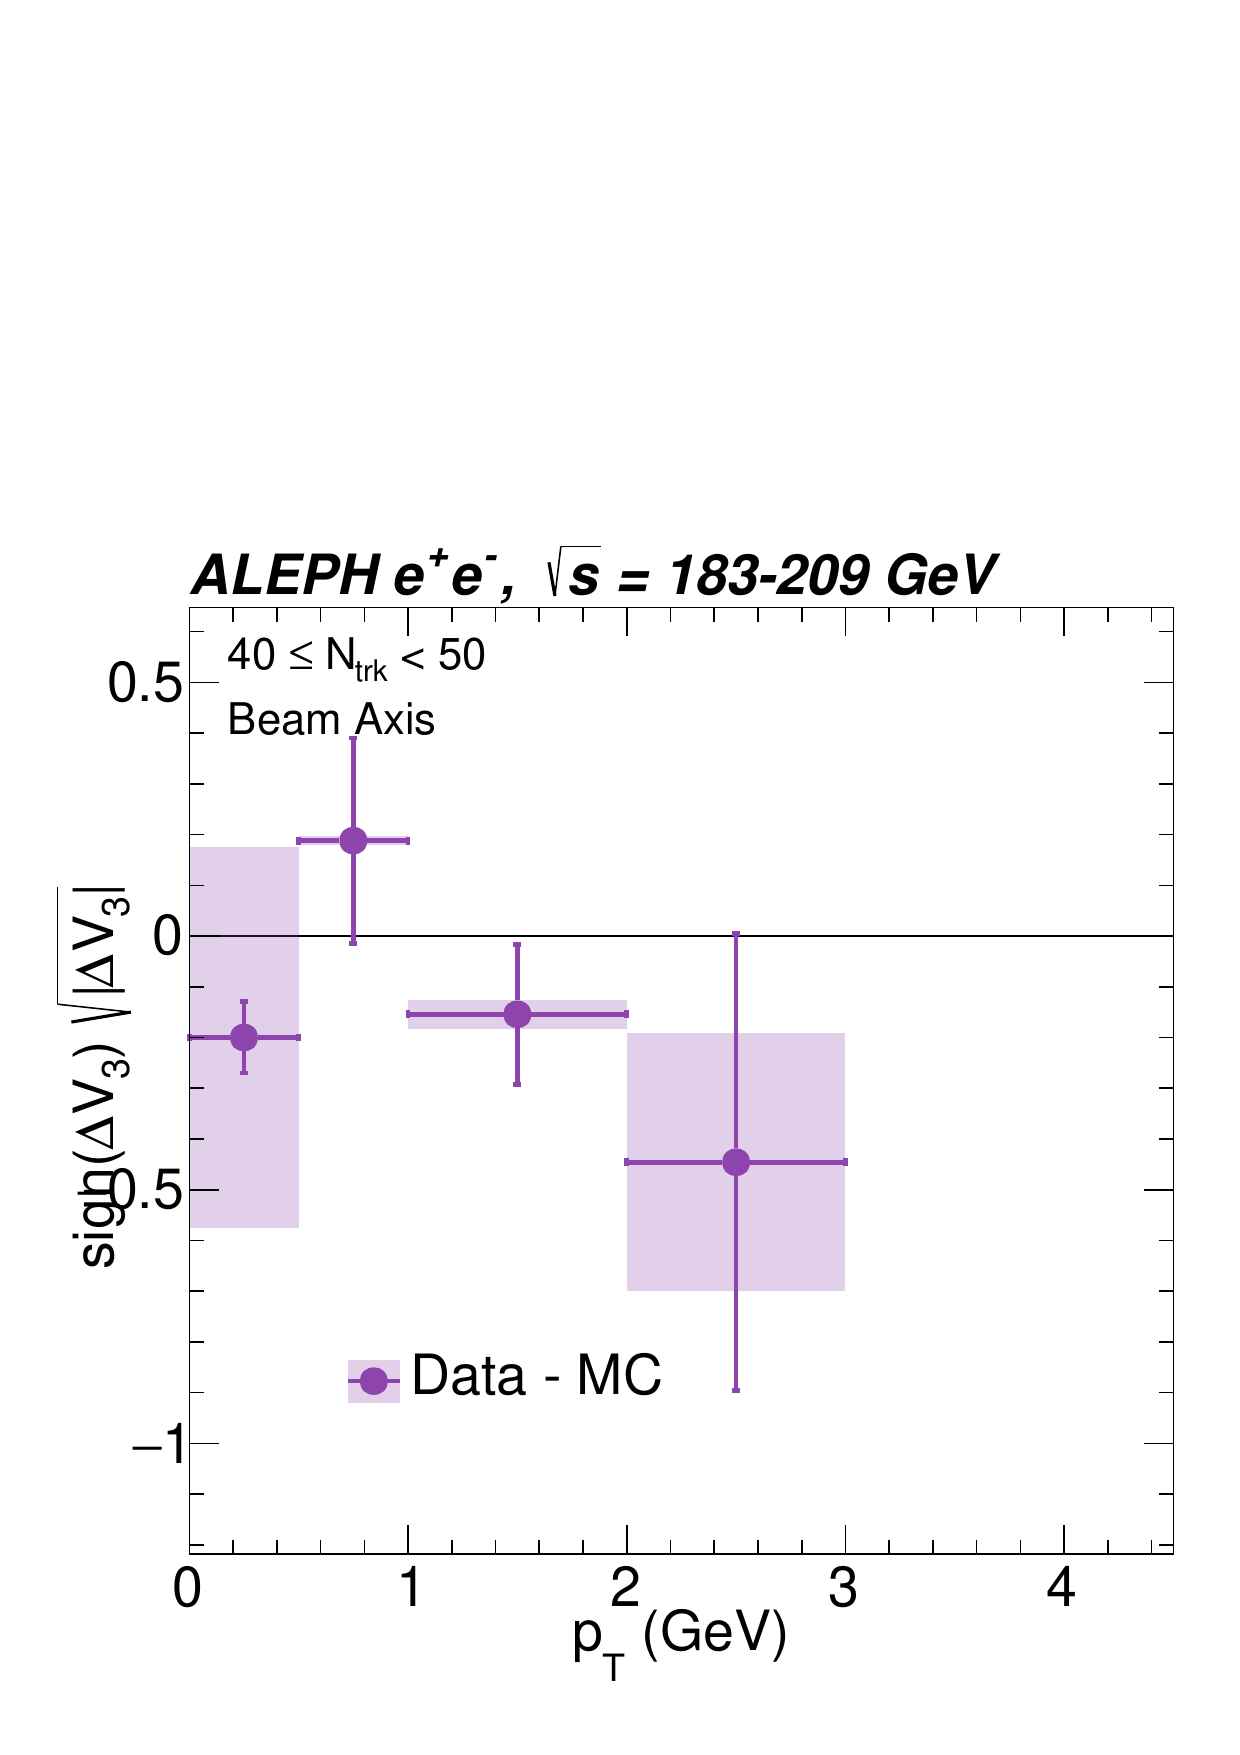}
    \caption{$40 \le {\rm N}_{\rm trk} < 50$}
        %\label{fig:}
    \end{subfigure}
    \begin{subfigure}[b]{0.48\textwidth}
    \includegraphics[width=\textwidth]{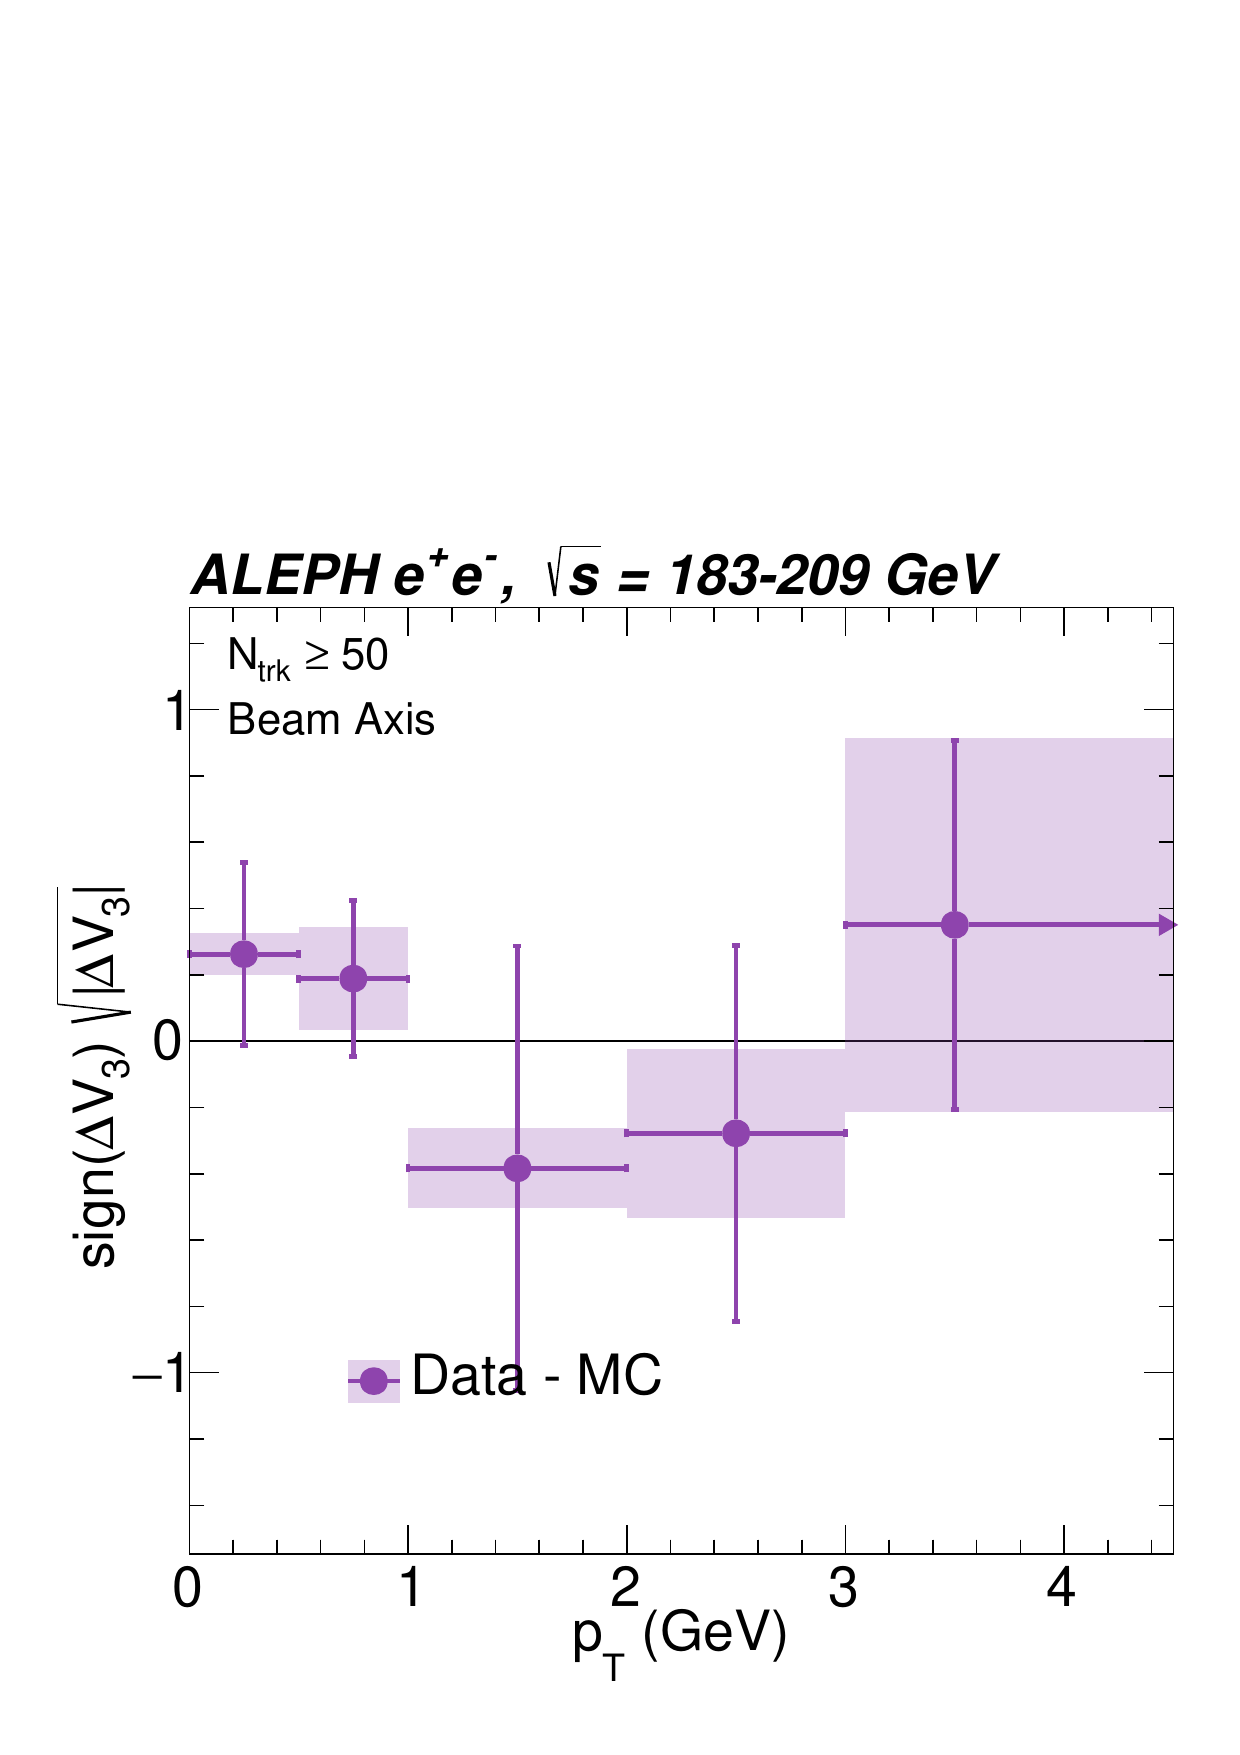}
    \caption{${\rm N}_{\rm trk} \ge 50$}
        %\label{fig:}
    \end{subfigure}
\caption{$\Delta v_{3}$ as a function of the track pairs' $p_{T}$ requirement in different  multiplicity intervals for the beam axis analysis for LEP-II high-energy sample.}
\label{fig:Dv3VsPt_beam}
\end{figure}

%%%%%%%%%%%%%%%%%%%% Thrust axis: Delta v3 vs pt
\begin{figure}[ht]
\centering
    \begin{subfigure}[b]{0.48\textwidth}
    \includegraphics[width=\textwidth]{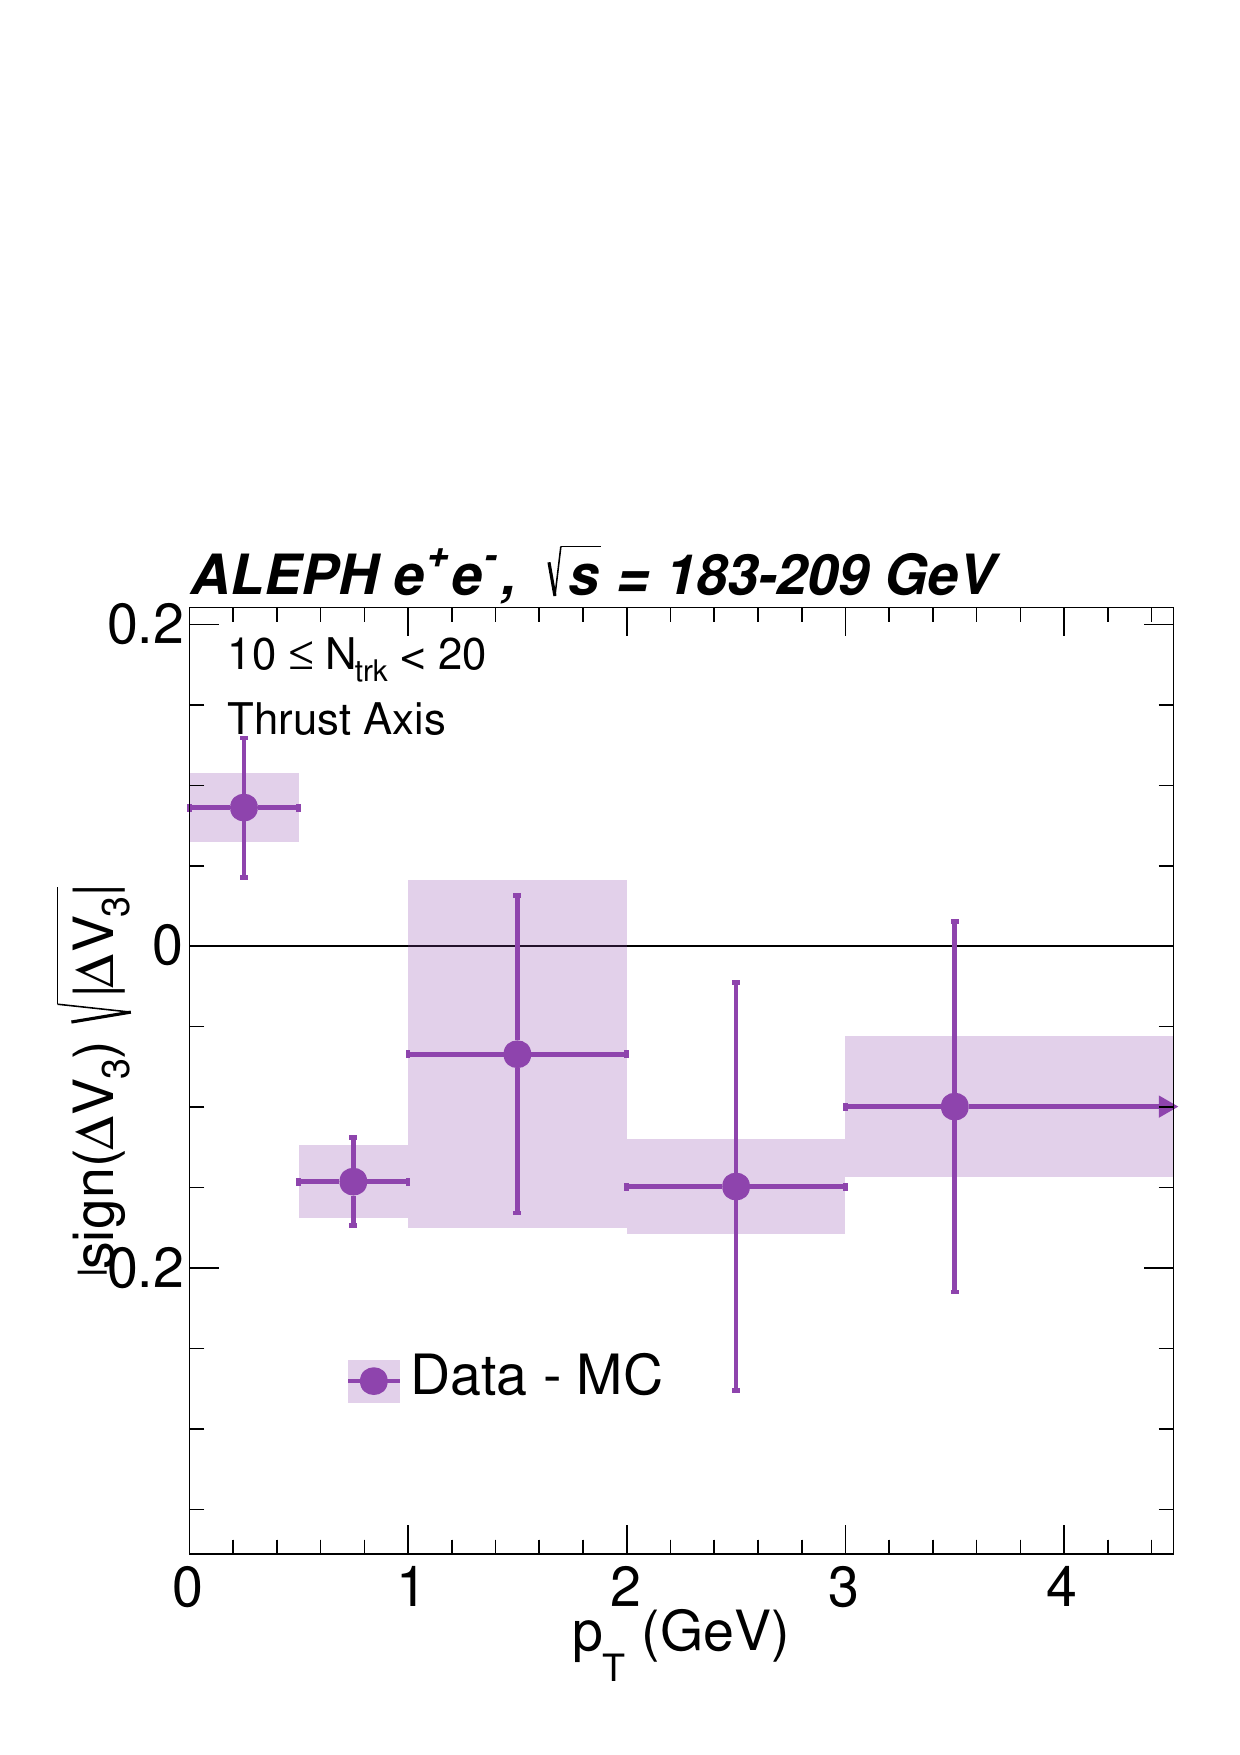}
    \caption{$10 \le {\rm N}_{\rm trk} < 20$}
        %\label{fig:}
    \end{subfigure}
    \begin{subfigure}[b]{0.48\textwidth}
    \includegraphics[width=\textwidth]{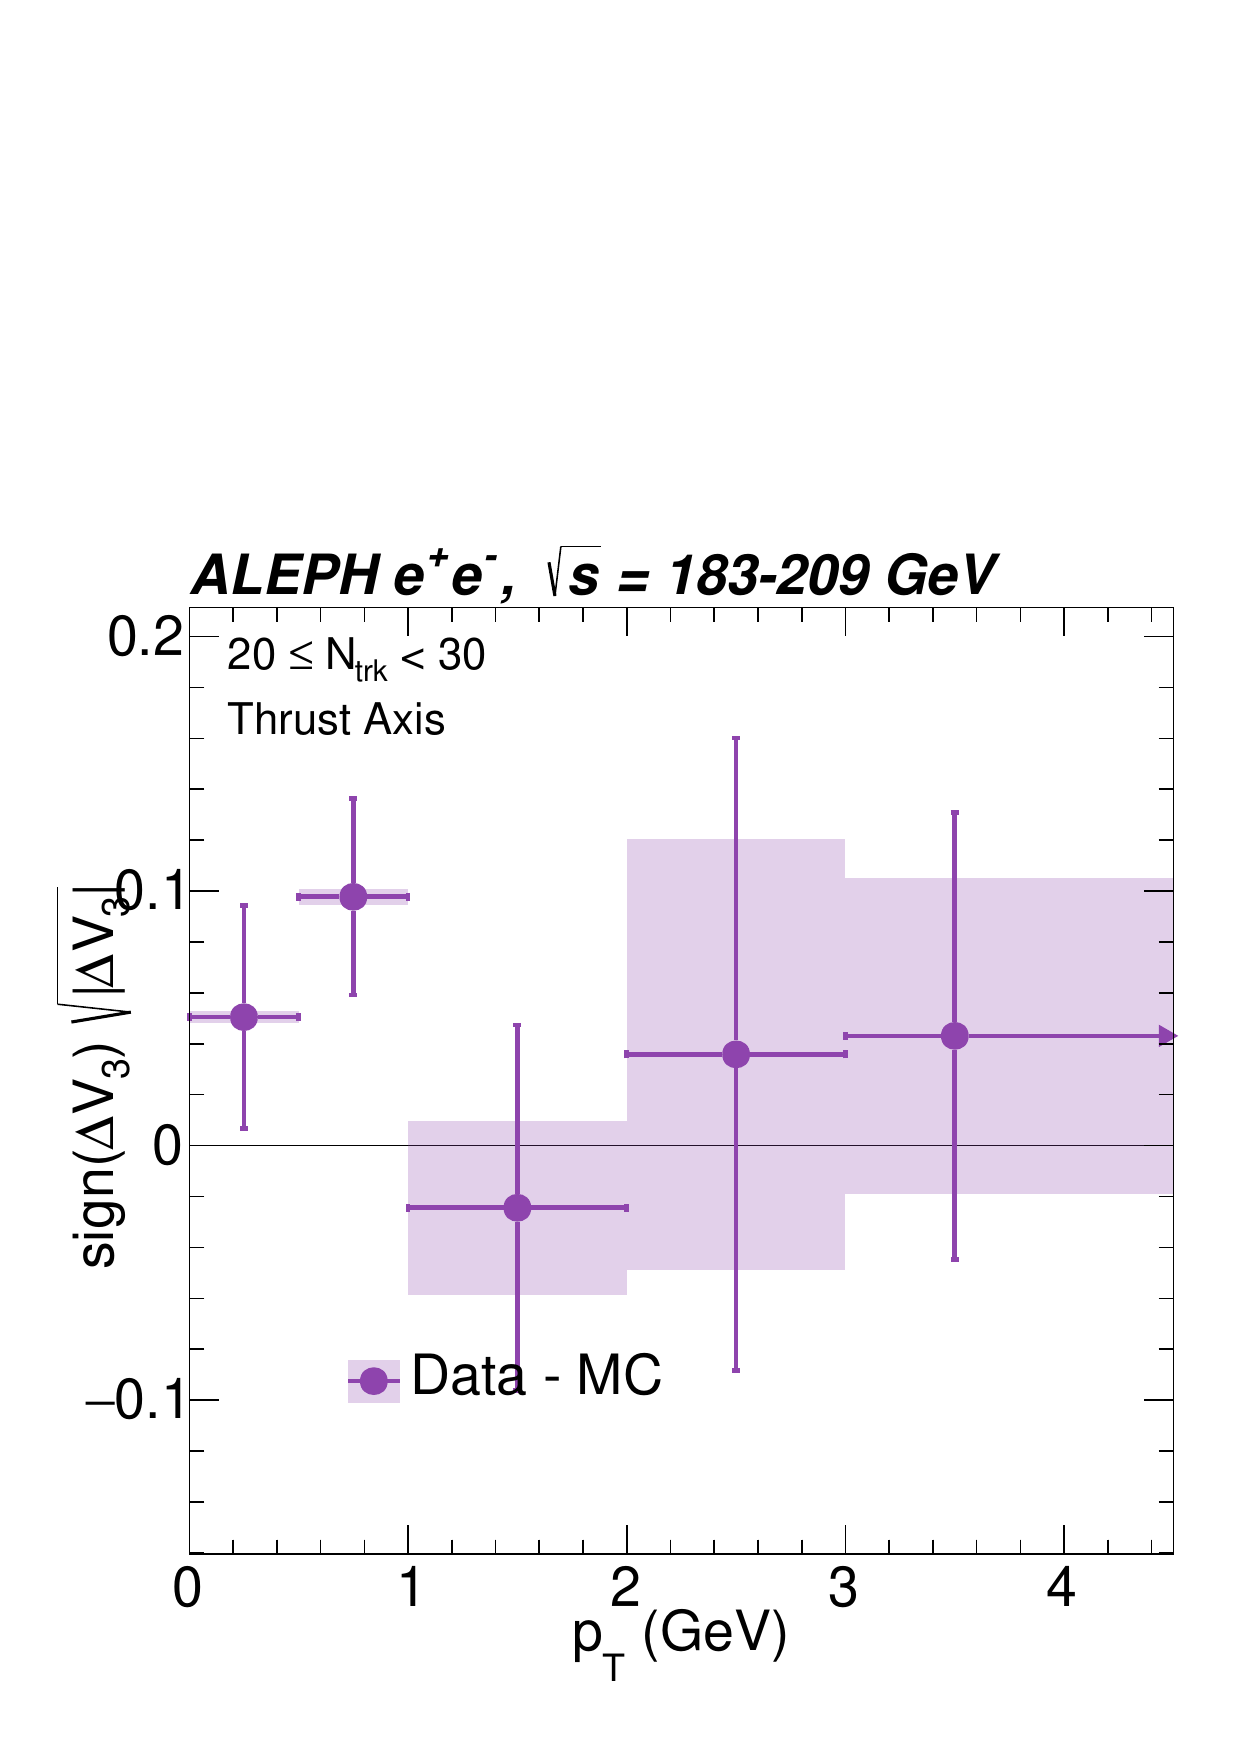}
    \caption{$20 \le {\rm N}_{\rm trk} < 30$}
        %\label{fig:}
    \end{subfigure}
    \begin{subfigure}[b]{0.48\textwidth}
    \includegraphics[width=\textwidth]{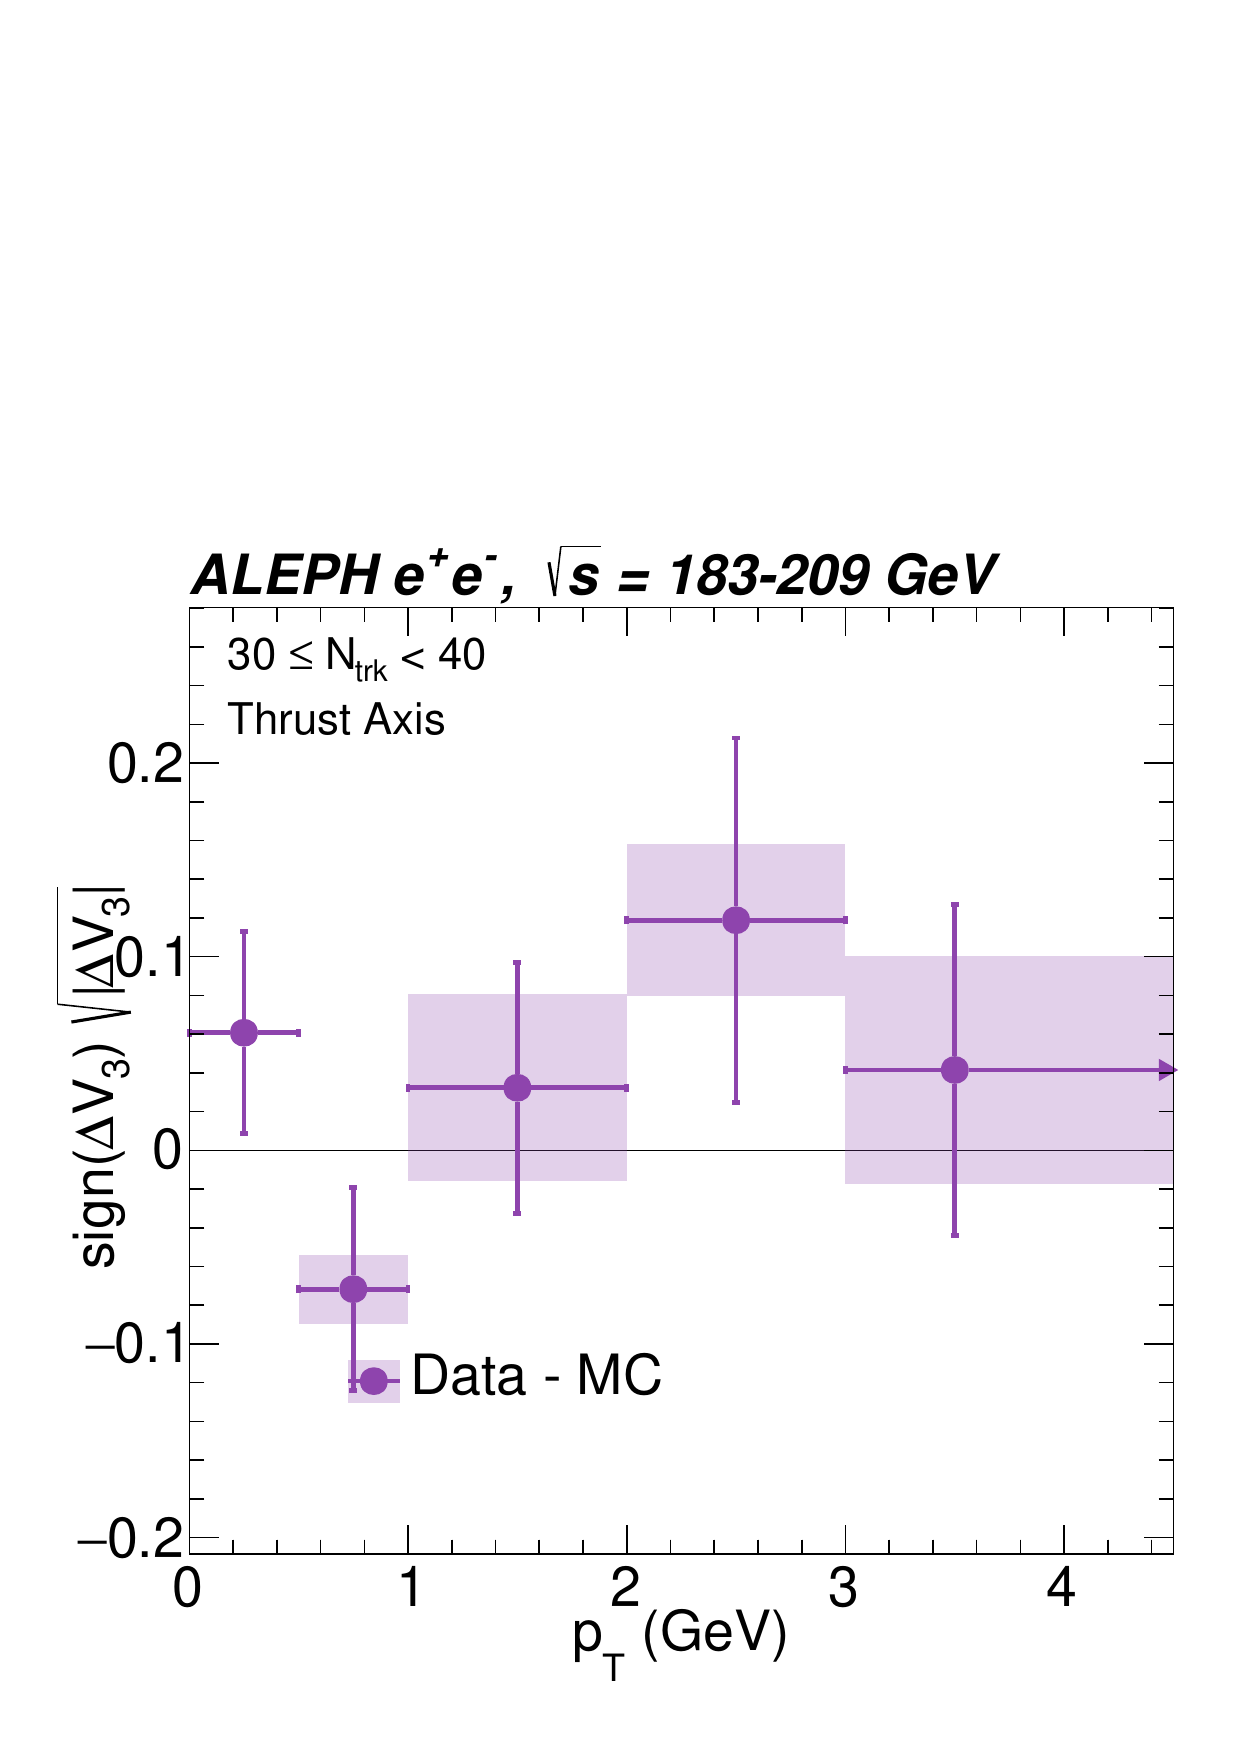}
    \caption{$30 \le {\rm N}_{\rm trk} < 40$}
        %\label{fig:}
    \end{subfigure}
    \begin{subfigure}[b]{0.48\textwidth}
    \includegraphics[width=\textwidth]{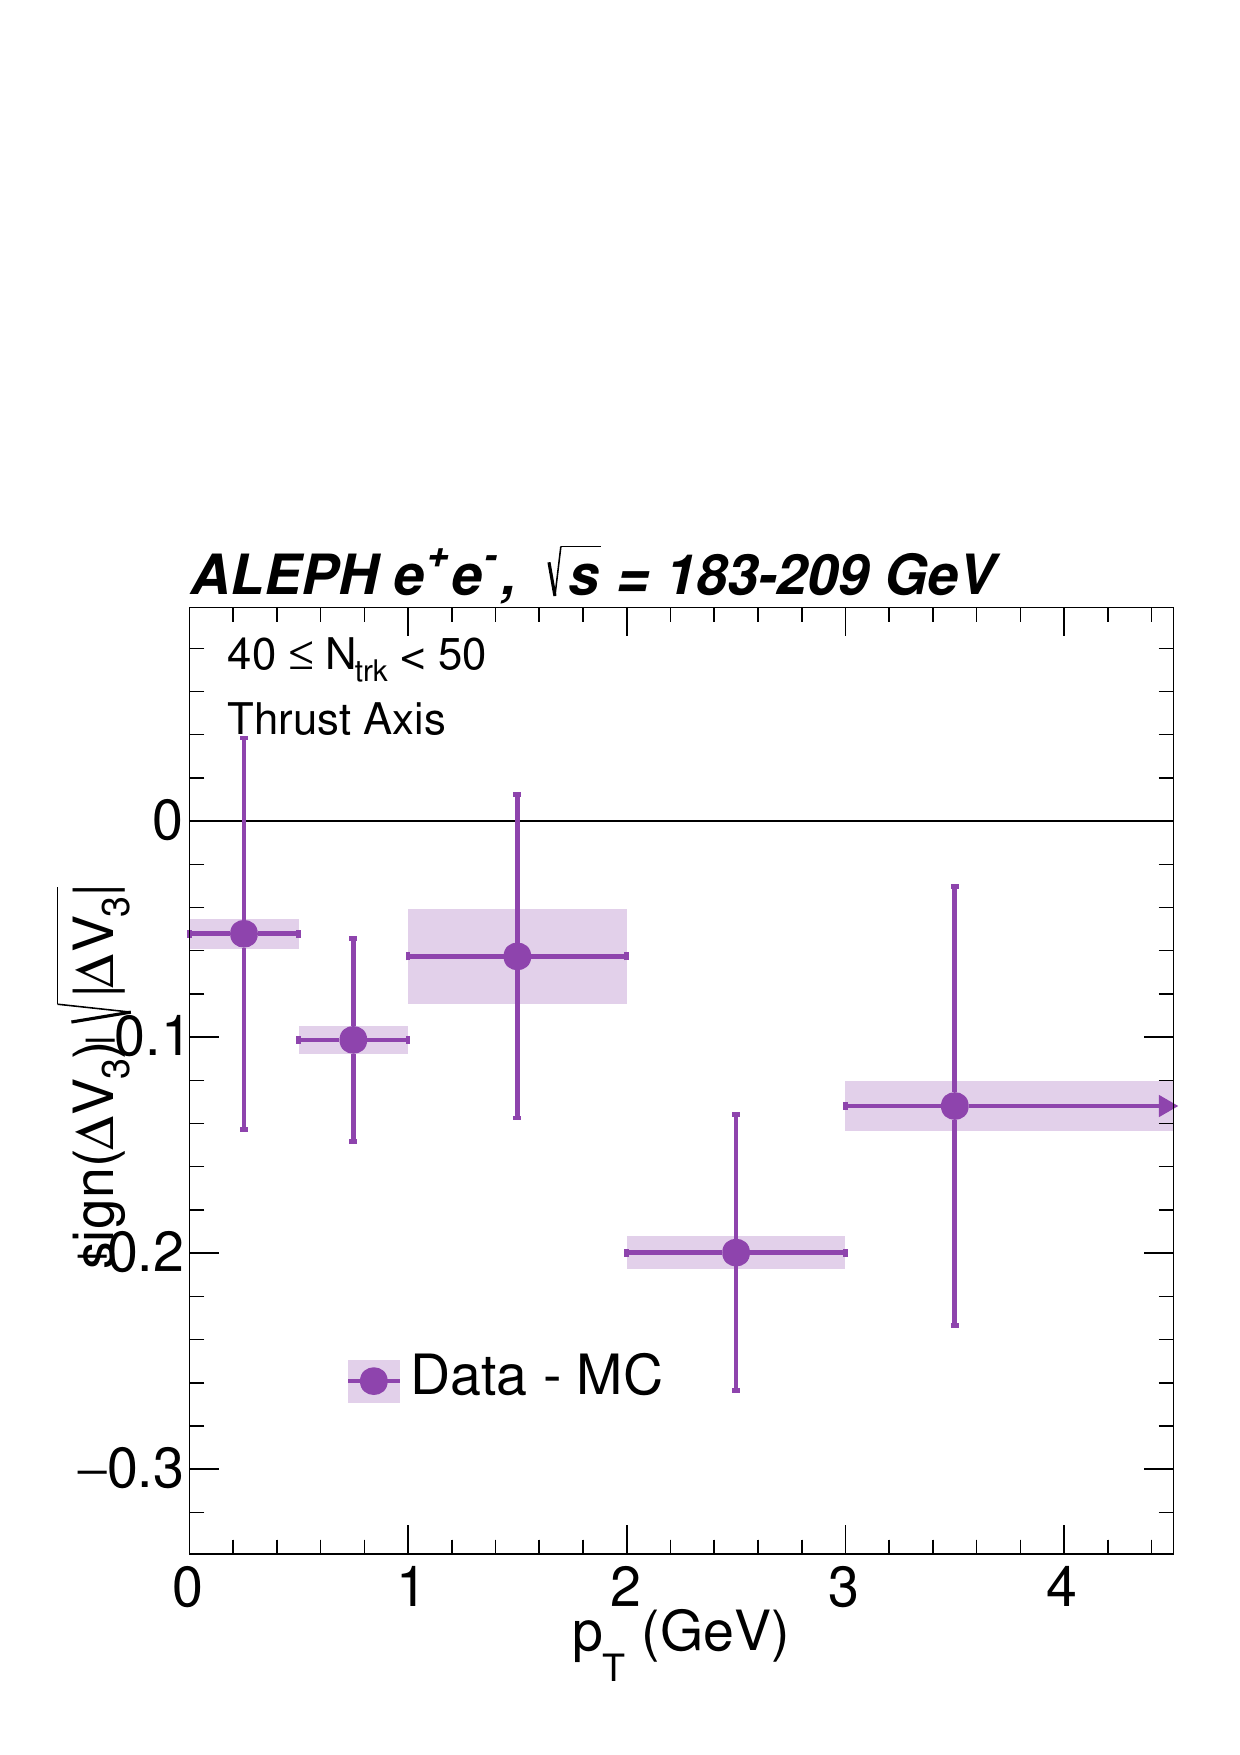}
    \caption{$40 \le {\rm N}_{\rm trk} < 50$}
        %\label{fig:}
    \end{subfigure}
    \begin{subfigure}[b]{0.48\textwidth}
    \includegraphics[width=\textwidth]{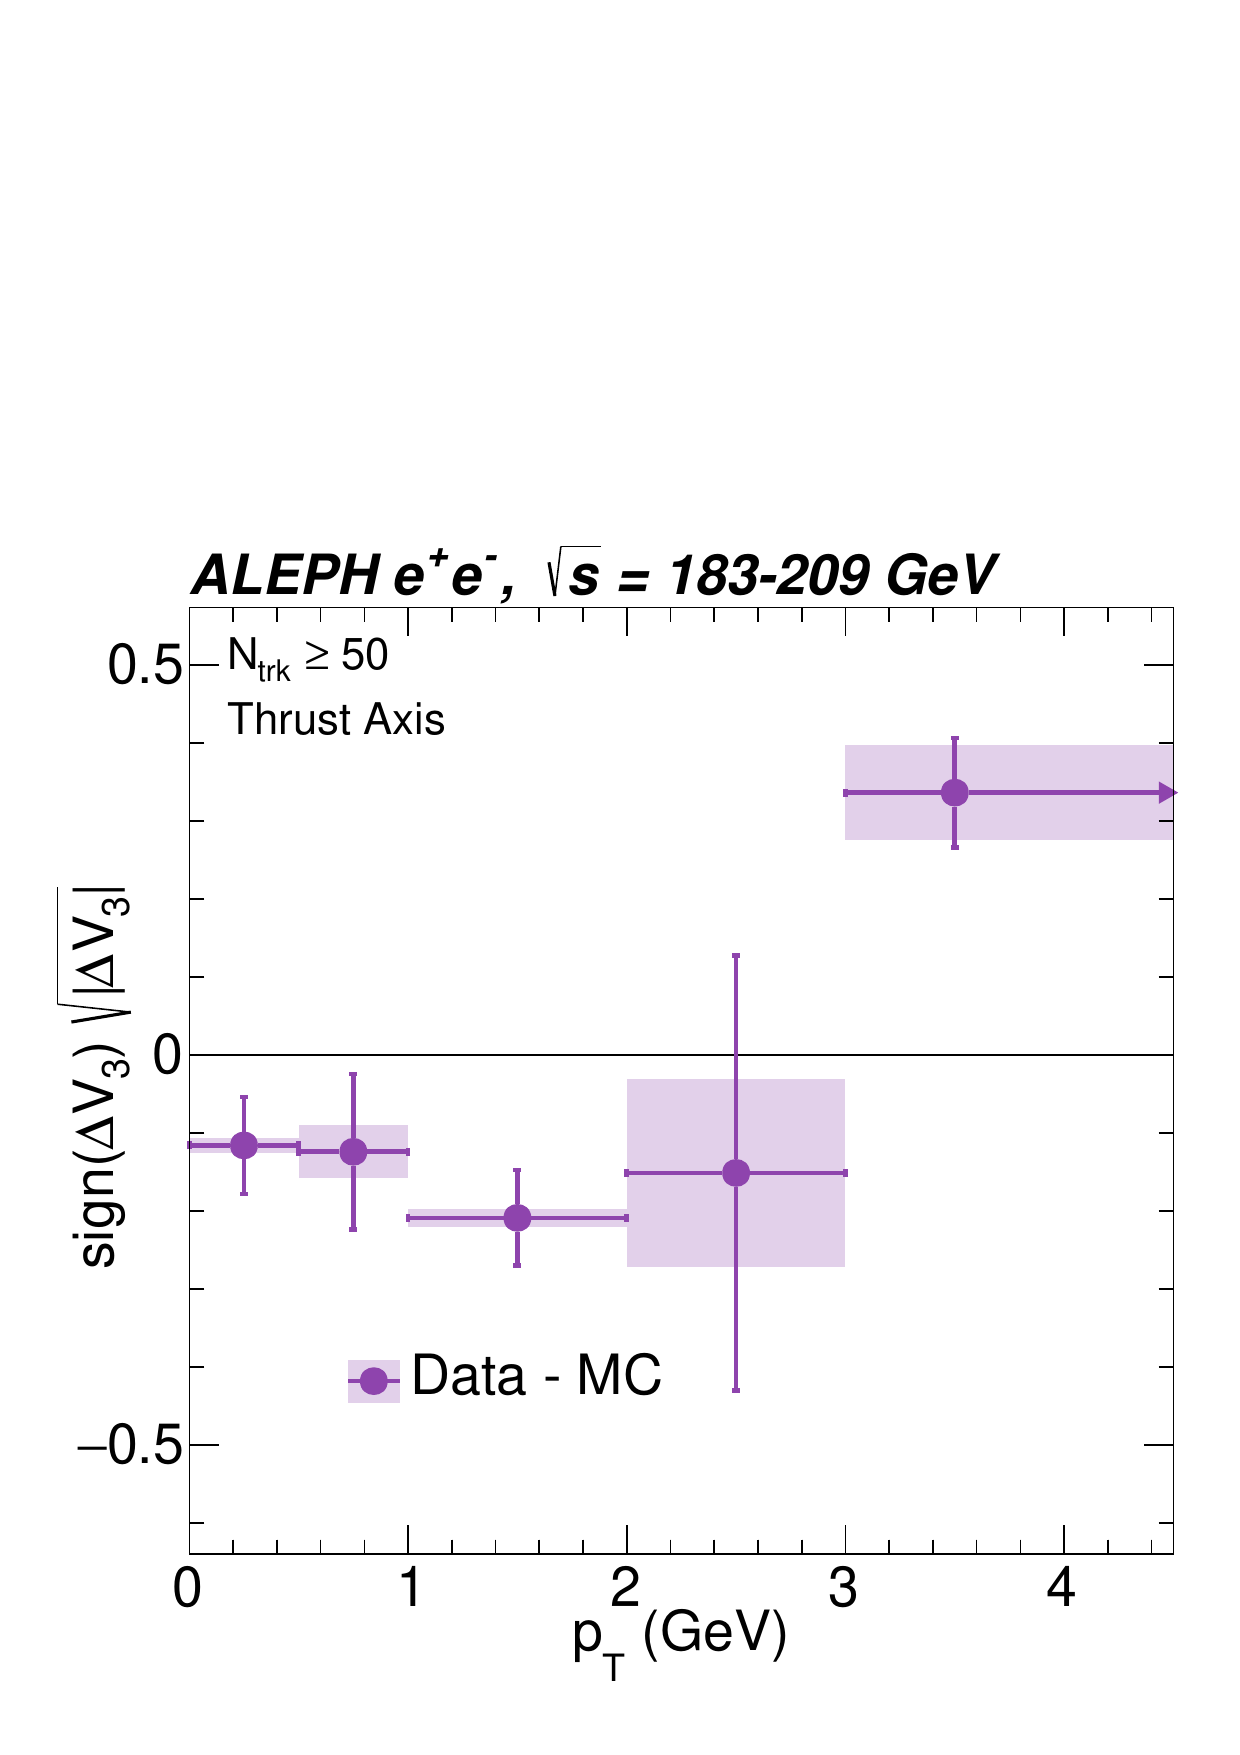}
    \caption{${\rm N}_{\rm trk} \ge 50$}
        %\label{fig:}
    \end{subfigure}
\caption{$\Delta v_{3}$ as a function of the track pairs' $p_{T}$ requirement in different  multiplicity intervals for the thrust axis analysis for LEP-II high-energy sample.}
\label{fig:Dv3VsPt_thrust}
\end{figure}

\clearpage

\section{Physics processes above $W^{+}W^{-}$ production threshold}

For high-energy events above the $W$-pair production threshold,  four-fermion processes mediated by the double- or single- $W$ or $Z$ boson are the sub-dominant contributions. 
The topology of four-fermion processes differs largely from that of the $e^+e^- \to q\bar{q}$; more importantly, there can be non-trivial final-state interconnection (FSI) effects such as Color Reconnection (CR) and Bose-Einstein Correlation (BEC) in hadronic decays of boson pairs. 
These physics processes might accommodate promising potentials for the ridge-signal search, which is beyond our current understanding of the $e^+e^-$ collision system. A recent theoretical work~\cite{Larkoski:2021hee} calculating by assuming the large-$N$ limit also makes remarks that for processes beyond the leading order $e^+e^- \to q\bar{q}$  events via $Z$ decays, there is no suppression for generating such collectivity correlations.
We further categorize the high-energy sample into {\it $qq$-like events} and {\it $WW$-like events}. 
Two quantities are computed by clustering the final-state particles into four jets,
\begin{equation}
\begin{aligned}
d^2 &= min[\frac{(m_{ij}-M_W)^2+(m_{kl}-M_W)^2}{M_W^2}] \quad (M_W=80.4~\text{GeV, with $i,j,k,l$ being jet indices})\\
c_W &= \cos(\text{smallest interjet angle})
\end{aligned}
\end{equation}
Events with $d^2 \ge 0.1$ or $c_W \ge 0.9$ are treated as the hadronic-$q\bar{q}$-dominant sample, otherwise the four-fermion-process-enhanced sample.

\txcb{[Need to update to Bayesian results]}
\begin{figure}[ht]
\centering
\makebox[\textwidth][c]{
    \includegraphics[width=1.2\textwidth]{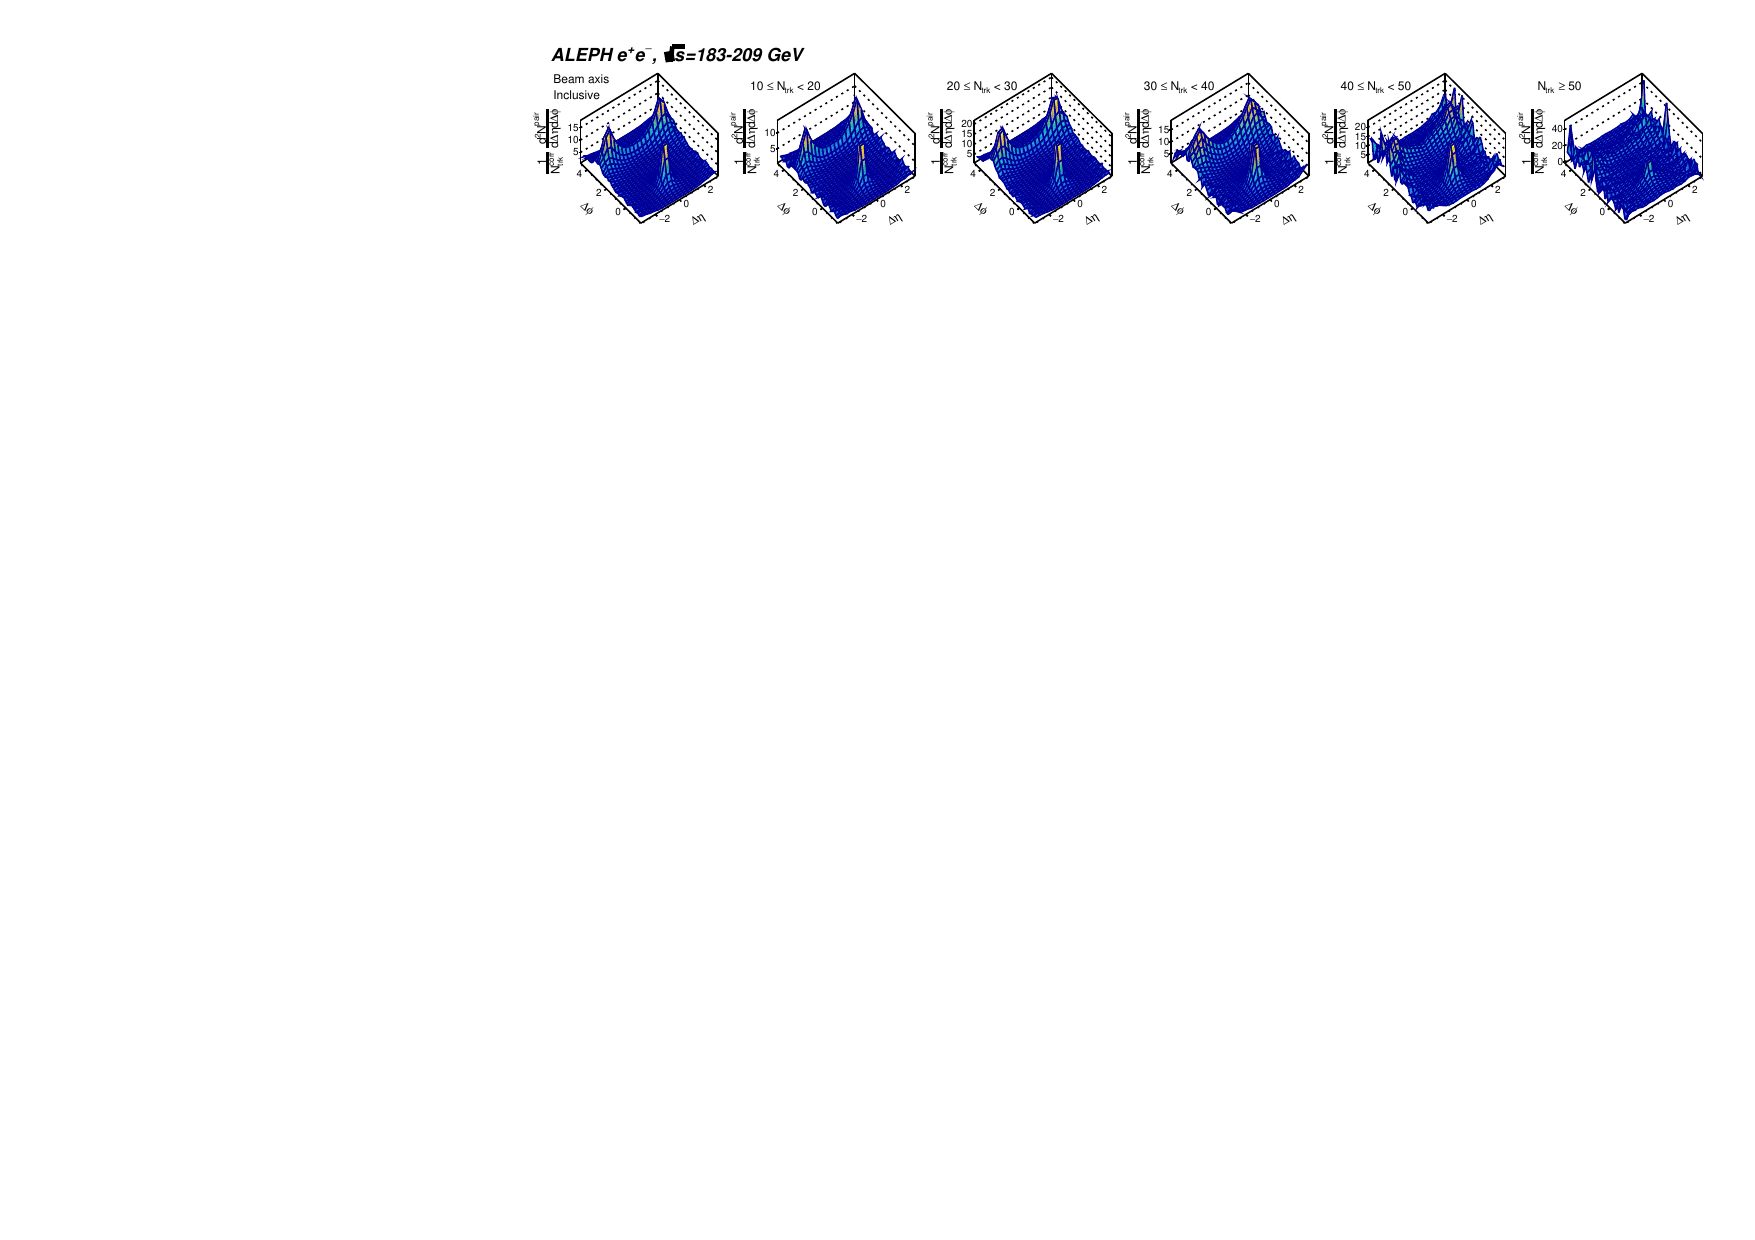}
}
\caption{Two-particle correlation function for $q\bar{q}$-like high-energy sample in the beam axis analysis. Results are shown multiplicity-inclusively and as a function of the offline multiplicity in $[10,20), [20,30), [30,40), [40,50), [50, \infty)$ intervals.}
\label{fig:EnergyCut_ge_100_TopoCut_qqLike_beam}
\end{figure}

\begin{figure}[ht]
\centering
\makebox[\textwidth][c]{
    \includegraphics[width=1.2\textwidth]{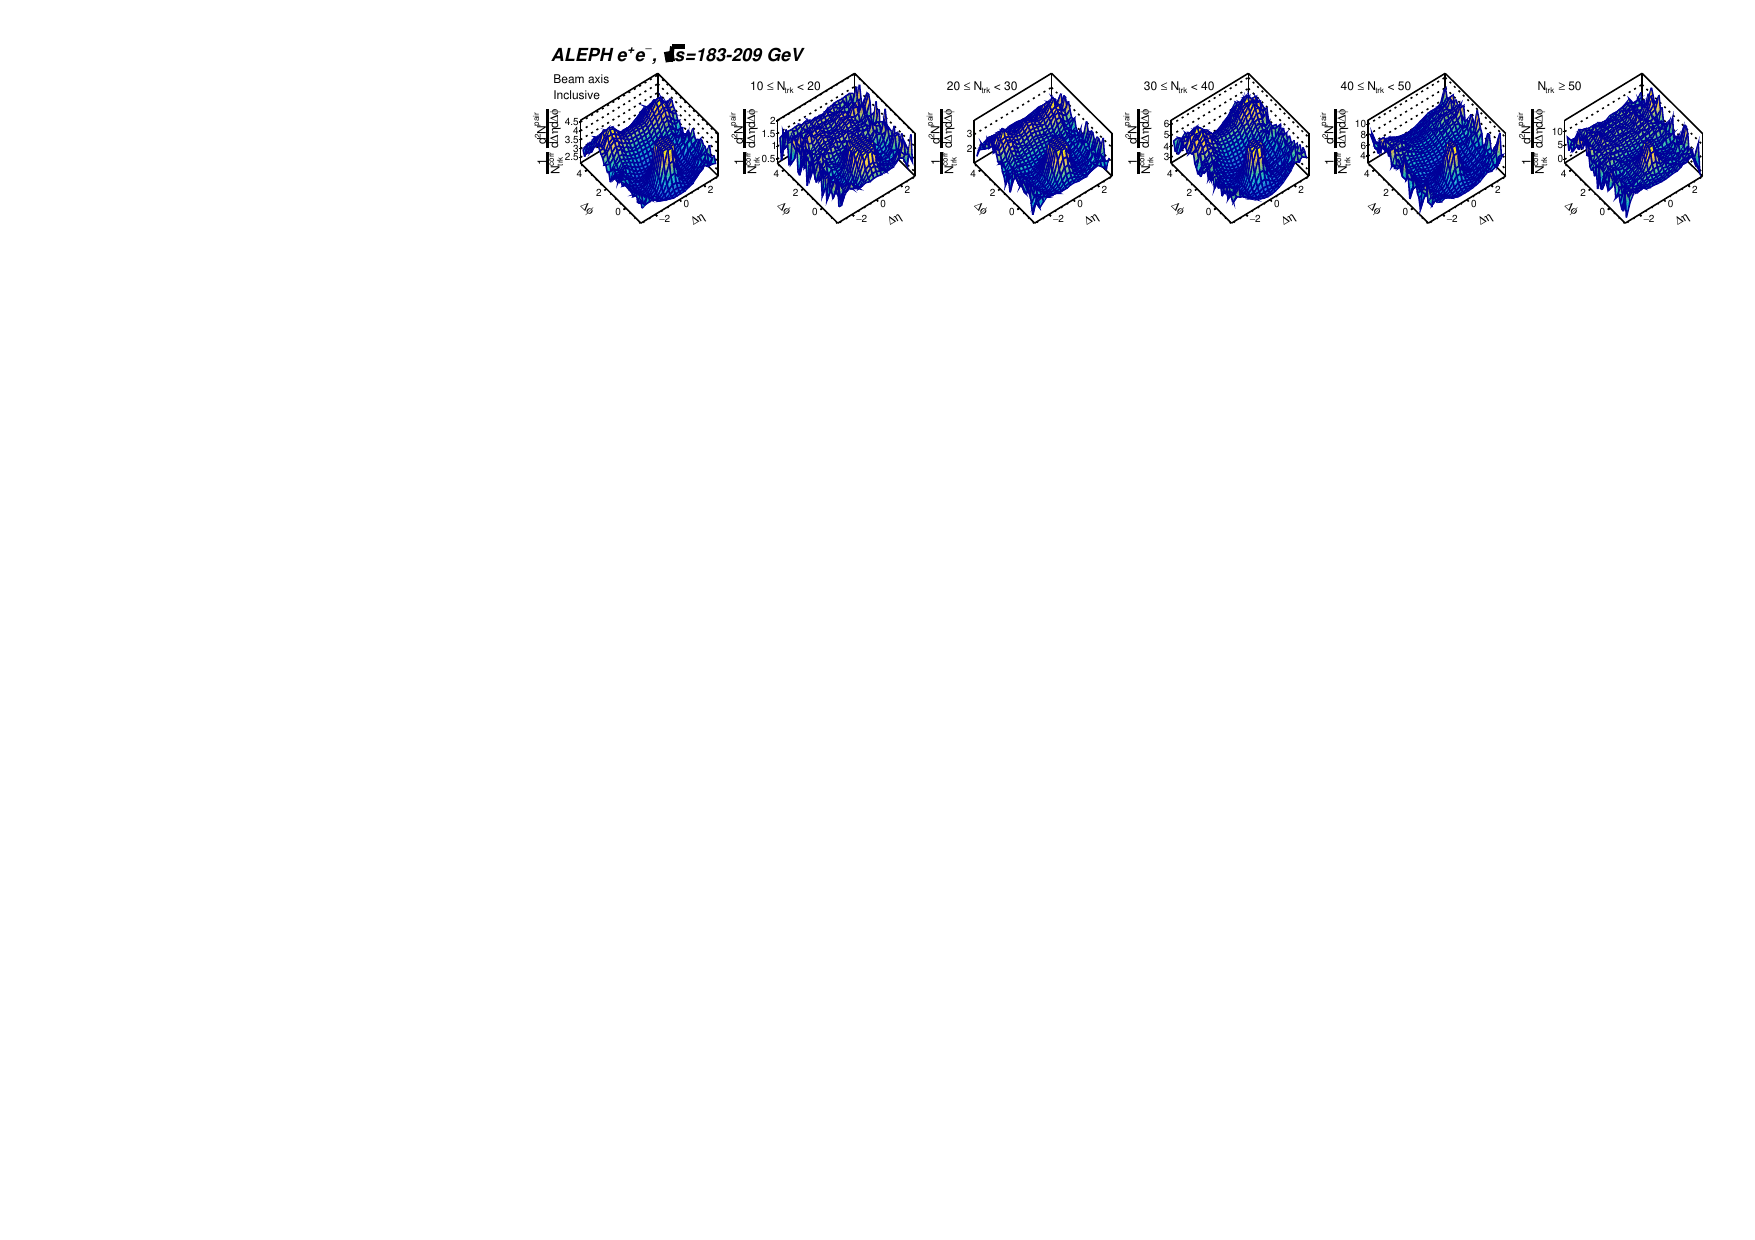}
}
\caption{Two-particle correlation function for $WW$-like high-energy sample in the beam axis analysis. Results are shown multiplicity-inclusively and as a function of the offline multiplicity in $[10,20), [20,30), [30,40), [40,50), [50, \infty)$ intervals.}
\label{fig:EnergyCut_ge_100_TopoCut_WWLike_beam}
\end{figure}

\begin{figure}[ht]
\centering
\makebox[\textwidth][c]{
    \includegraphics[width=1.2\textwidth]{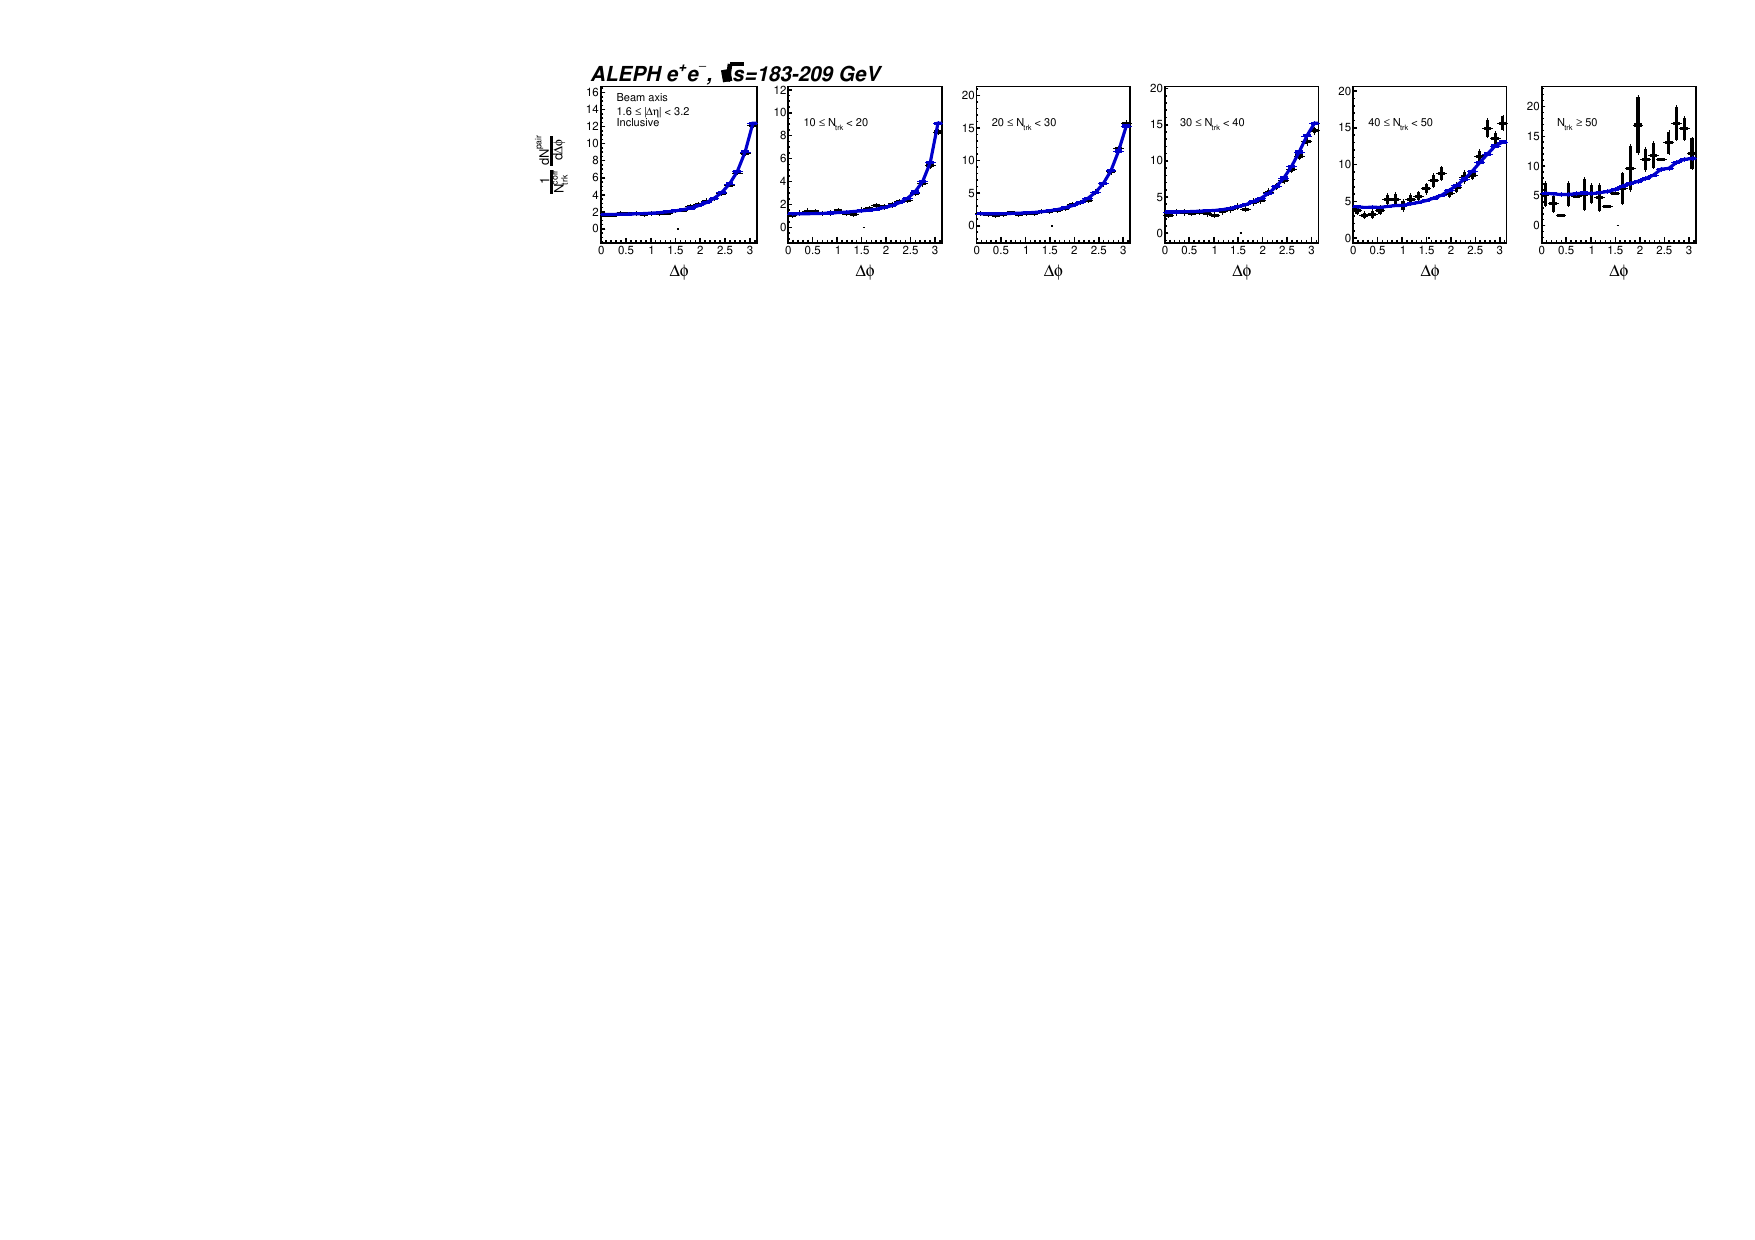}
}
\caption{Long-range azimuthal differential yields for $q\bar{q}$-like high-energy sample in the beam axis analysis. Results are shown multiplicity-inclusively and as a function of the offline multiplicity in $[10,20), [20,30), [30,40), [40,50), [50, \infty)$ intervals.}
\label{fig:EnergyCut_ge_100_TopoCut_qqLike_beam_1d}
\end{figure}

\begin{figure}[ht]
\centering
\makebox[\textwidth][c]{
    \includegraphics[width=1.2\textwidth]{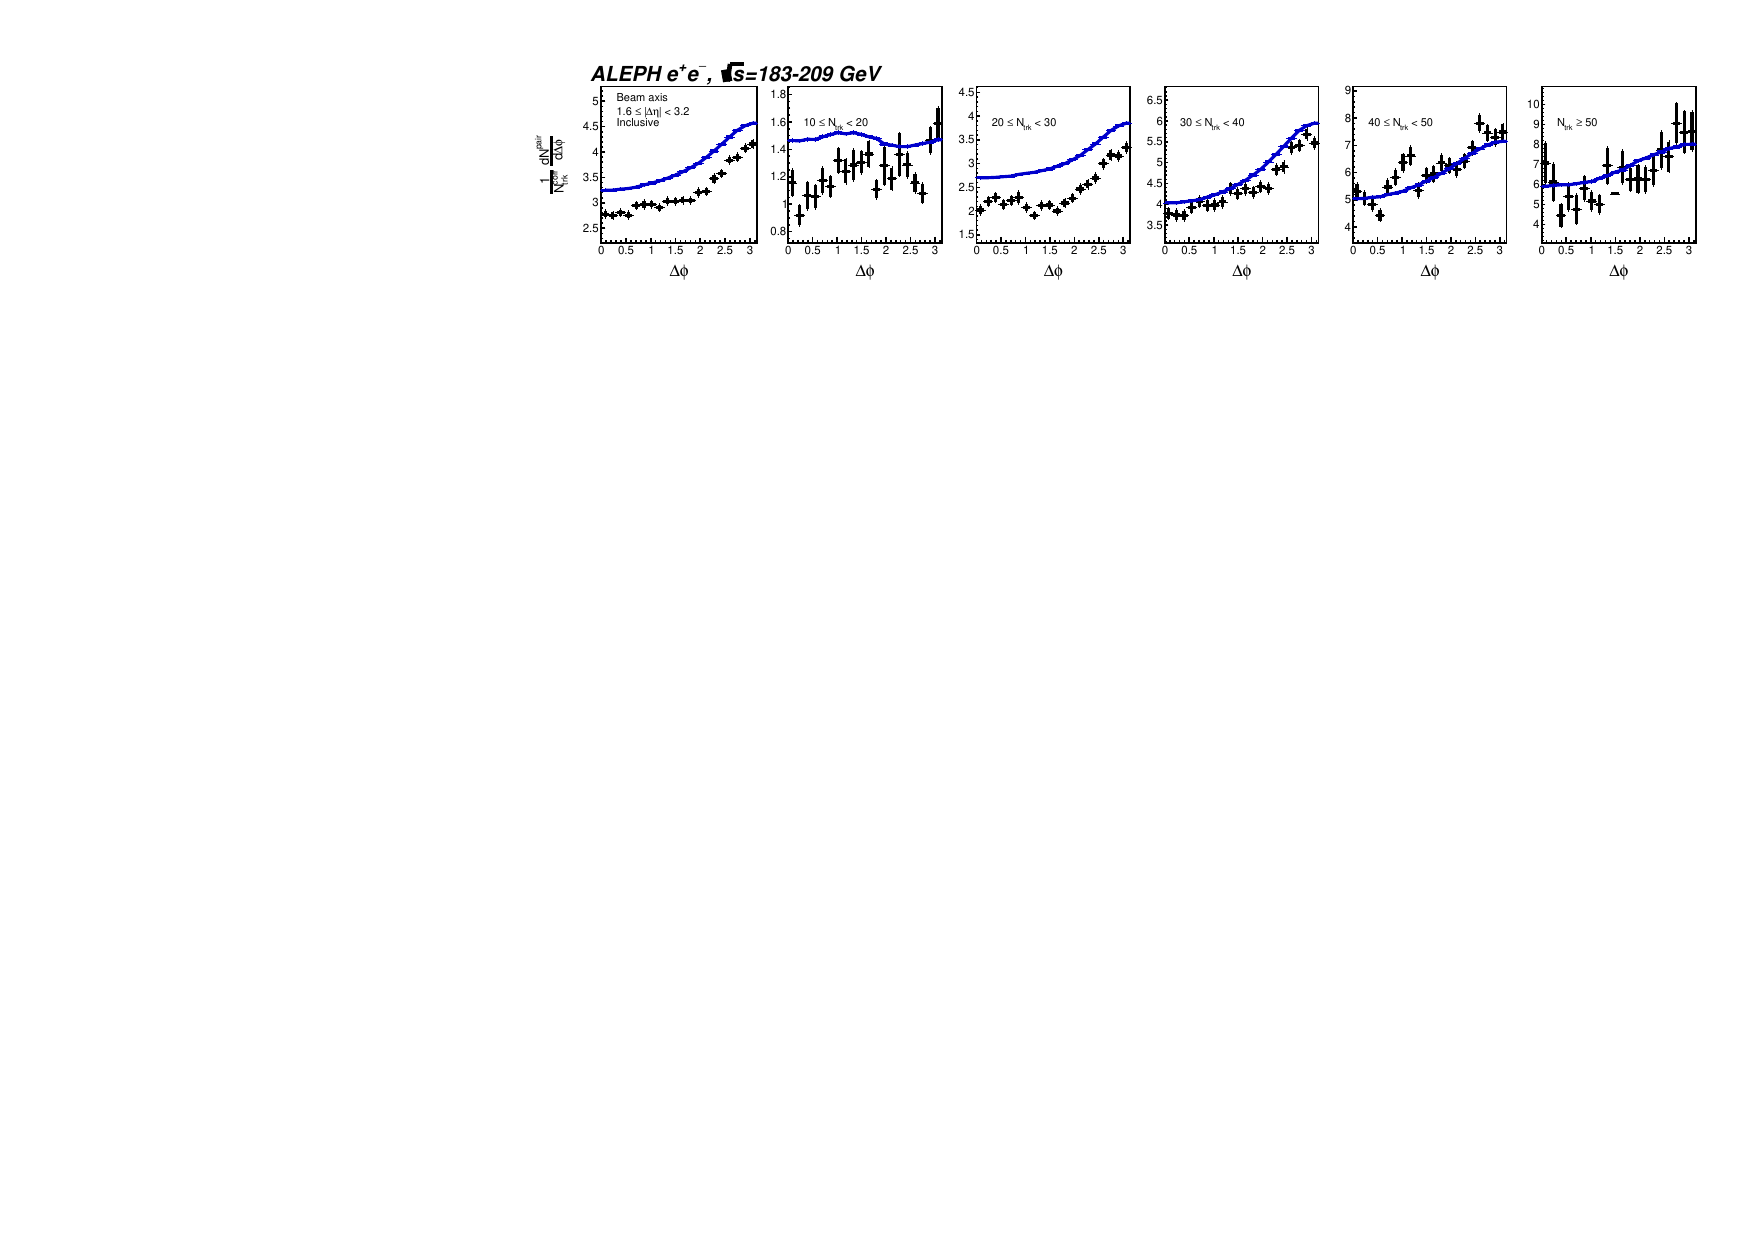}
}
\caption{Long-range azimuthal differential yields for $WW$-like high-energy sample in the beam axis analysis. Results are shown multiplicity-inclusively and as a function of the offline multiplicity in $[10,20), [20,30), [30,40), [40,50), [50, \infty)$ intervals.}
\label{fig:EnergyCut_ge_100_TopoCut_WWLike_beam_1d}
\end{figure}

\begin{figure}[ht]
\centering
\makebox[\textwidth][c]{
    \includegraphics[width=1.2\textwidth]{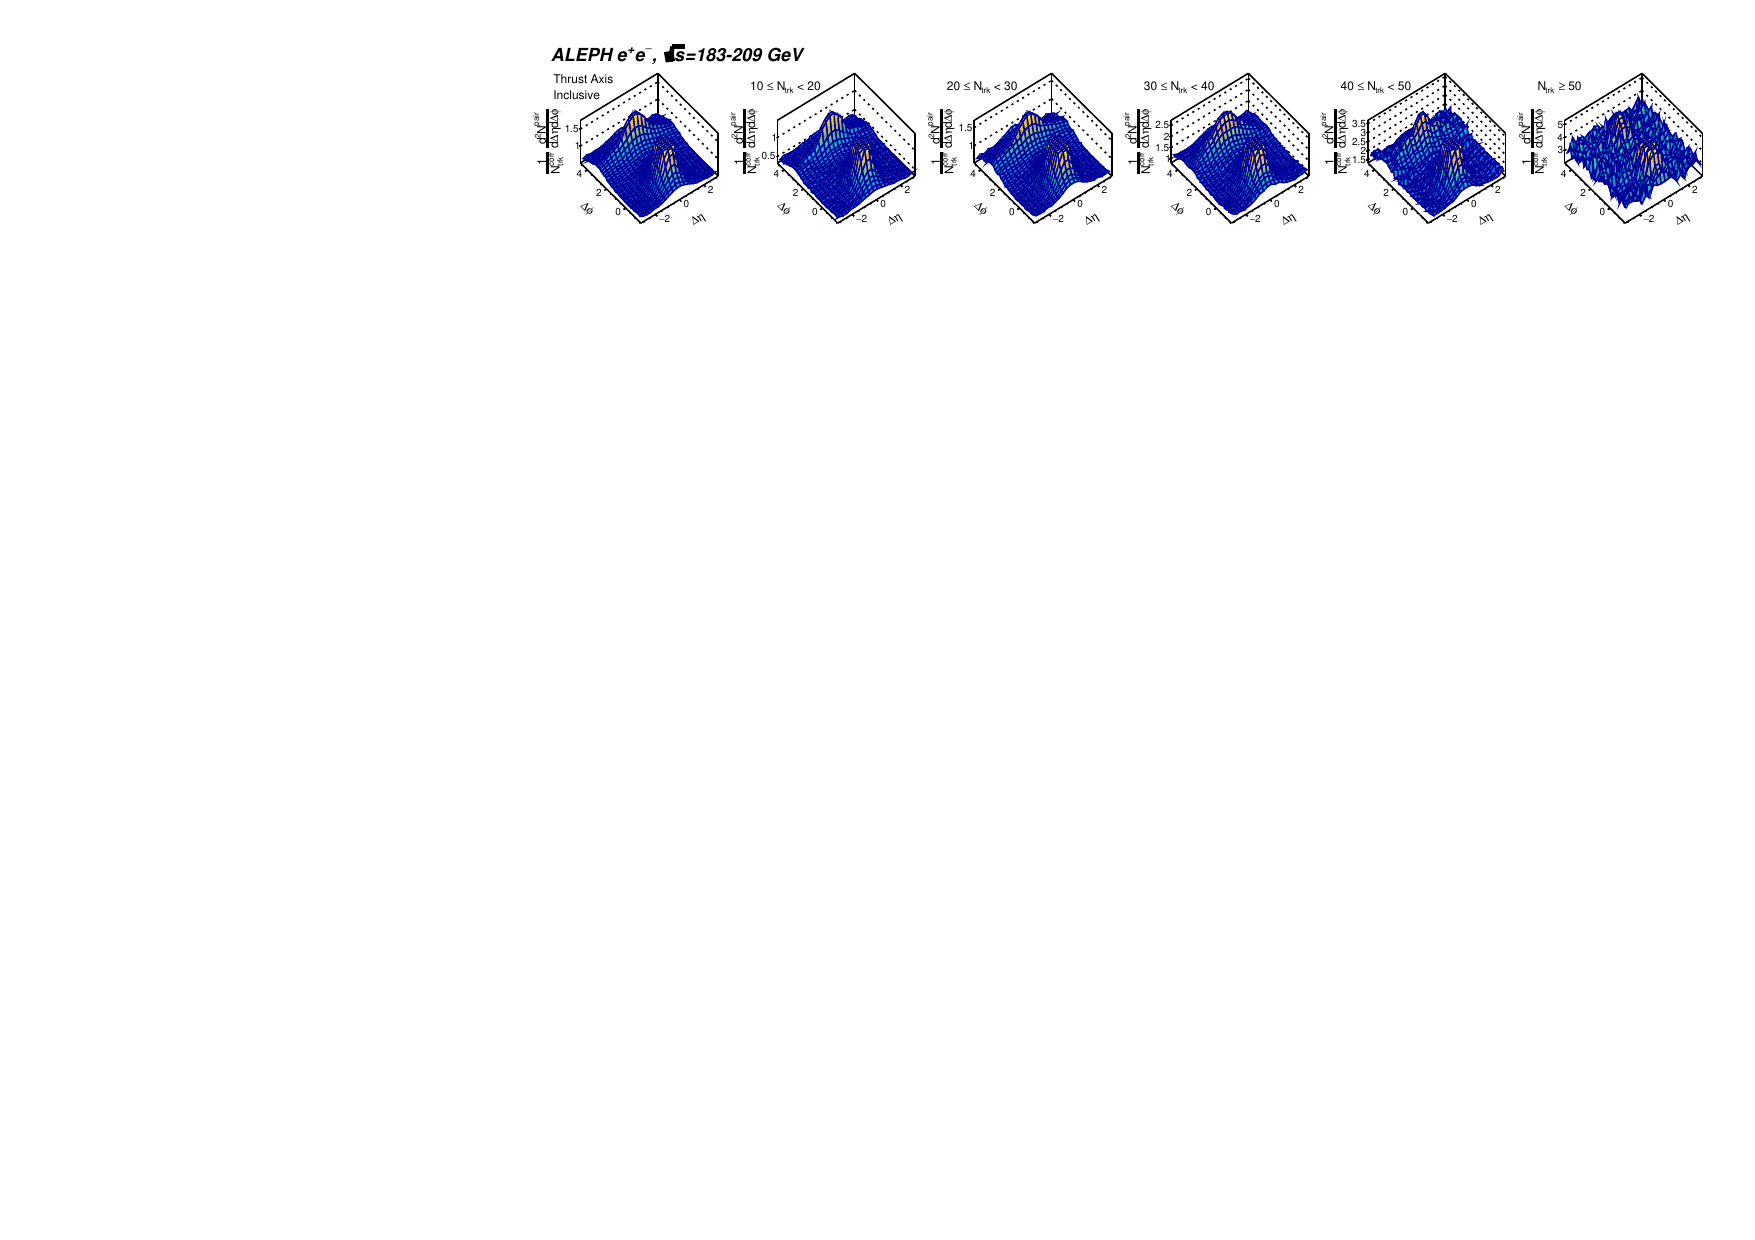}
}
\caption{Two-particle correlation function for $q\bar{q}$-like high-energy sample in the thrust axis analysis. Results are shown multiplicity-inclusively and as a function of the offline multiplicity in $[10,20), [20,30), [30,40), [40,50), [50, \infty)$ intervals.}
\label{fig:EnergyCut_ge_100_TopoCut_qqLike_thrust}
\end{figure}

\begin{figure}[ht]
\centering
\makebox[\textwidth][c]{
    \includegraphics[width=1.2\textwidth]{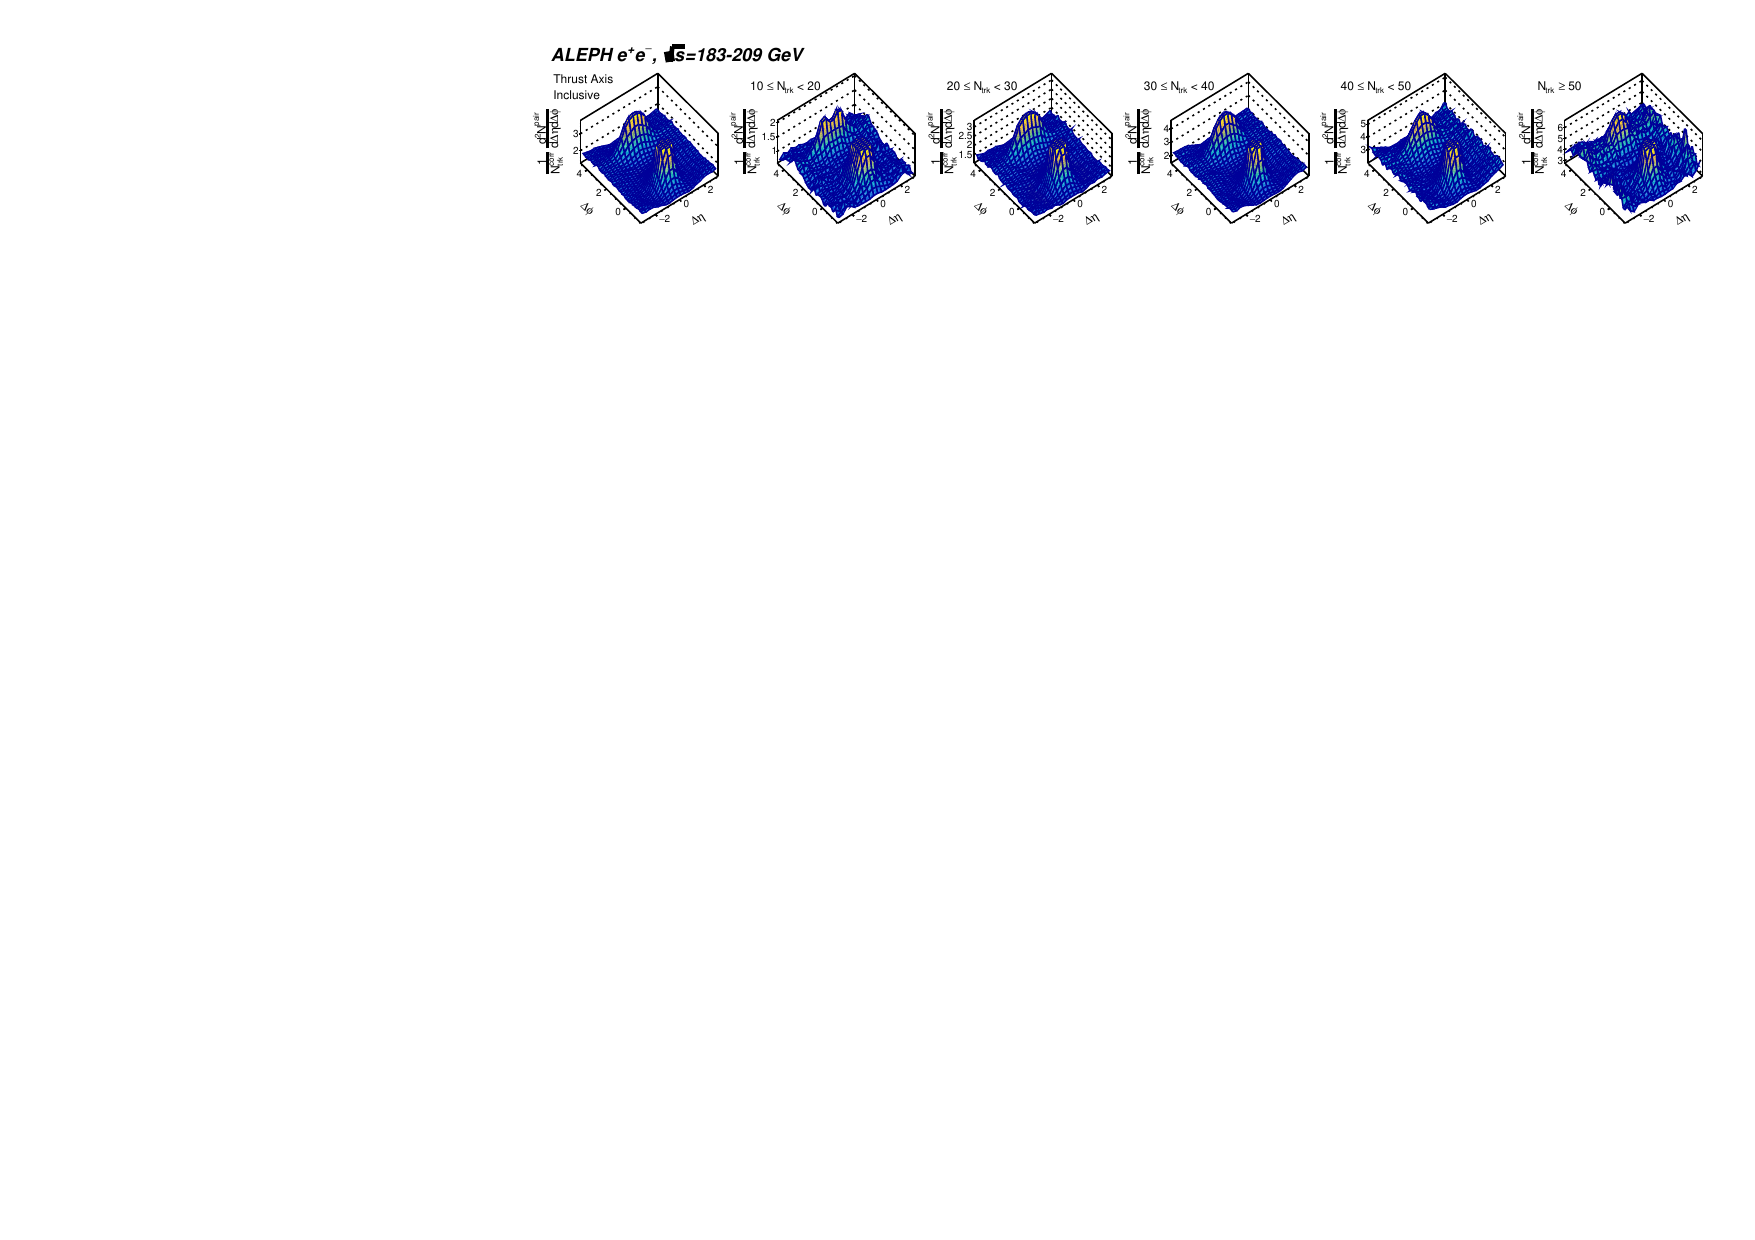}
}
\caption{Two-particle correlation function for $WW$-like high-energy sample in the thrust axis analysis. Results are shown multiplicity-inclusively and as a function of the offline multiplicity in $[10,20), [20,30), [30,40), [40,50), [50, \infty)$ intervals.}
\label{fig:EnergyCut_ge_100_TopoCut_WWLike_thrust}
\end{figure}

\begin{figure}[ht]
\centering
\makebox[\textwidth][c]{
    \includegraphics[width=1.2\textwidth]{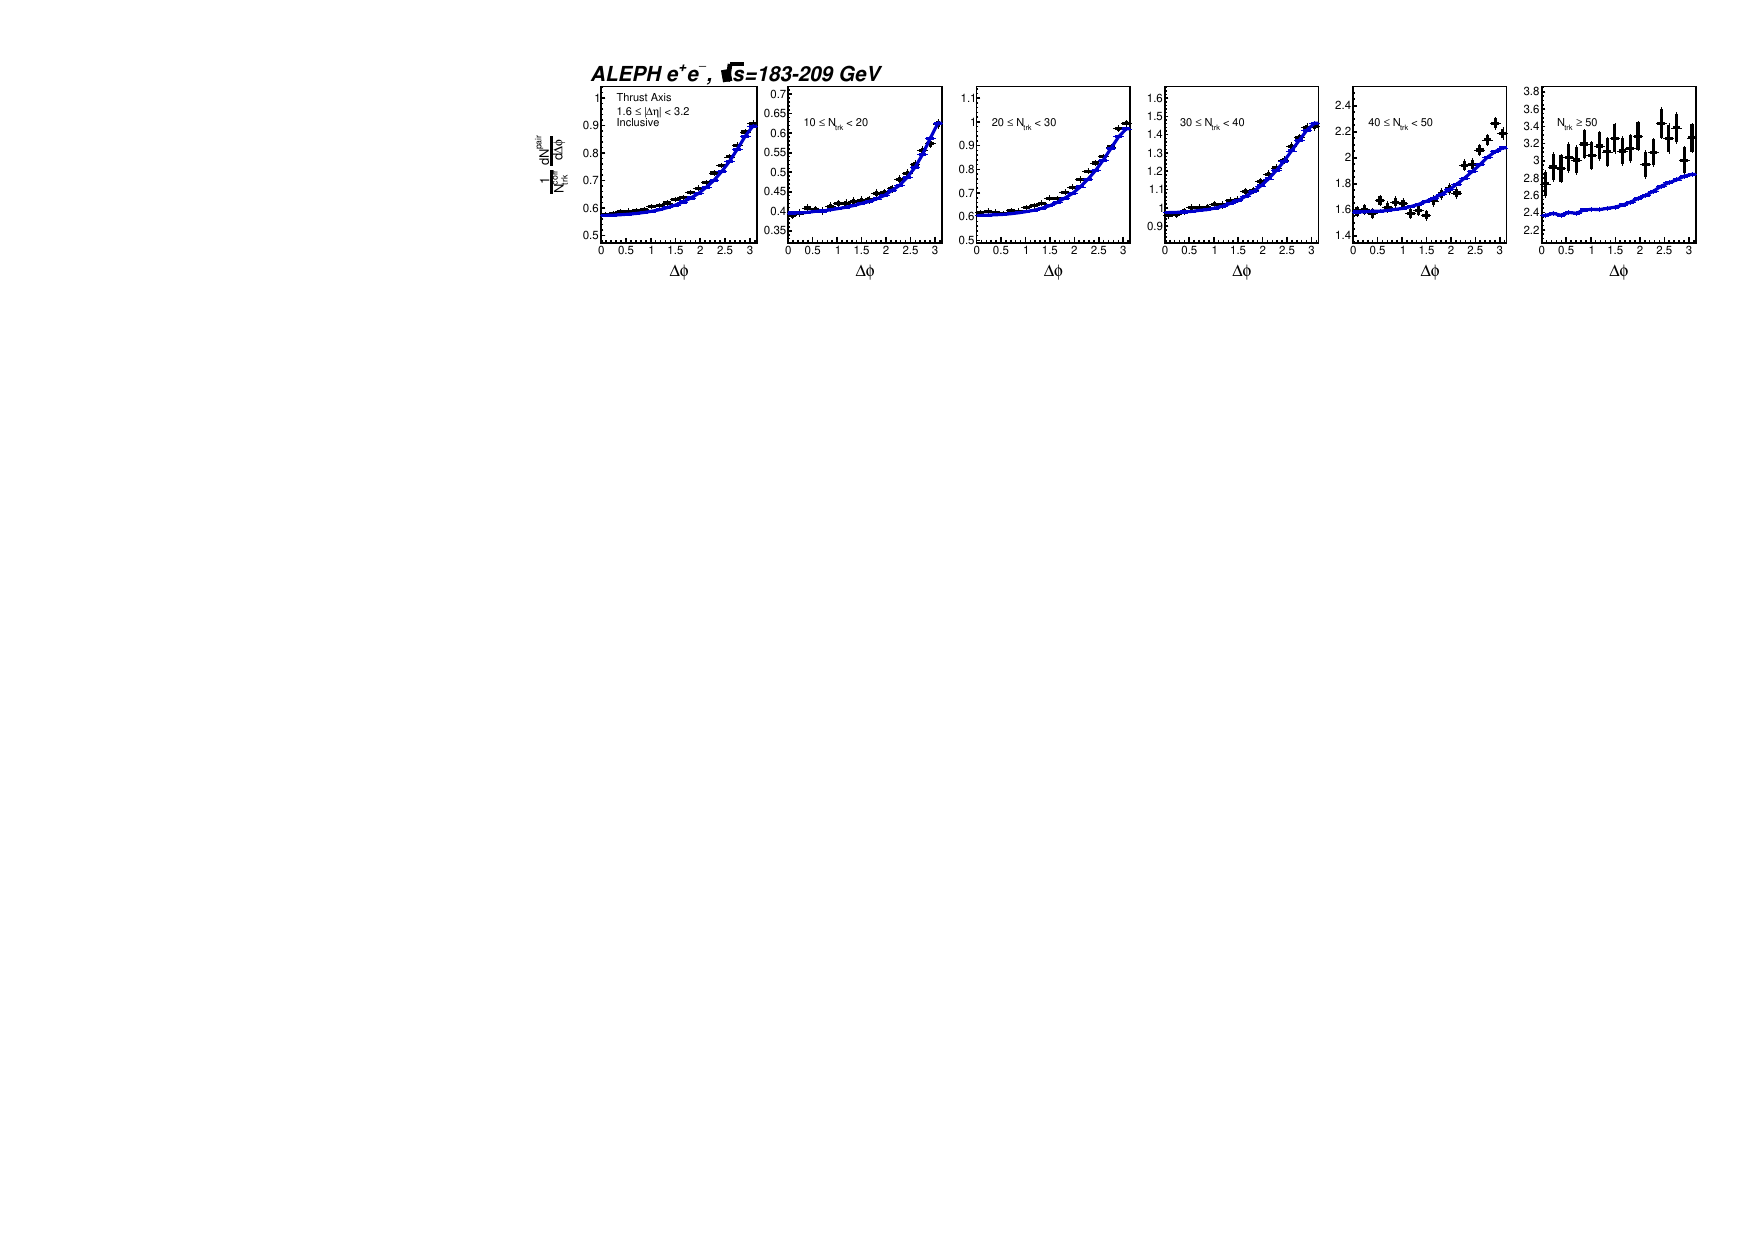}
}

\caption{Long-range azimuthal differential yields for $q\bar{q}$-like high-energy sample in the thrust axis analysis. Results are shown multiplicity-inclusively and as a function of the offline multiplicity in $[10,20), [20,30), [30,40), [40,50), [50, \infty)$ intervals.}
\label{fig:EnergyCut_ge_100_TopoCut_qqLike_thrust_1d}
\end{figure}

\begin{figure}[ht]
\centering
\makebox[\textwidth][c]{
    \includegraphics[width=1.2\textwidth]{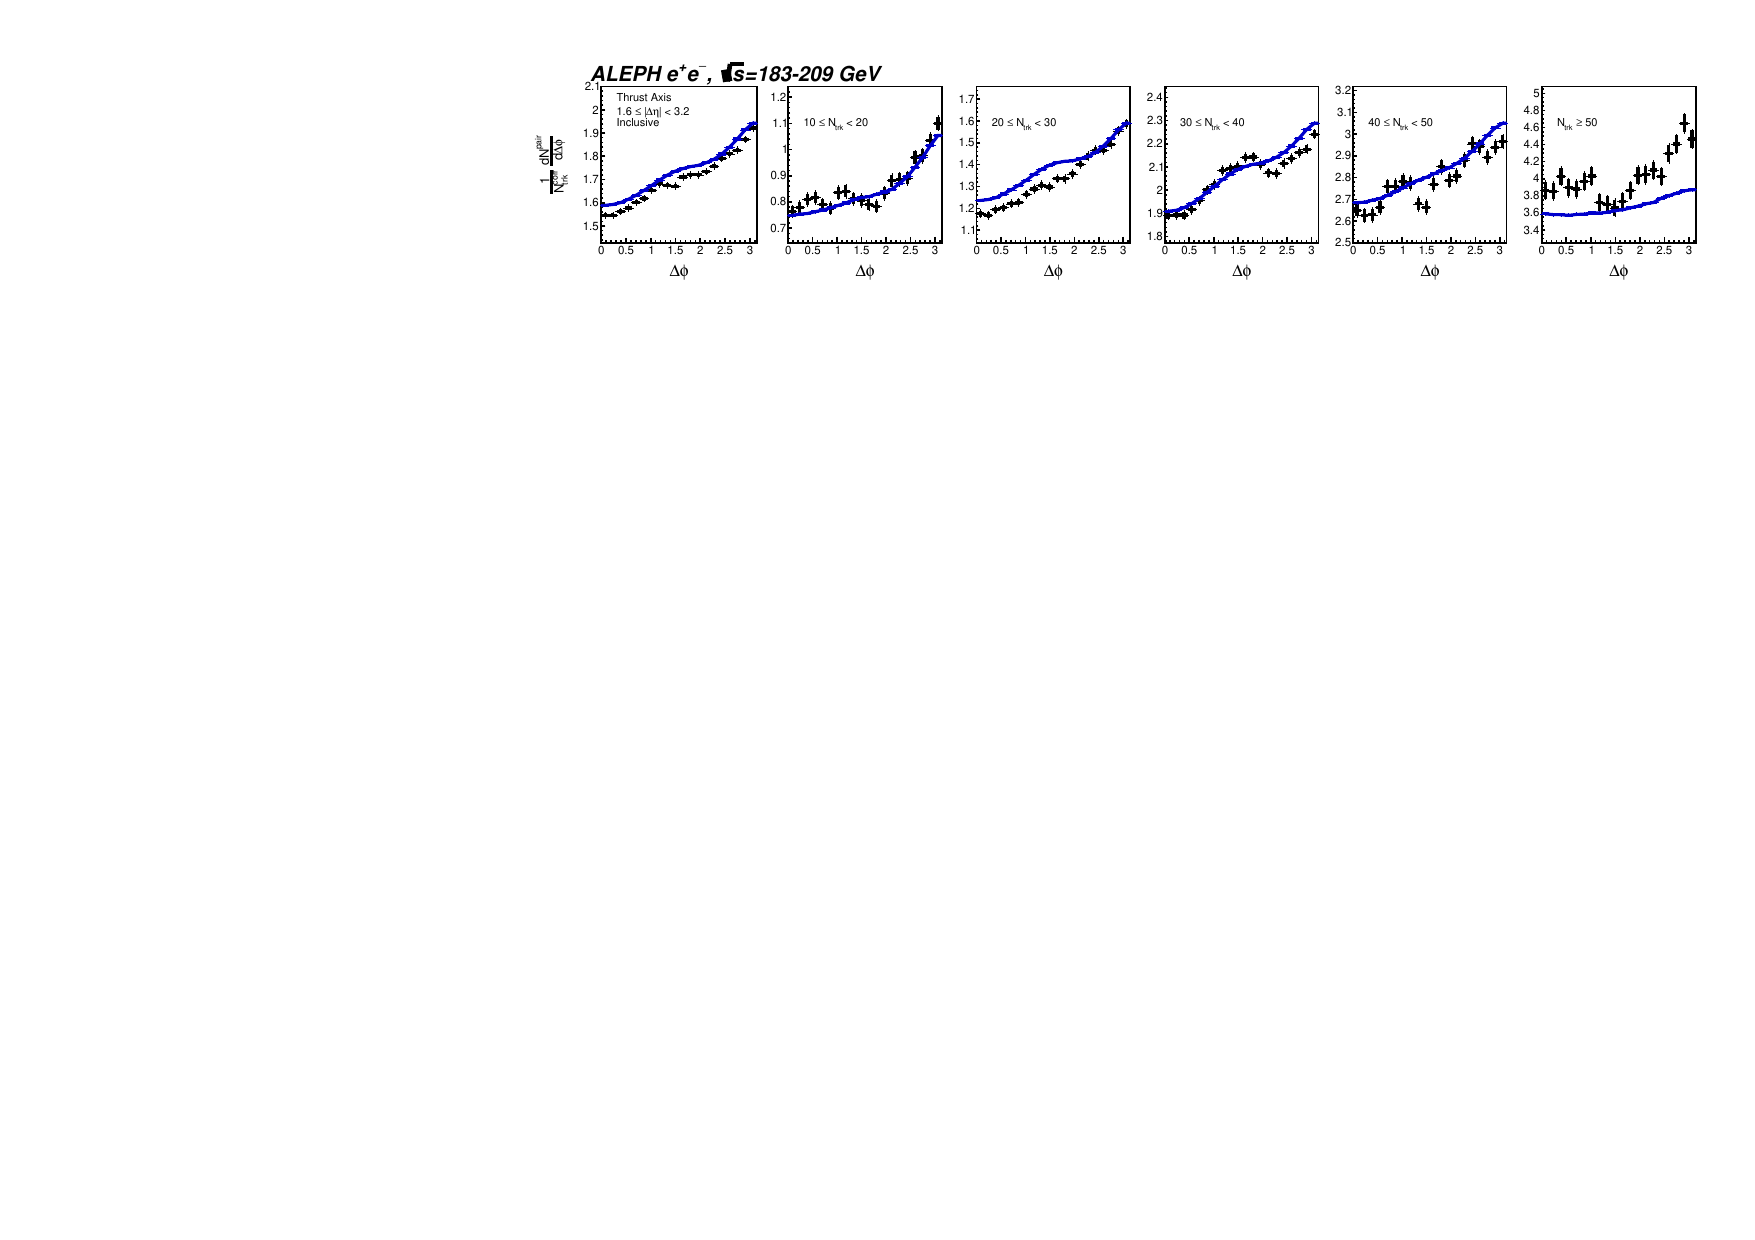}
}
\caption{Long-range azimuthal differential yields for $WW$-like high-energy sample in the thrust axis analysis. Results are shown multiplicity-inclusively and as a function of the offline multiplicity in $[10,20), [20,30), [30,40), [40,50), [50, \infty)$ intervals.}
\label{fig:EnergyCut_ge_100_TopoCut_WWLike_thrust_1d}
\end{figure}
